# Supplementary material for: WPDA: Frequency-based Backdoor Attack with Wavelet Packet Decomposition
Source: arXiv:2401.13578 source file (2024-12-01)
Supplement: Supplementary file 1 [file 7_appendix.tex]

\onecolumn
\newpage
\appendix
\section{Appendix}
\label{appendix}
\subsection{\textbf{Derivation and verification}: Using the absolute average algorithm could potentially reduce sensitivity to noise compared to using the average absolute algorithm.
\label{explain why it is important to take the average value before taking the absolute value}
}
% Here's a detailed explanation of
% Reducing Sensitivity to Noise: Absolute Mean vs. Mean of Absolute Values
Here's a detailed explanation of why using the absolute average could potentially reduce sensitivity to noise compared to using the average absolute:\\
1. Understanding Noise and Its Impact:\\
In image processing and signal analysis, noise refers to unwanted variations or disturbances that corrupt the original signal. Noise can arise from various sources, such as sensor limitations, transmission errors, or environmental factors. When applying wavelet packet decomposition to an image, noise can manifest as small fluctuations in the coefficient values within each sub-spectrogram. These fluctuations might not necessarily represent meaningful information but rather random disturbances.The design of effectiveness metric $E$ influences how sensitive the selection of key frequency regions is to these noise-induced fluctuations.\\
2. Absolute average algorithm \textit{vs} Average absolute algorithm and Noise Reduction:\\
Before calculating the absolute values, computing the average of the coefficient matrix can reduce the impact of noise-induced fluctuations on the overall average. For example, considering a sub-spectrogram with a coefficient matrix like [-3, +4, -2, +5], the absolute average value of the coefficient matrix is +1. However, if noise causes small fluctuations, the coefficient matrix might become [-3.1, +3.9, -1.9, +4.2]. The average value of the coefficient matrix now changes to 1.025, even though the overall information content has not significantly changed.
Using the average absolute algorithm, the average absolute value of the coefficient matrix is +3.5, while the average absolute value of the coefficient matrix with noise is +3.275, demonstrating a higher sensitivity to the noise-induced fluctuations.\\
3. Verification Experiment:\\
Using the average absolute algorithm, the key frequency regions are `ah', `hh', `vv', `dd'. We conduct empirical experiments to complete the training and generate backdoor samples in the same way as WPDA. Take CIFAR-10 as an example, Fig.~\ref{abs mean} demonstrates that poisoned samples generated by the average absolute algorithm are less effective than those produced by absolute average algorithm. \\
\begin{figure}[H]
\centering  %图片全局居中
    {
    \includegraphics[width=1.65in]{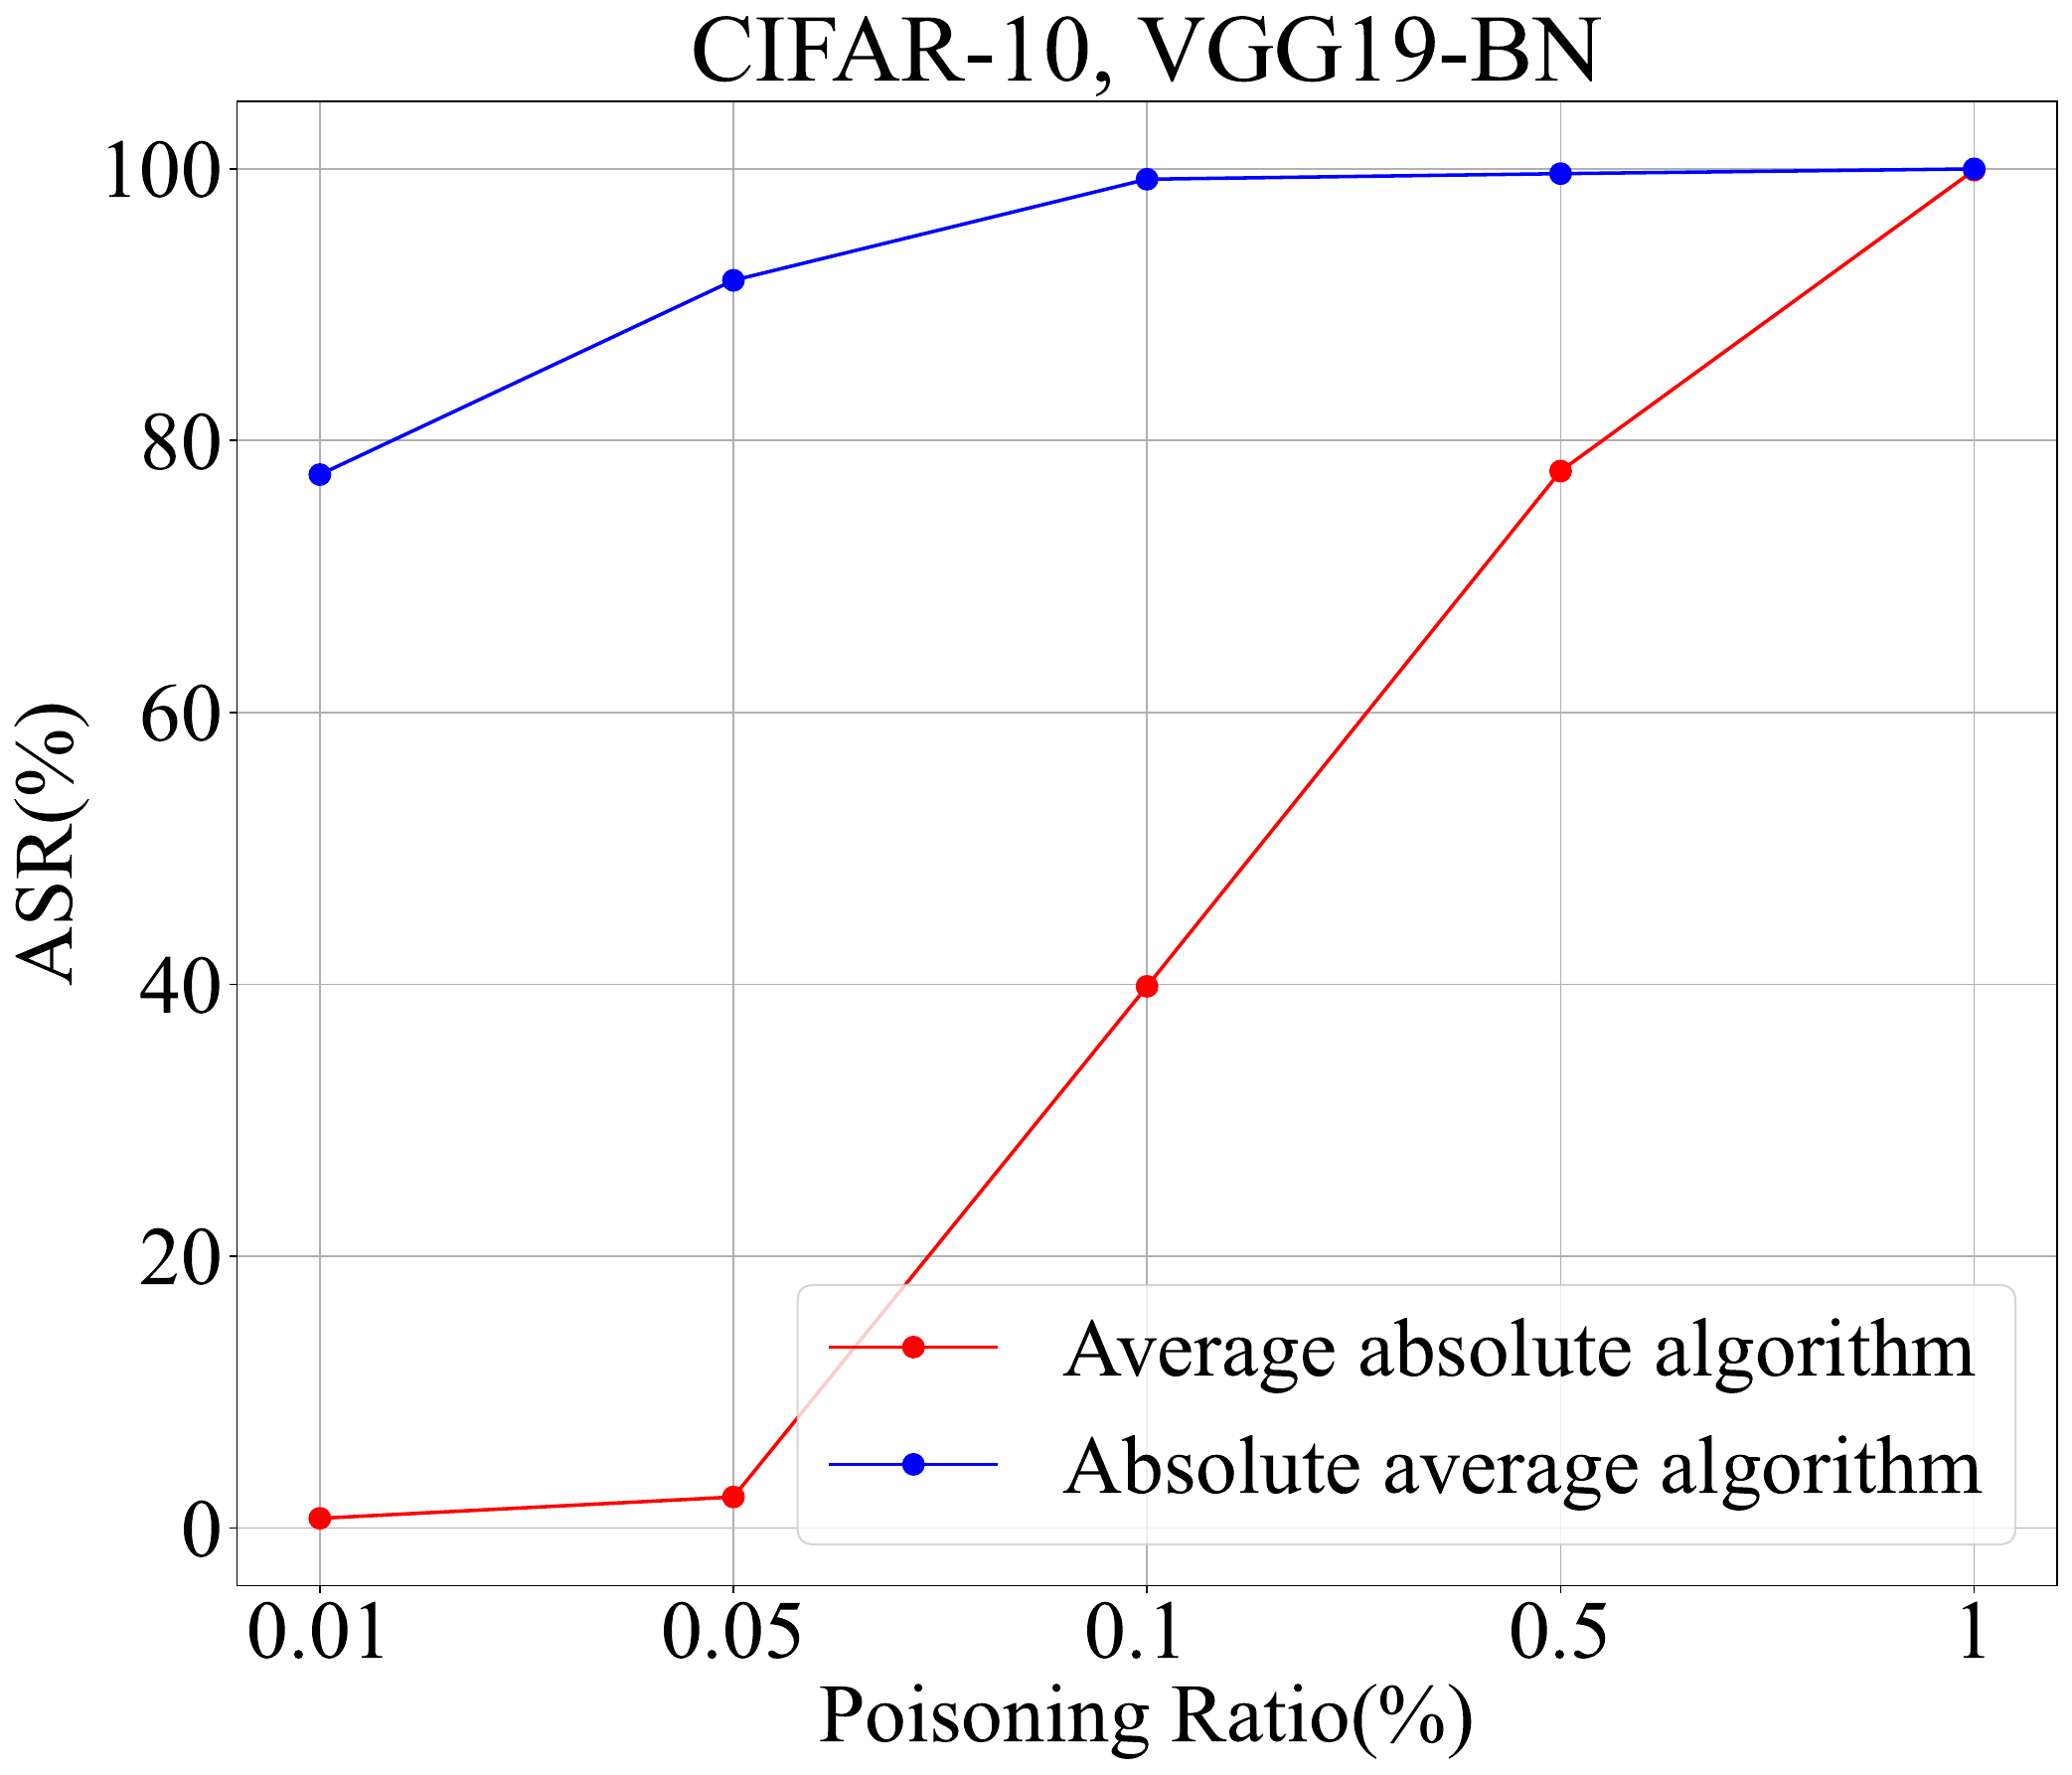}}
    \label{vgg19bn_abs_mean}
    {
    \includegraphics[width=1.65in]{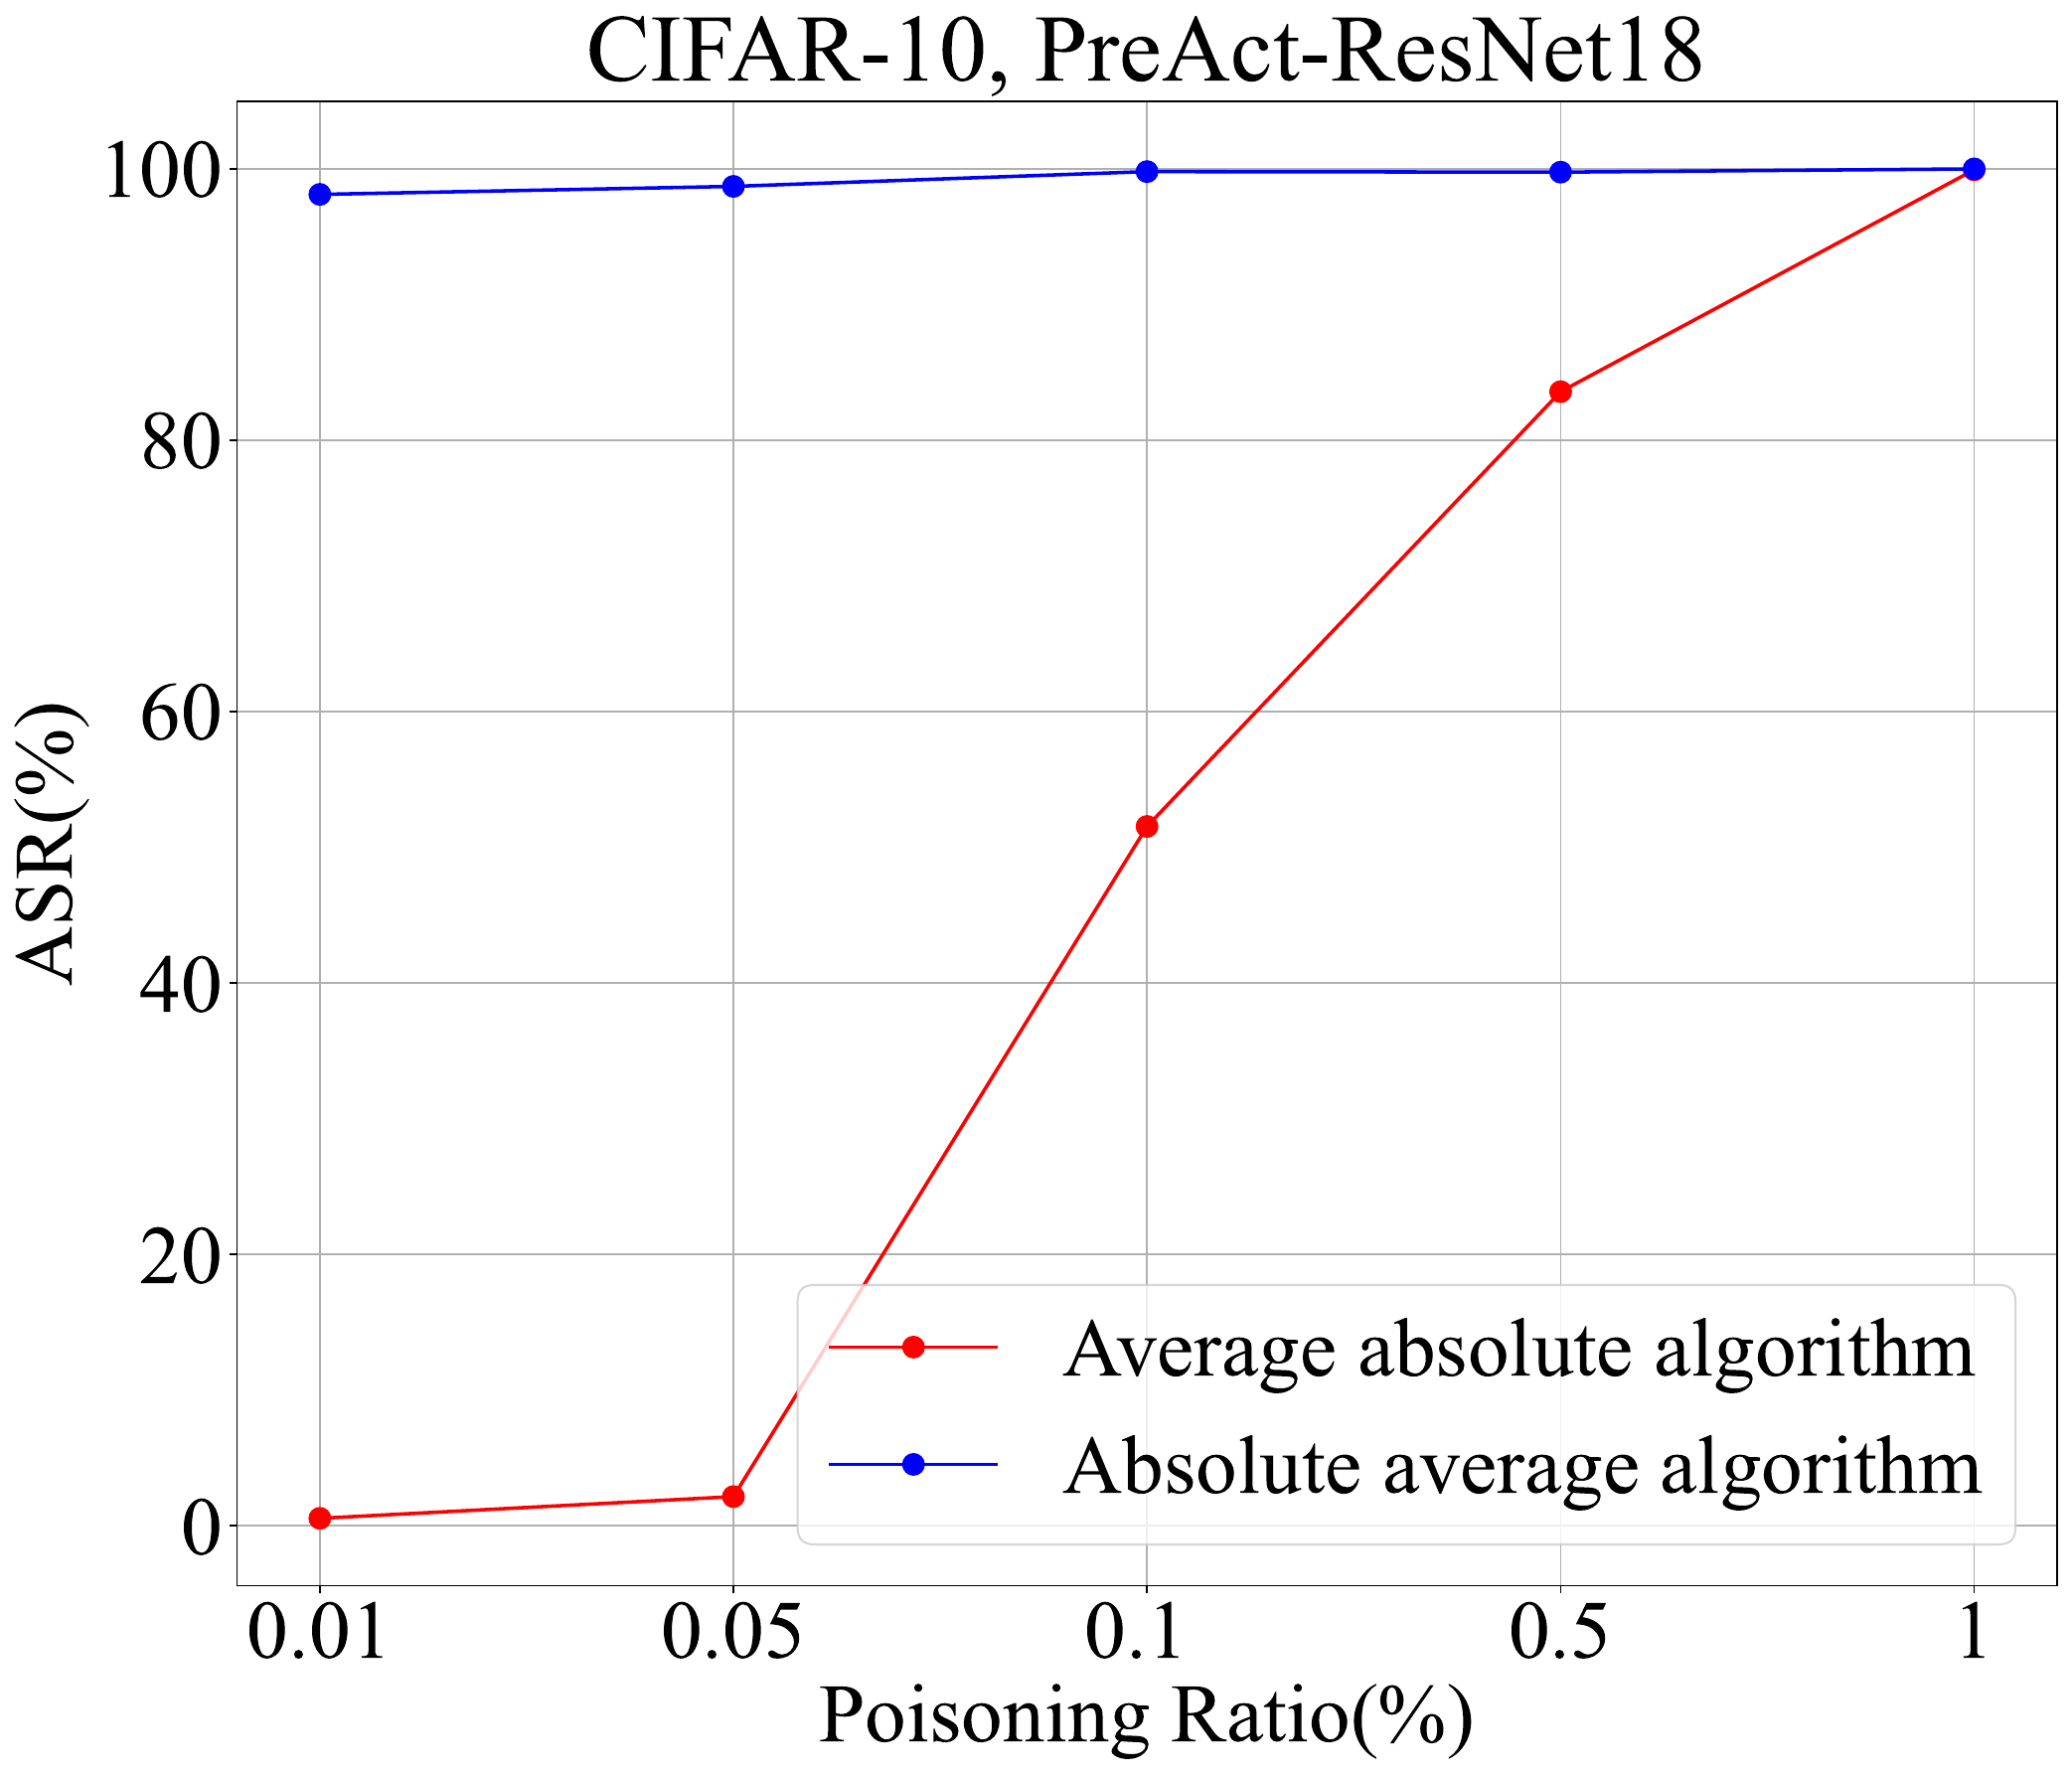}}
    \label{preactresnet18_abs_mean}
\caption{Effect of original information in key frequency regions on model learning triggers.}
\label{abs mean}
\end{figure}
\noindent4. Combining Evidence and Reasoning:\\
By combining theoretical reasoning and empirical evidence, we can infer that absolute average algorithm can effectively reduce the effect of noise on the samples and help us accurately select key frequency regions.

\subsection{\textbf{Derivation and verification}:
\label{original information have negative effect on the backdoor activation}
The original sample information compete with the trigger information for the model’s attention, making it harder for the model to learn the association between the trigger and the target label. 
}
% Here is the refined approach to prove $P(t|\tilde{x},\xi,\triangle)<P(t|\tilde{x},\triangle)$ using Bayes' theorem, considering the condition that the target label $t$ is associated with both the presence of the trigger $\triangle$ on the sample $\tilde{x}+\xi+\triangle$ and the backdoor sample $\tilde{x}+\triangle$:\\
% where the target label $t$ is associated with the presence of the trigger $\triangle$, $\xi$ represents the masked information of the original training sample in the key frequency regions, $\tilde{x}$ is the original training sample with key regions masked:
% \begin{itemize}
1. Define the Probabilities:\\
$P(t|\tilde{x},\triangle,\xi=1)$: Probability of predicting target label $t$ given the sample $\tilde{x}$, the trigger $\triangle$ and the masked information of the sample in the key frequency regions $\xi$ being present.\\
$P(t|\tilde{x},\triangle,\xi=0)$: Probability of predicting target label $t$ given the sample $\tilde{x}$ and the trigger $\triangle$ being present.\\
2.Apply Bayes' Theorem:\\
\begin{equation}
P(t|\tilde{x},\xi,\triangle) = \frac{P(\tilde{x},\xi,\triangle | t) P(t)}{P(\tilde{x}, \xi, \triangle)}.
\label{Bayes_with_xi}
\end{equation}
\begin{equation}
P(t|\tilde{x},\triangle) = \frac{P(\tilde{x},\triangle | t) P(t)}{P(\tilde{x},  \triangle)}.
\end{equation}
3. Conditional Independence Assumption:\\
We can assume that masked information $\xi$ does not provide any additional information about the target label $t$ given the sample with the trigger $\tilde{x}+\triangle$ and the trigger $\triangle$. Therefore, we can state:\\
\begin{equation}
P(\tilde{x},\xi,\triangle | t) = P(\xi|\tilde{x},\triangle,t)P(\tilde{x},\triangle|t).
\label{1}
\end{equation}
Since $\xi$ doesn't provide additional information about $t$, we can further simplify:
\begin{equation}
P(\xi|\tilde{x},\triangle,t) = P(\xi|\tilde{x},\triangle).
\label{2}
\end{equation}
4. Substituting and Simplifying:\\
Considering Equ.~\ref{1} and ~\ref{2}, we substitute the conditional independence assumption into the ratio:
\begin{equation}
\frac{P(t|\tilde{x},\xi,\triangle)}{P(t|\tilde{x},\triangle)}=\frac{P(\xi|\tilde{x},\triangle)P(\tilde{x},\triangle|t)P(\tilde{x},\triangle)}{P(\tilde{x},\xi,\triangle)P(\tilde{x},\triangle|t)}.
\label{}
\end{equation}
Simplifying, we get:
\begin{equation}
\frac{P(t|\tilde{x},\xi,\triangle)}{P(t|\tilde{x},\triangle)}=\frac{P(\xi|\tilde{x},\triangle)P(\tilde{x},\triangle)}{P(\tilde{x},\xi,\triangle)}
\end{equation}
5. Interpretation:\\
(1) Analyzing $P(\xi|\tilde{x},\triangle)$: Argue that the $\xi$, given the sample $\tilde{x}$ with the trigger $\triangle$, provides limited or no additional information for predicting the target label $t$. This implies that $P(\xi|\tilde{x},\triangle)$ would be relatively small (\textit{i.e.}, $P(\xi|\tilde{x},\triangle)\rightarrow{0}$) or close to a uniform distribution.\\
(2) Comparing Probabilities of Sample Configurations:
The trigger $\triangle$ is the dominant factor influencing the prediction of the target label $t$ when present on the sample $\tilde{x}+\triangle$ or $\tilde{x}+\xi+\triangle$. This implies that the presence or absence of the $\xi$ should have a relatively minor impact on the overall probability $P(\tilde{x},\xi,\triangle)$ compared to $P(\tilde{x},\triangle)$.\\
(3) We conduct empirical experiments to complete the training process while preserving the original sample information and to generate poisoned testing samples in the same way as WPDA. Take CIFAR-10 as an example, Fig.~\ref{effect of original_information} demonstrates that the ASR of  preserving the original sample information in the training process is lower than that of masking the original sample information.\\
\begin{figure}[H]
\centering  %图片全局居中
    {
    \includegraphics[width=1.65in]{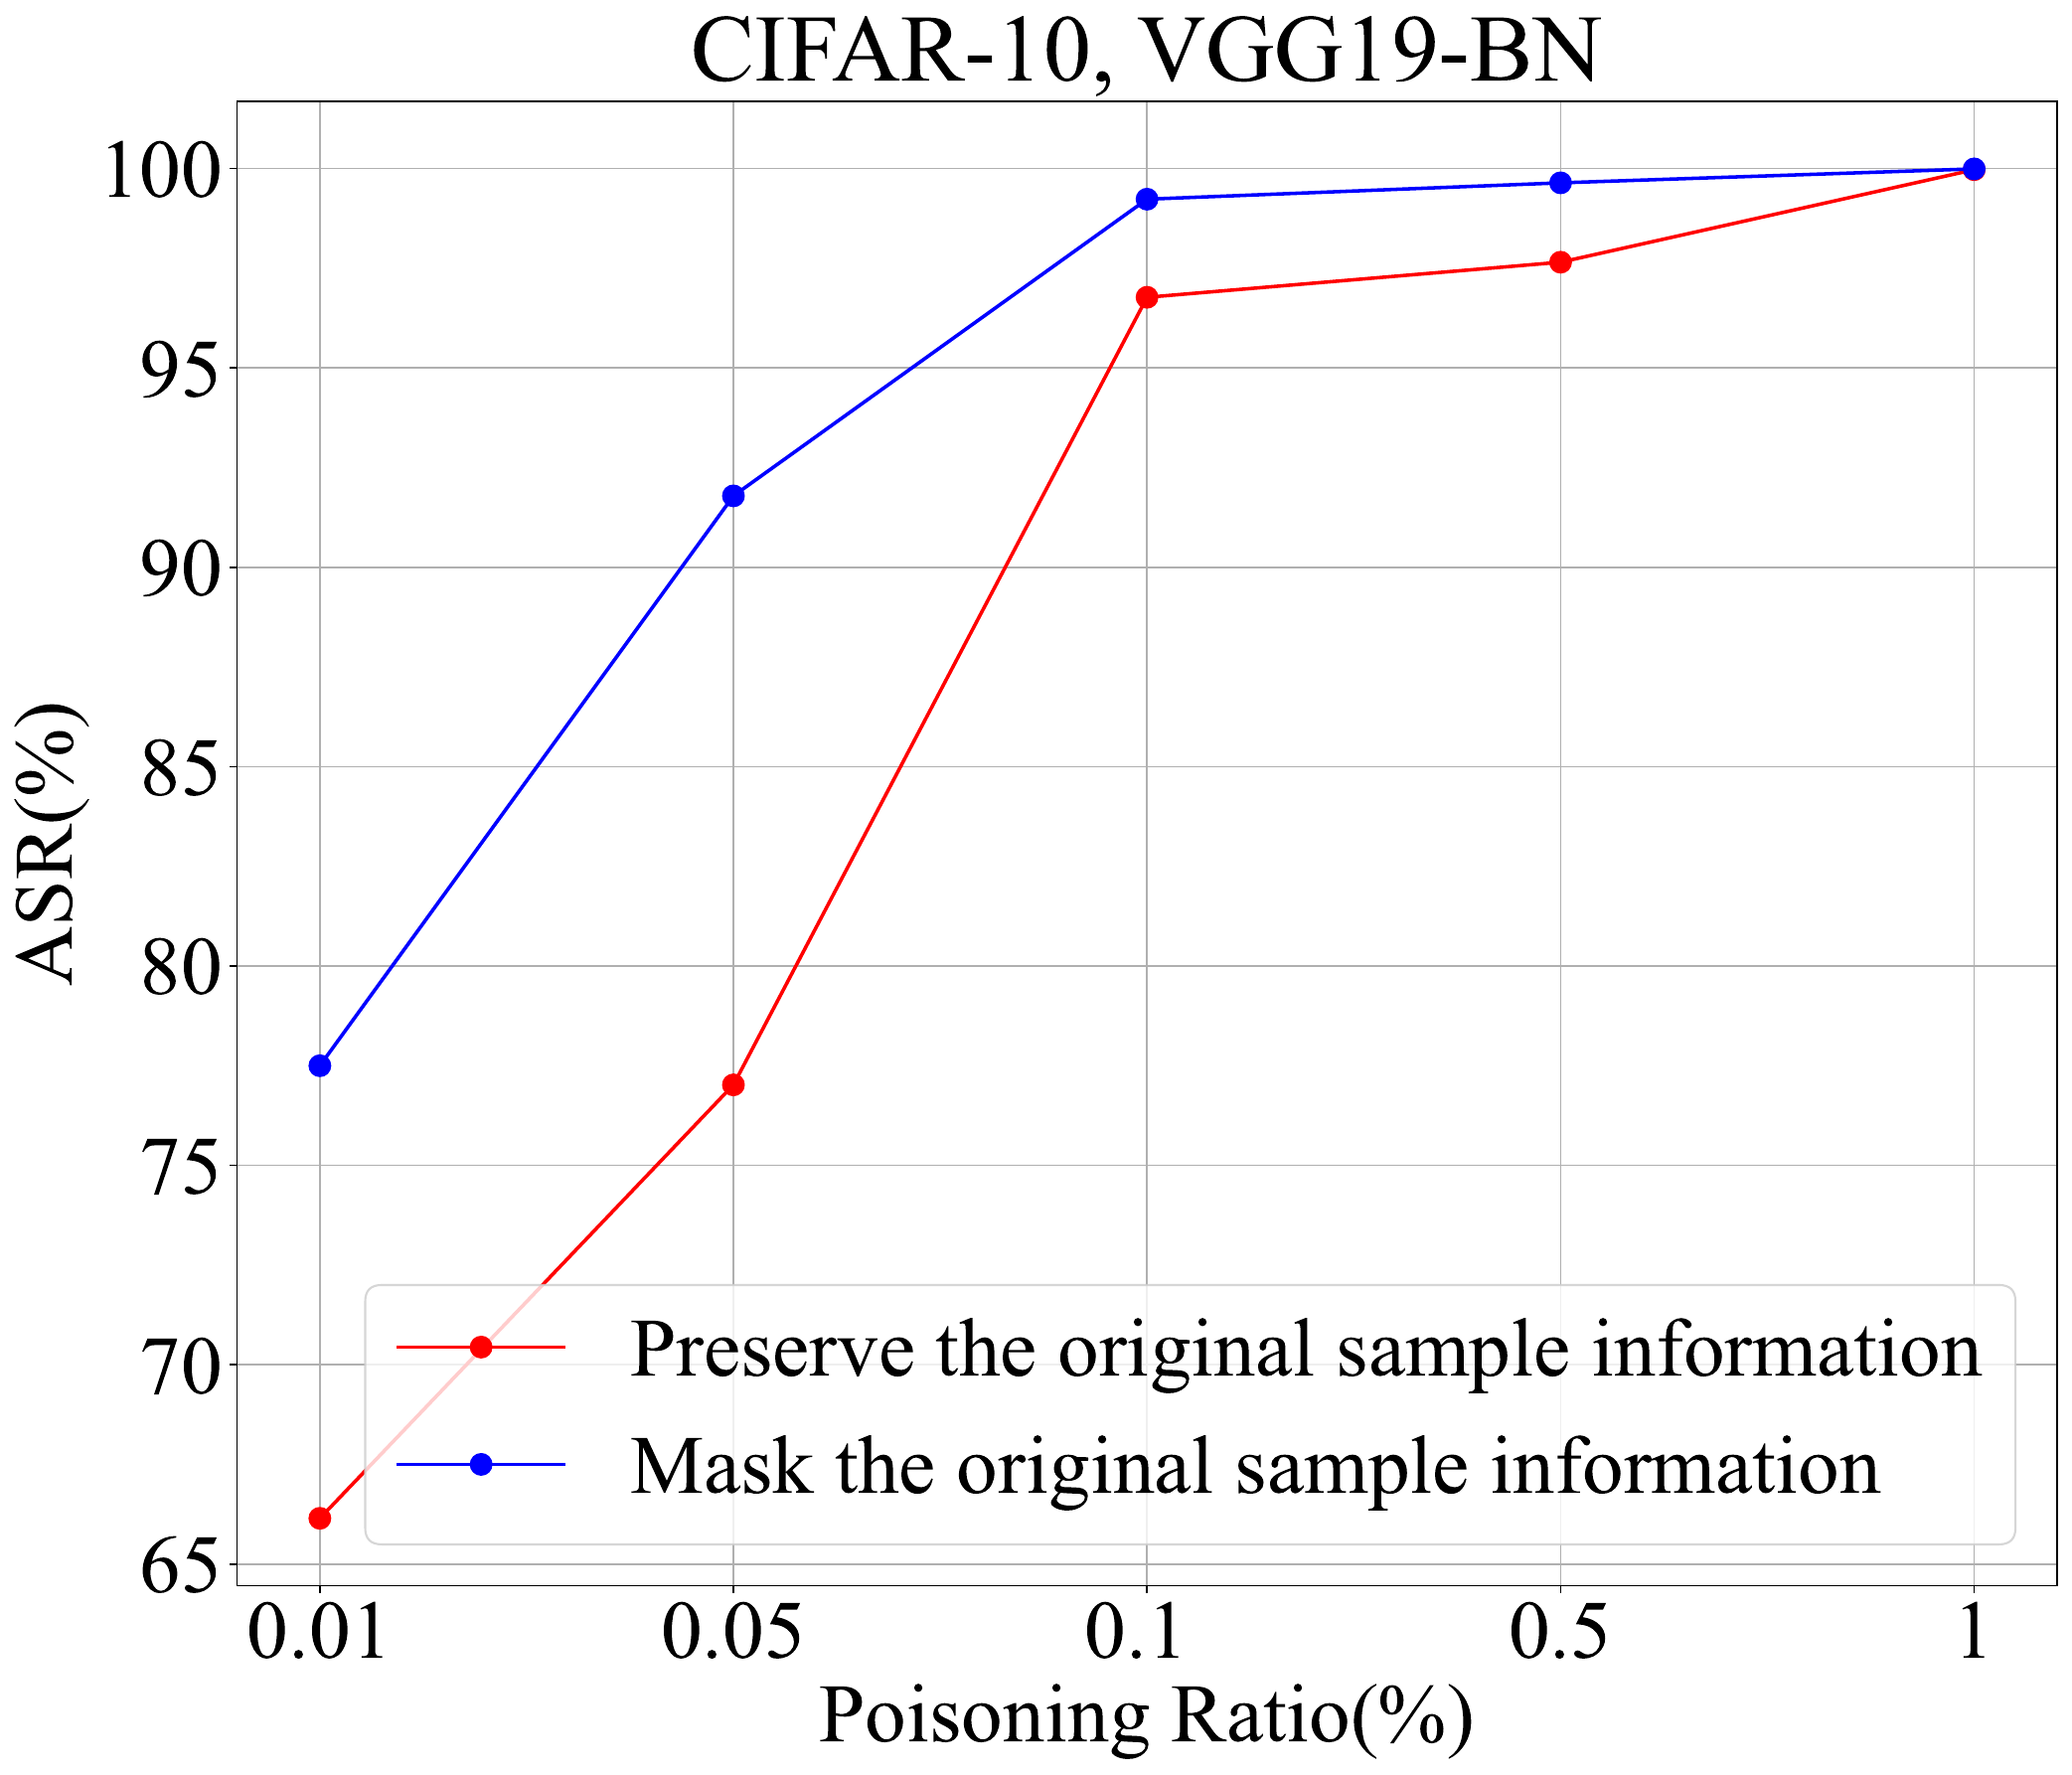}}
    \label{vgg19bn_original_information}
    {
    \includegraphics[width=1.65in]{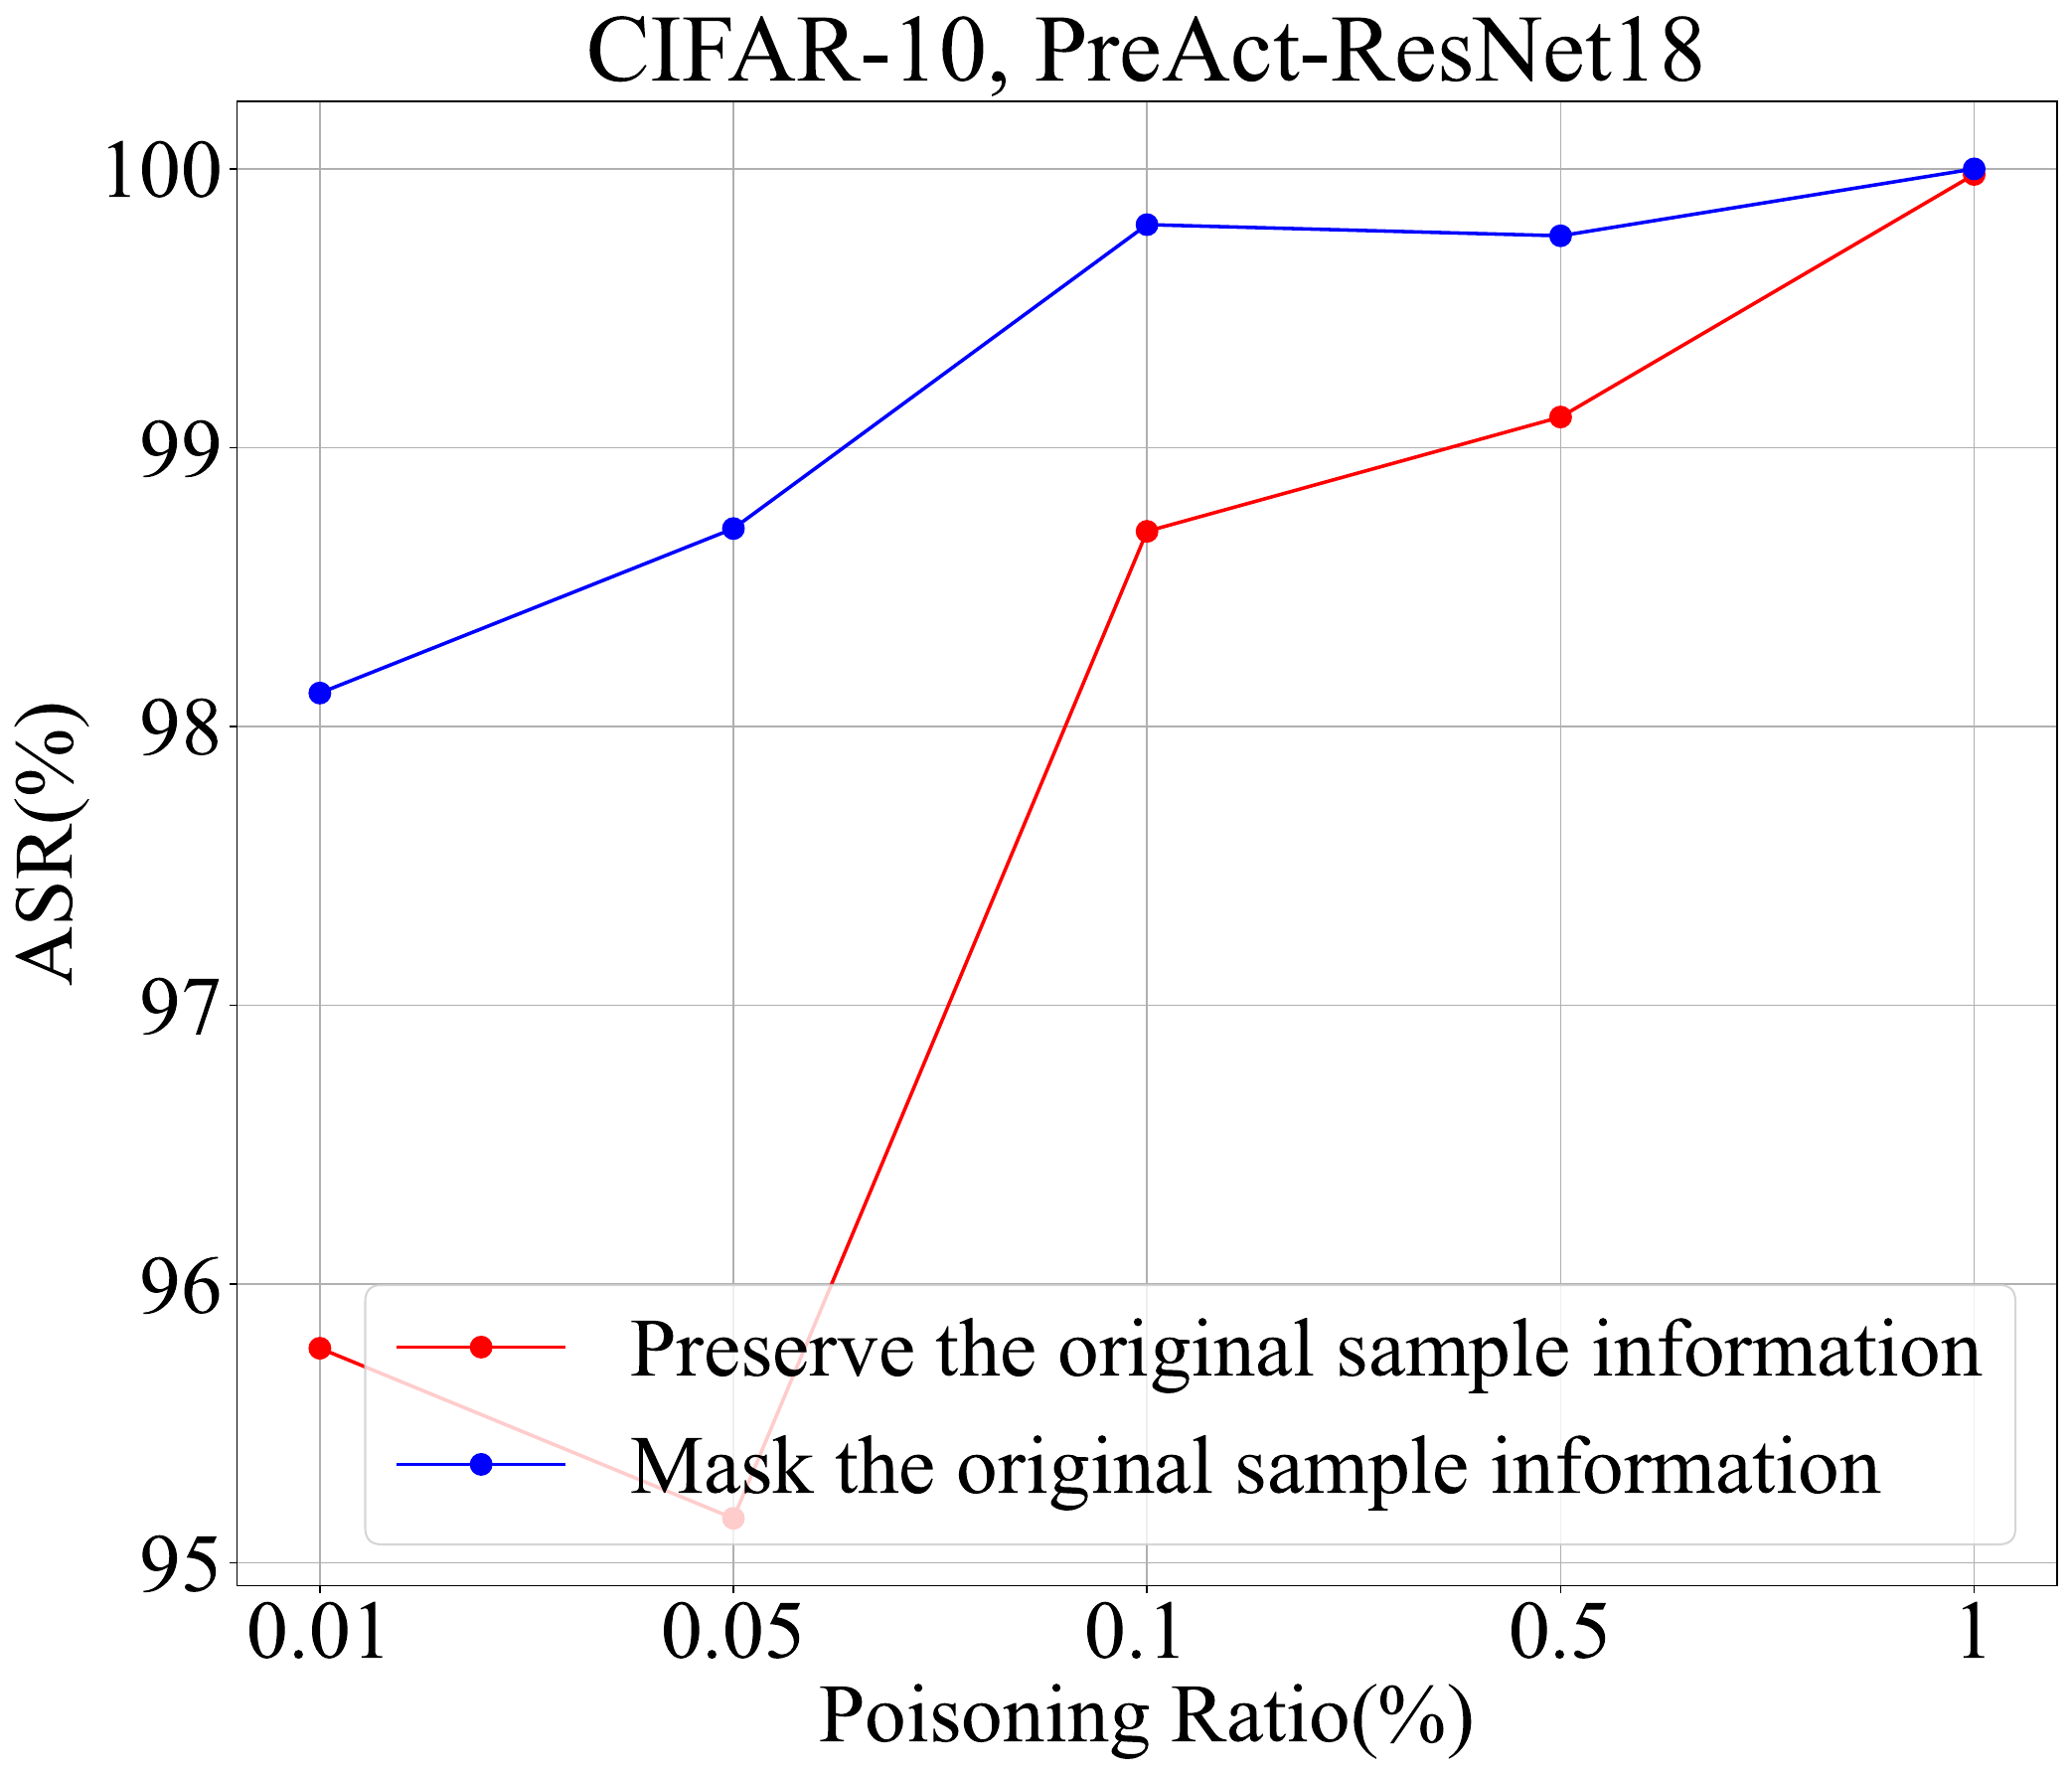}}
    \label{preactresnet18_original_information}
\caption{Effect of original information in key frequency regions on model learning triggers.}
\label{effect of original_information}
\end{figure}
\noindent6. Combining Evidence and Reasoning:\\
By combining theoretical reasoning and empirical evidence, we can infer $P(\xi|\tilde{x},\triangle)P(\tilde{x},\triangle)<P(\tilde{x},\xi,\triangle)$ , which ultimately supports the claim that $P(t|\tilde{x},\xi,\triangle)<P(t|\tilde{x},\triangle)$  and demonstrates the original sample information compete with the
trigger information for the model’s attention, making it
harder for the model to learn the association between the
trigger and the target label. 
% the negative effect of the original information on the model learning trigger.
% and analysis of specific backdoor attack scenarios, you can build a strong case for the inequality P(ξ|x, △, T=1) * P(x, △|T=1) < P(x, ξ, △|T=1), which ultimately supports the claim that P(t|x, ξ, △, T=1) / P(t|x, △, T=1) < 1 and demonstrates the suppressive effect of the original information on learning the trigger.

% given the target label $t$ and the trigger $\triangle$ presence, the masked information $\xi$ does not provide additional information about the specific configuration of the sample and trigger. Therefore:\\

% Using Bayes' theorem, we can write the probability of the model predicting the label $t$ given the original sample $x$ and the trigger $\xi$ as:
% $\tilde{x}$

\twocolumn
