# Supplementary material for: WPDA: Frequency-based Backdoor Attack with Wavelet Packet Decomposition
Source: arXiv:2401.13578 source file (2024-12-01)
Supplement: Supplementary file 2 [file 7_appendix_new2.tex]

\twocolumn[\section*{Supplementary}]
\newpage
% \section{Appendix}
% \appendix
\label{appendix}
% \section*{Appendix}
\setcounter{page}{1}
\subsection{\textbf{Verification}: Using the absolute average algorithm could potentially reduce sensitivity to noise compared to using the average absolute algorithm.
\label{explain why it is important to take the average value before taking the absolute value}
}

Due to the diverse sources of images in the dataset, factors such as sensors or environmental conditions may introduce disturbed noise. In Sec.~\ref{Analysis on dataset}, minimizing the impact of image noise is crucial for accurately quantifying the information in each frequency regions of the dataset. \textbf{Absolute average algorithm} refers to calculate the average of the coefficient matrix before calculating the absolute values. \textbf{Average absolute algorithm} refers to calculate the absolute of the coefficient matrix before calculating the average values. Compared to Average absolute algorithm, absolute average algorithm can more effectively minimize the overall impact of noise. For example, considering a sub-spectrogram with a coefficient matrix like [-3, +4, -2, +5], the absolute average value of the coefficient matrix is +1, and the average value of the coefficient matrix is +3.5. If noise causes small fluctuations, the coefficient matrix changes to [-3.1, +3.9, -1.9, +4.2]. As a result, the absolute average value of the coefficient matrix becomes +1.025, while the average absolute value becomes +3.275. The result demonstrates the absolute average algorithm is particularly effective at reducing the impact of noise on the quantification of information. Furthermore, we conduct experiments to confirm our conclusion. Take CIFAR-10 as an example, Fig.~\ref{abs mean} demonstrates that poisoned samples generated by the average absolute algorithm are less effective than those generated by absolute average algorithm. 

\begin{figure}[H]
\centering  %图片全局居中
    {
    \includegraphics[width=1.60in]{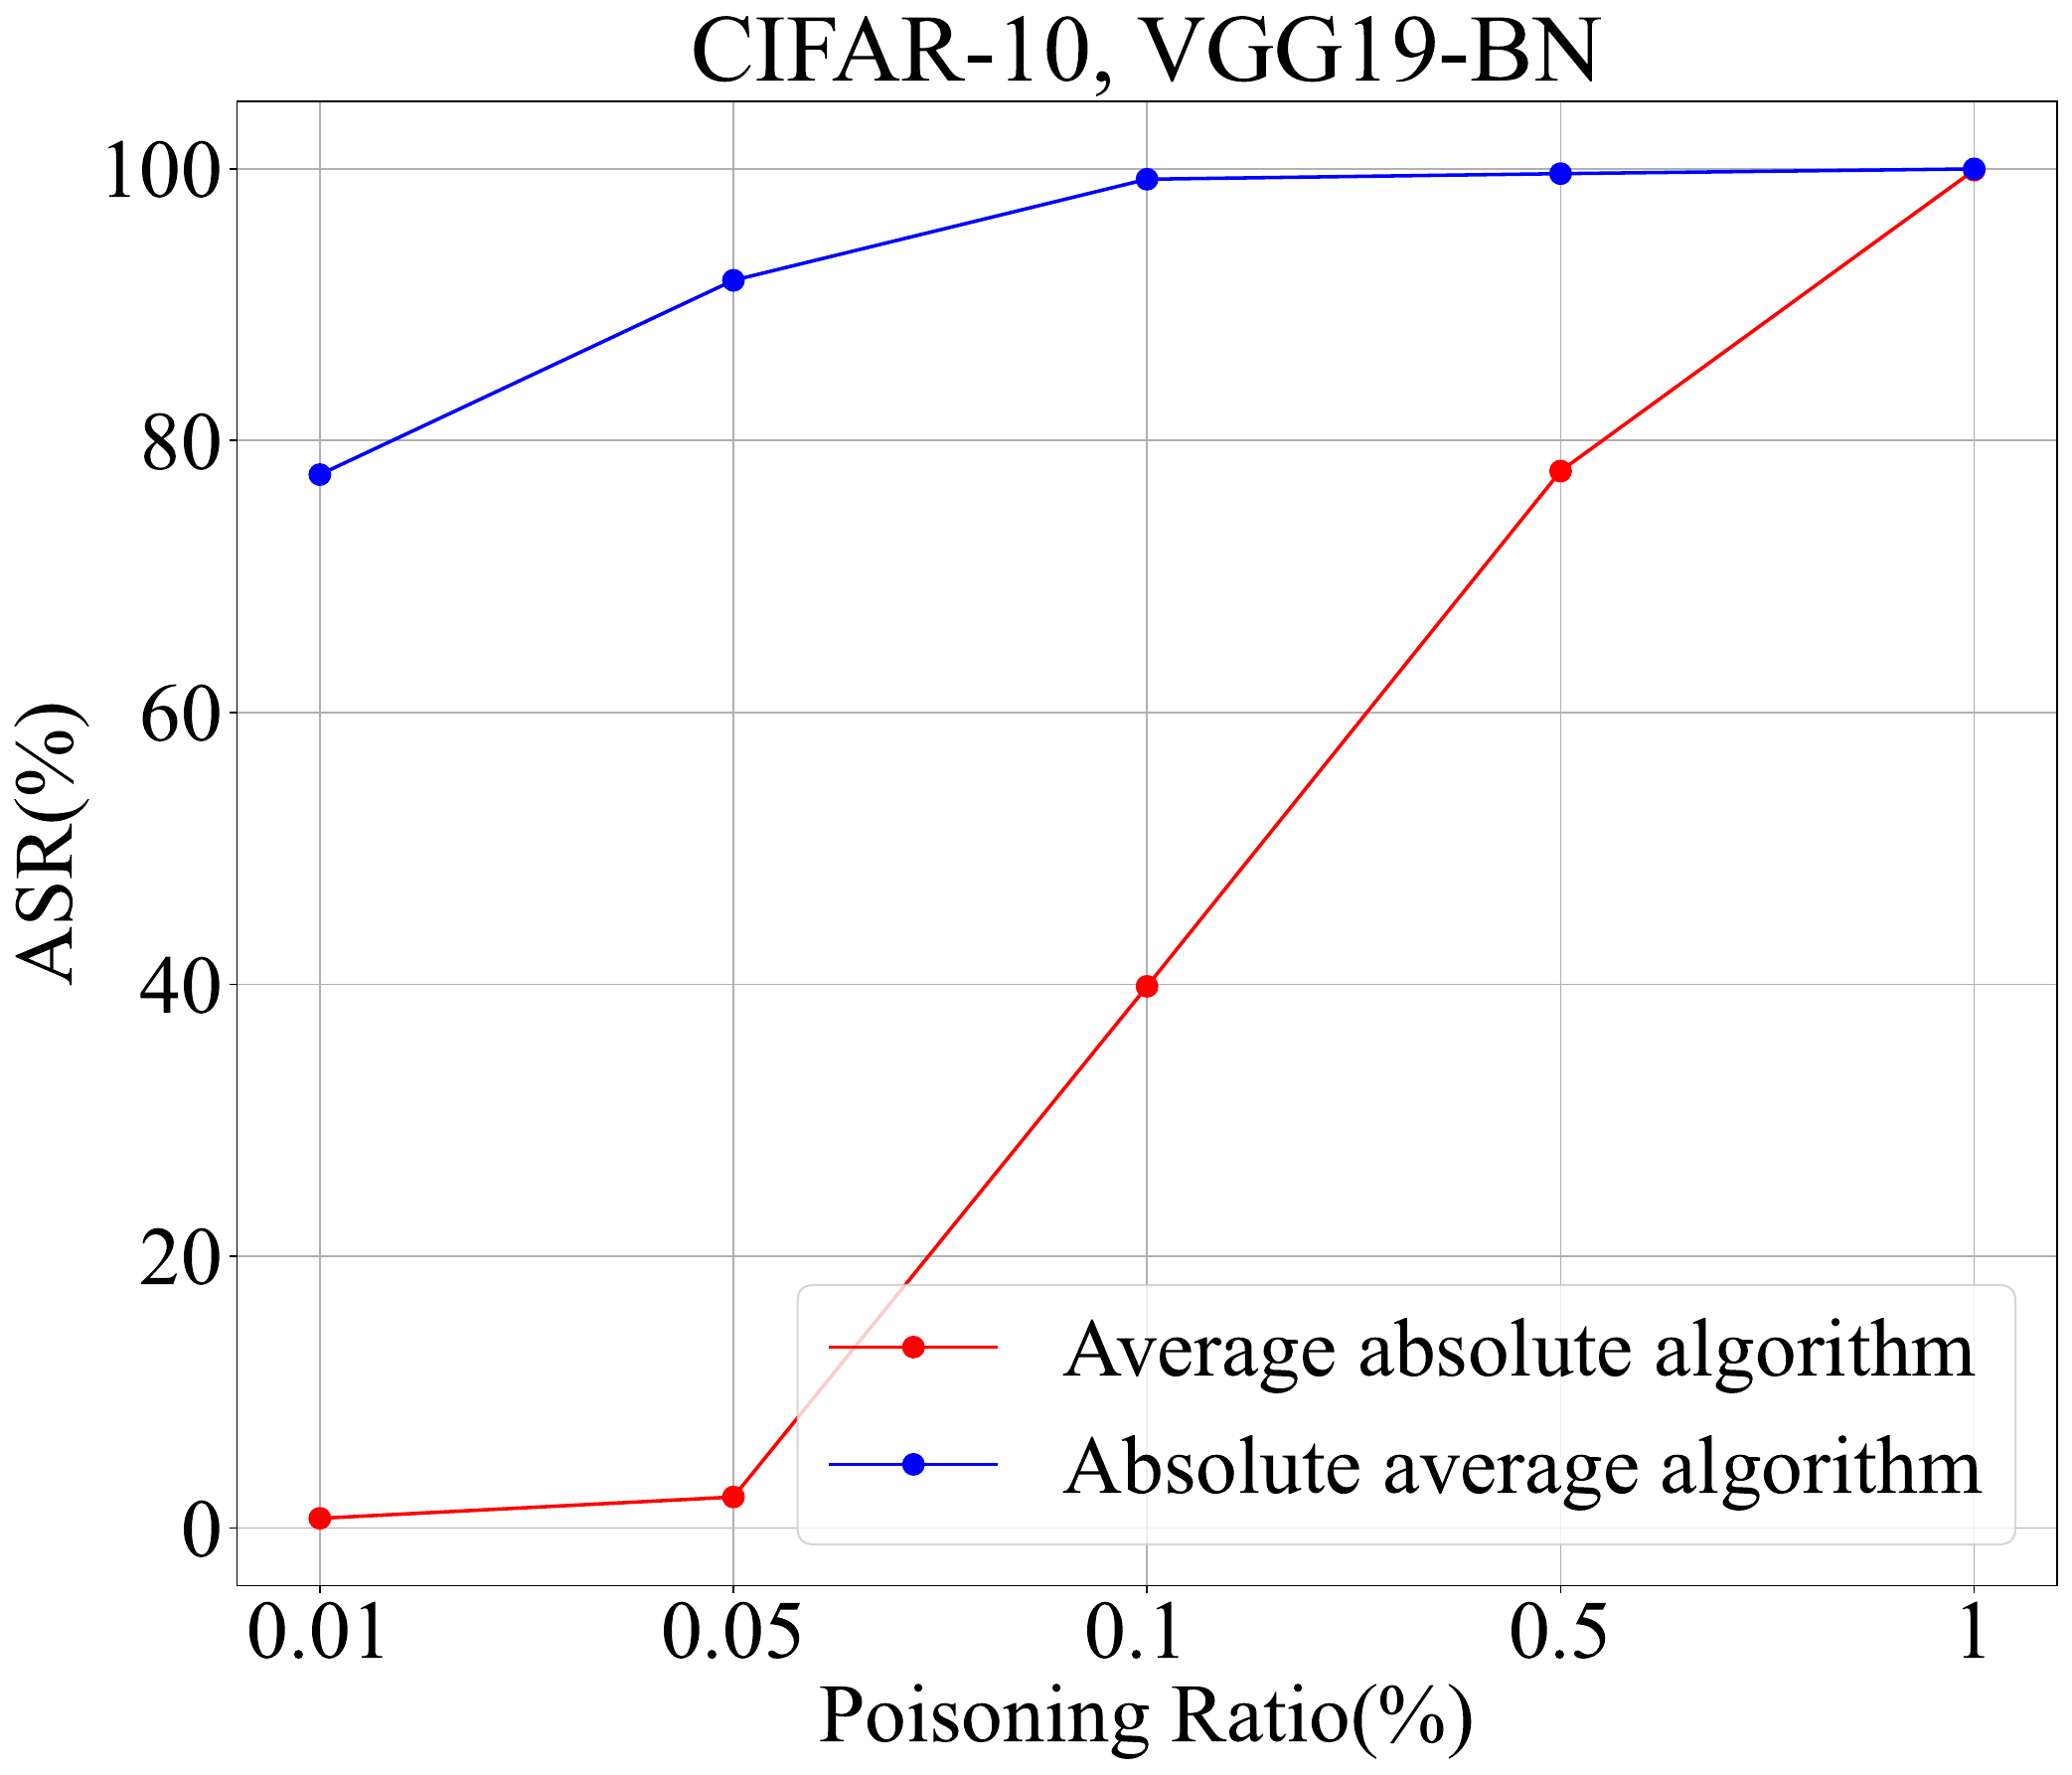}}
    \label{vgg19bn_abs_mean}
    {
    \includegraphics[width=1.60in]{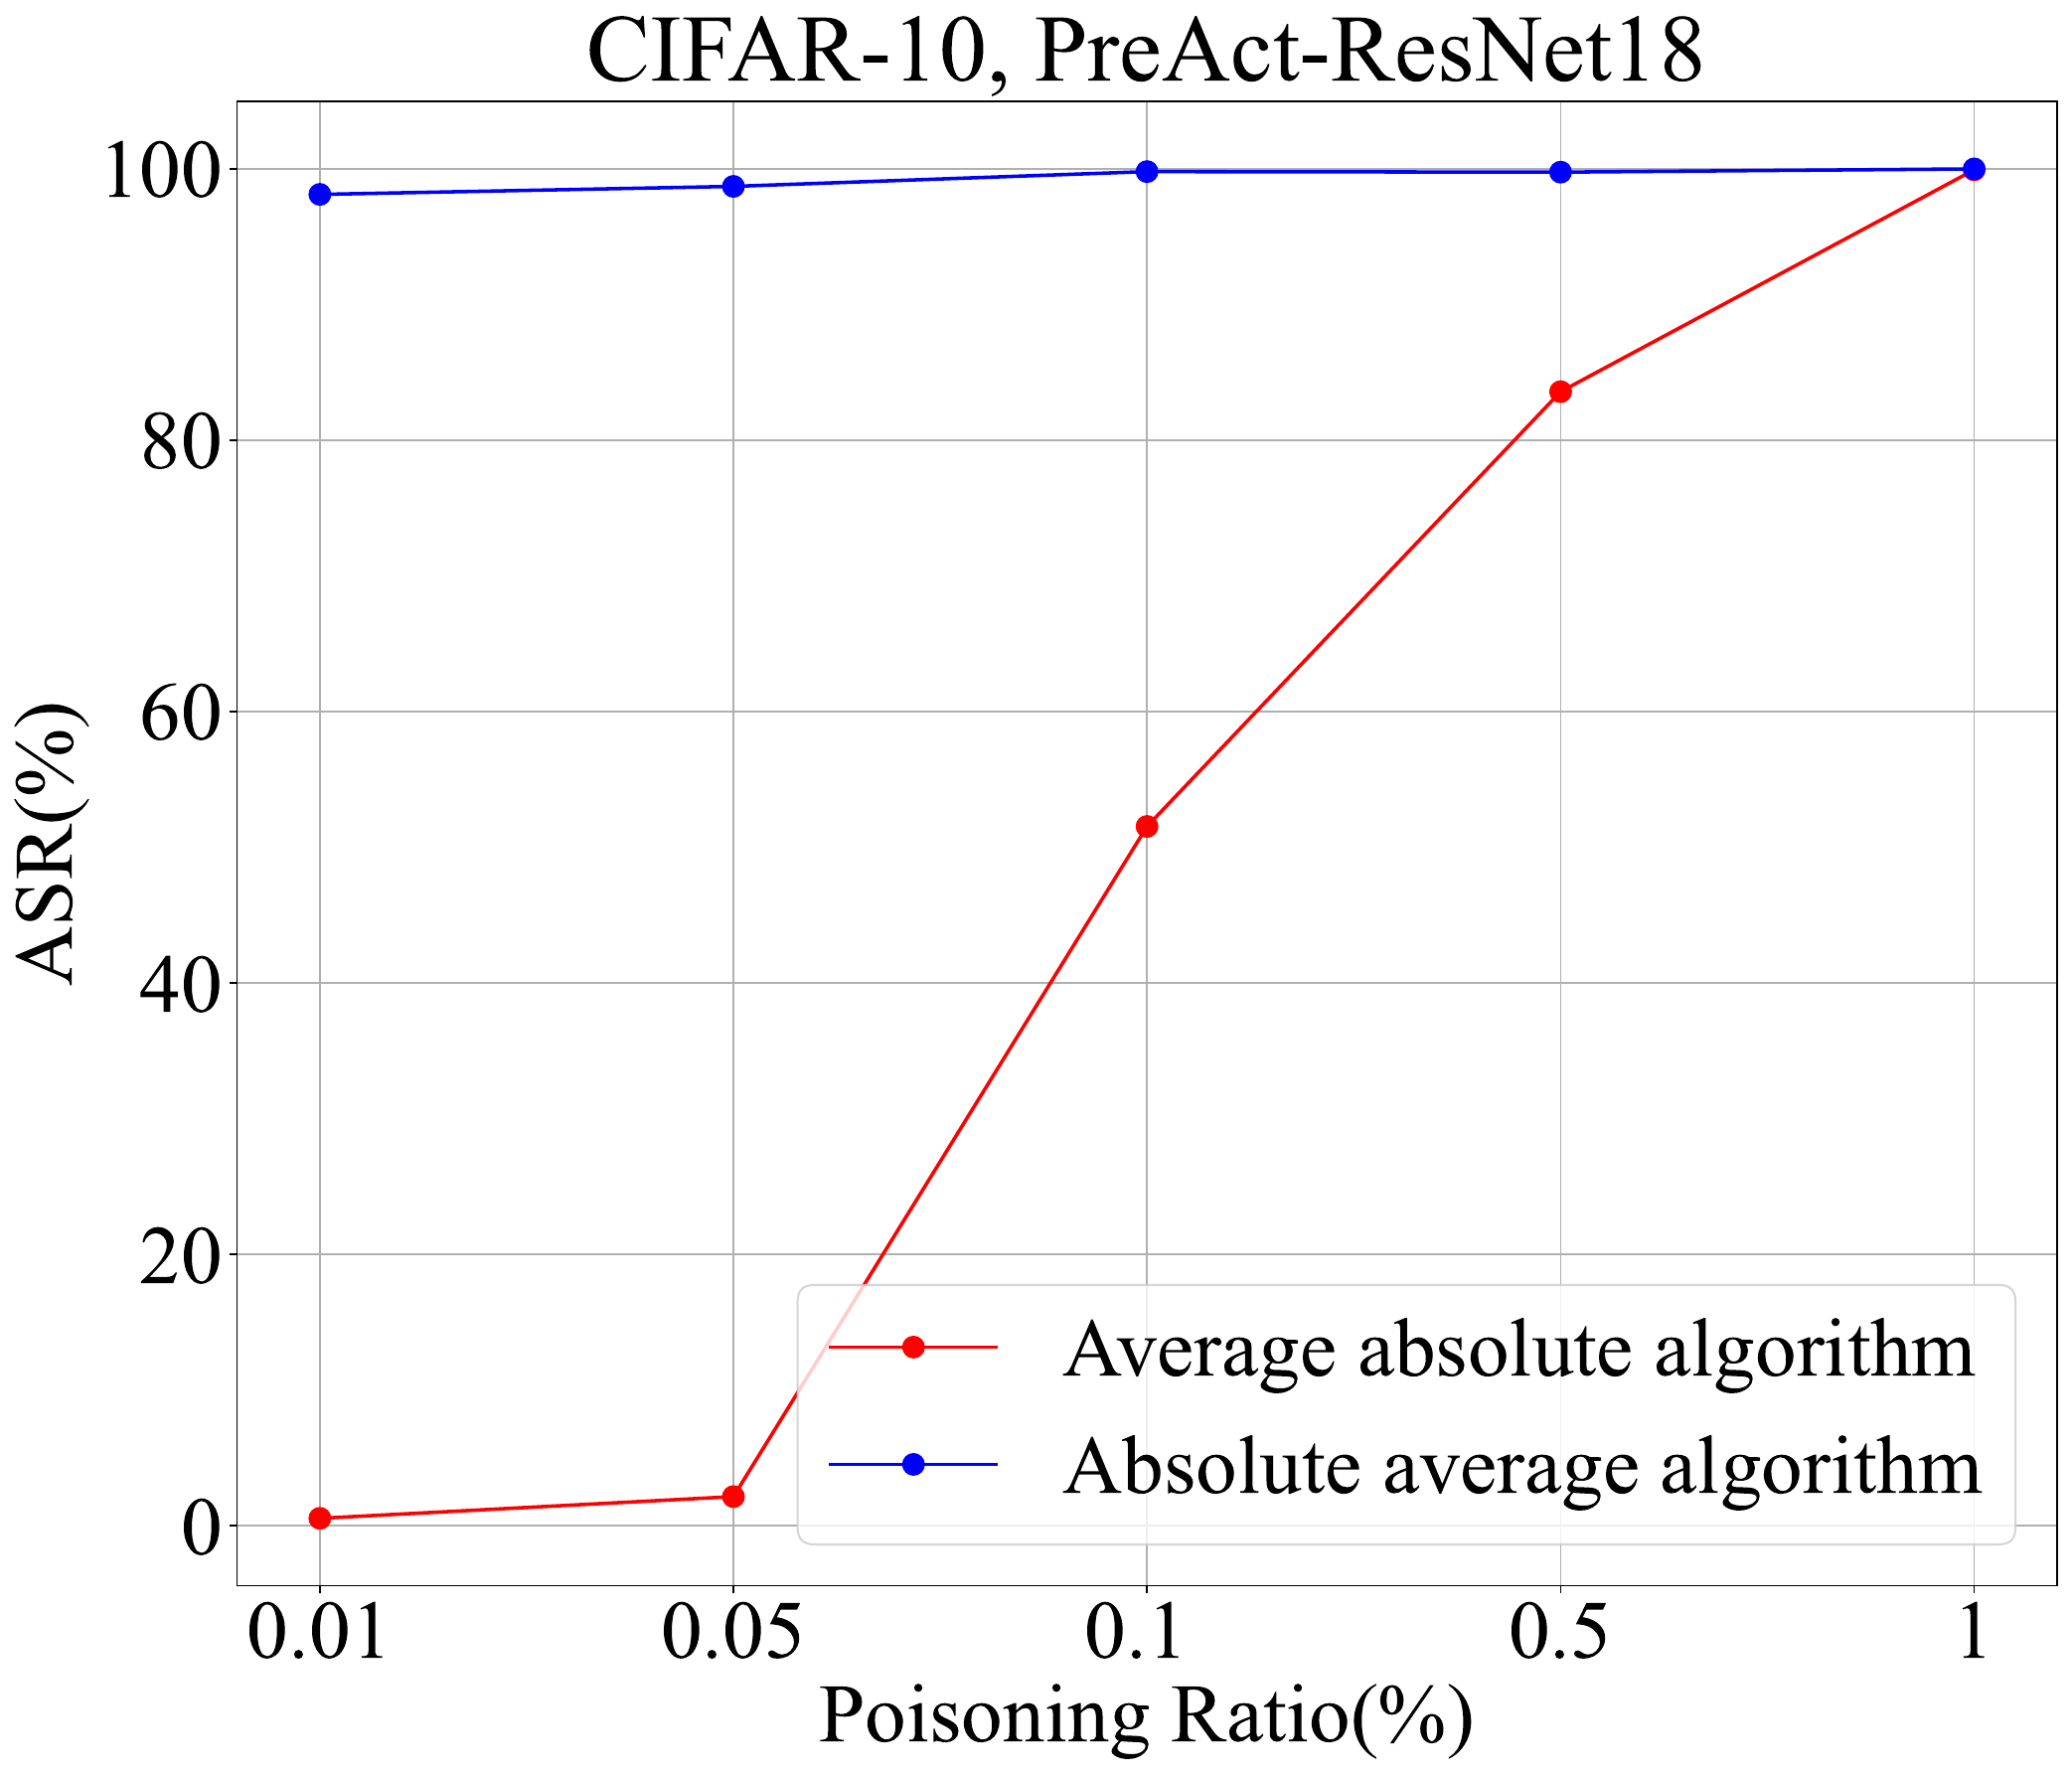}}
    \label{preactresnet18_abs_mean}
\caption{Performance of absolute average algorithm and average absolute algorithm.}
\label{abs mean}
% \vspace{-0.7cm}
\end{figure}
% \noindent\textbf{4. Combining Evidence and Reasoning:}
% By combining theoretical reasoning and empirical evidence, we can infer that absolute average algorithm can effectively reduce the effect of noise on the samples and help us accurately select key frequency regions.

\subsection{\textbf{Verification}:
\label{original information have negative effect on the backdoor activation}
The original benign sample information compete with the trigger information for the model’s attention, making it harder for the model to learn the association between the trigger and the target label. 
}
In Sec.~\ref{method}, we mask the information in the poisoning regions of the original samples when generating poisoned training samples (shown in Eq.~\ref{poisoned_training_samples_generation_equation}). This is based on the hypothesis that the original benign sample information might compete with the trigger information for the model’s attention, making it harder for the model to learn the association between the trigger and the target label. To verify this hypothesis, we conduct experiments to complete the training process while preserving the original benign sample information and to generate poisoned testing samples in the same way as WPDA. Take CIFAR-10 as an example, Fig.~\ref{effect of original_information} describes that the ASR of preserving the original benign sample information in the training process is lower than that of masking the original benign sample information, especially at low poisoning ratios. The results demonstrate a competition between the original benign sample information and trigger information. As an increased proportion of poisoned training samples,  the impact of the original benign sample information diminishes progressively. Consequently, for achieving effective backdoor attacks at low poisoning ratios, it becomes necessary to mask the original benign sample information in training process.
\begin{figure}[H]
\centering  %图片全局居中
    {
    \includegraphics[width=1.60in]{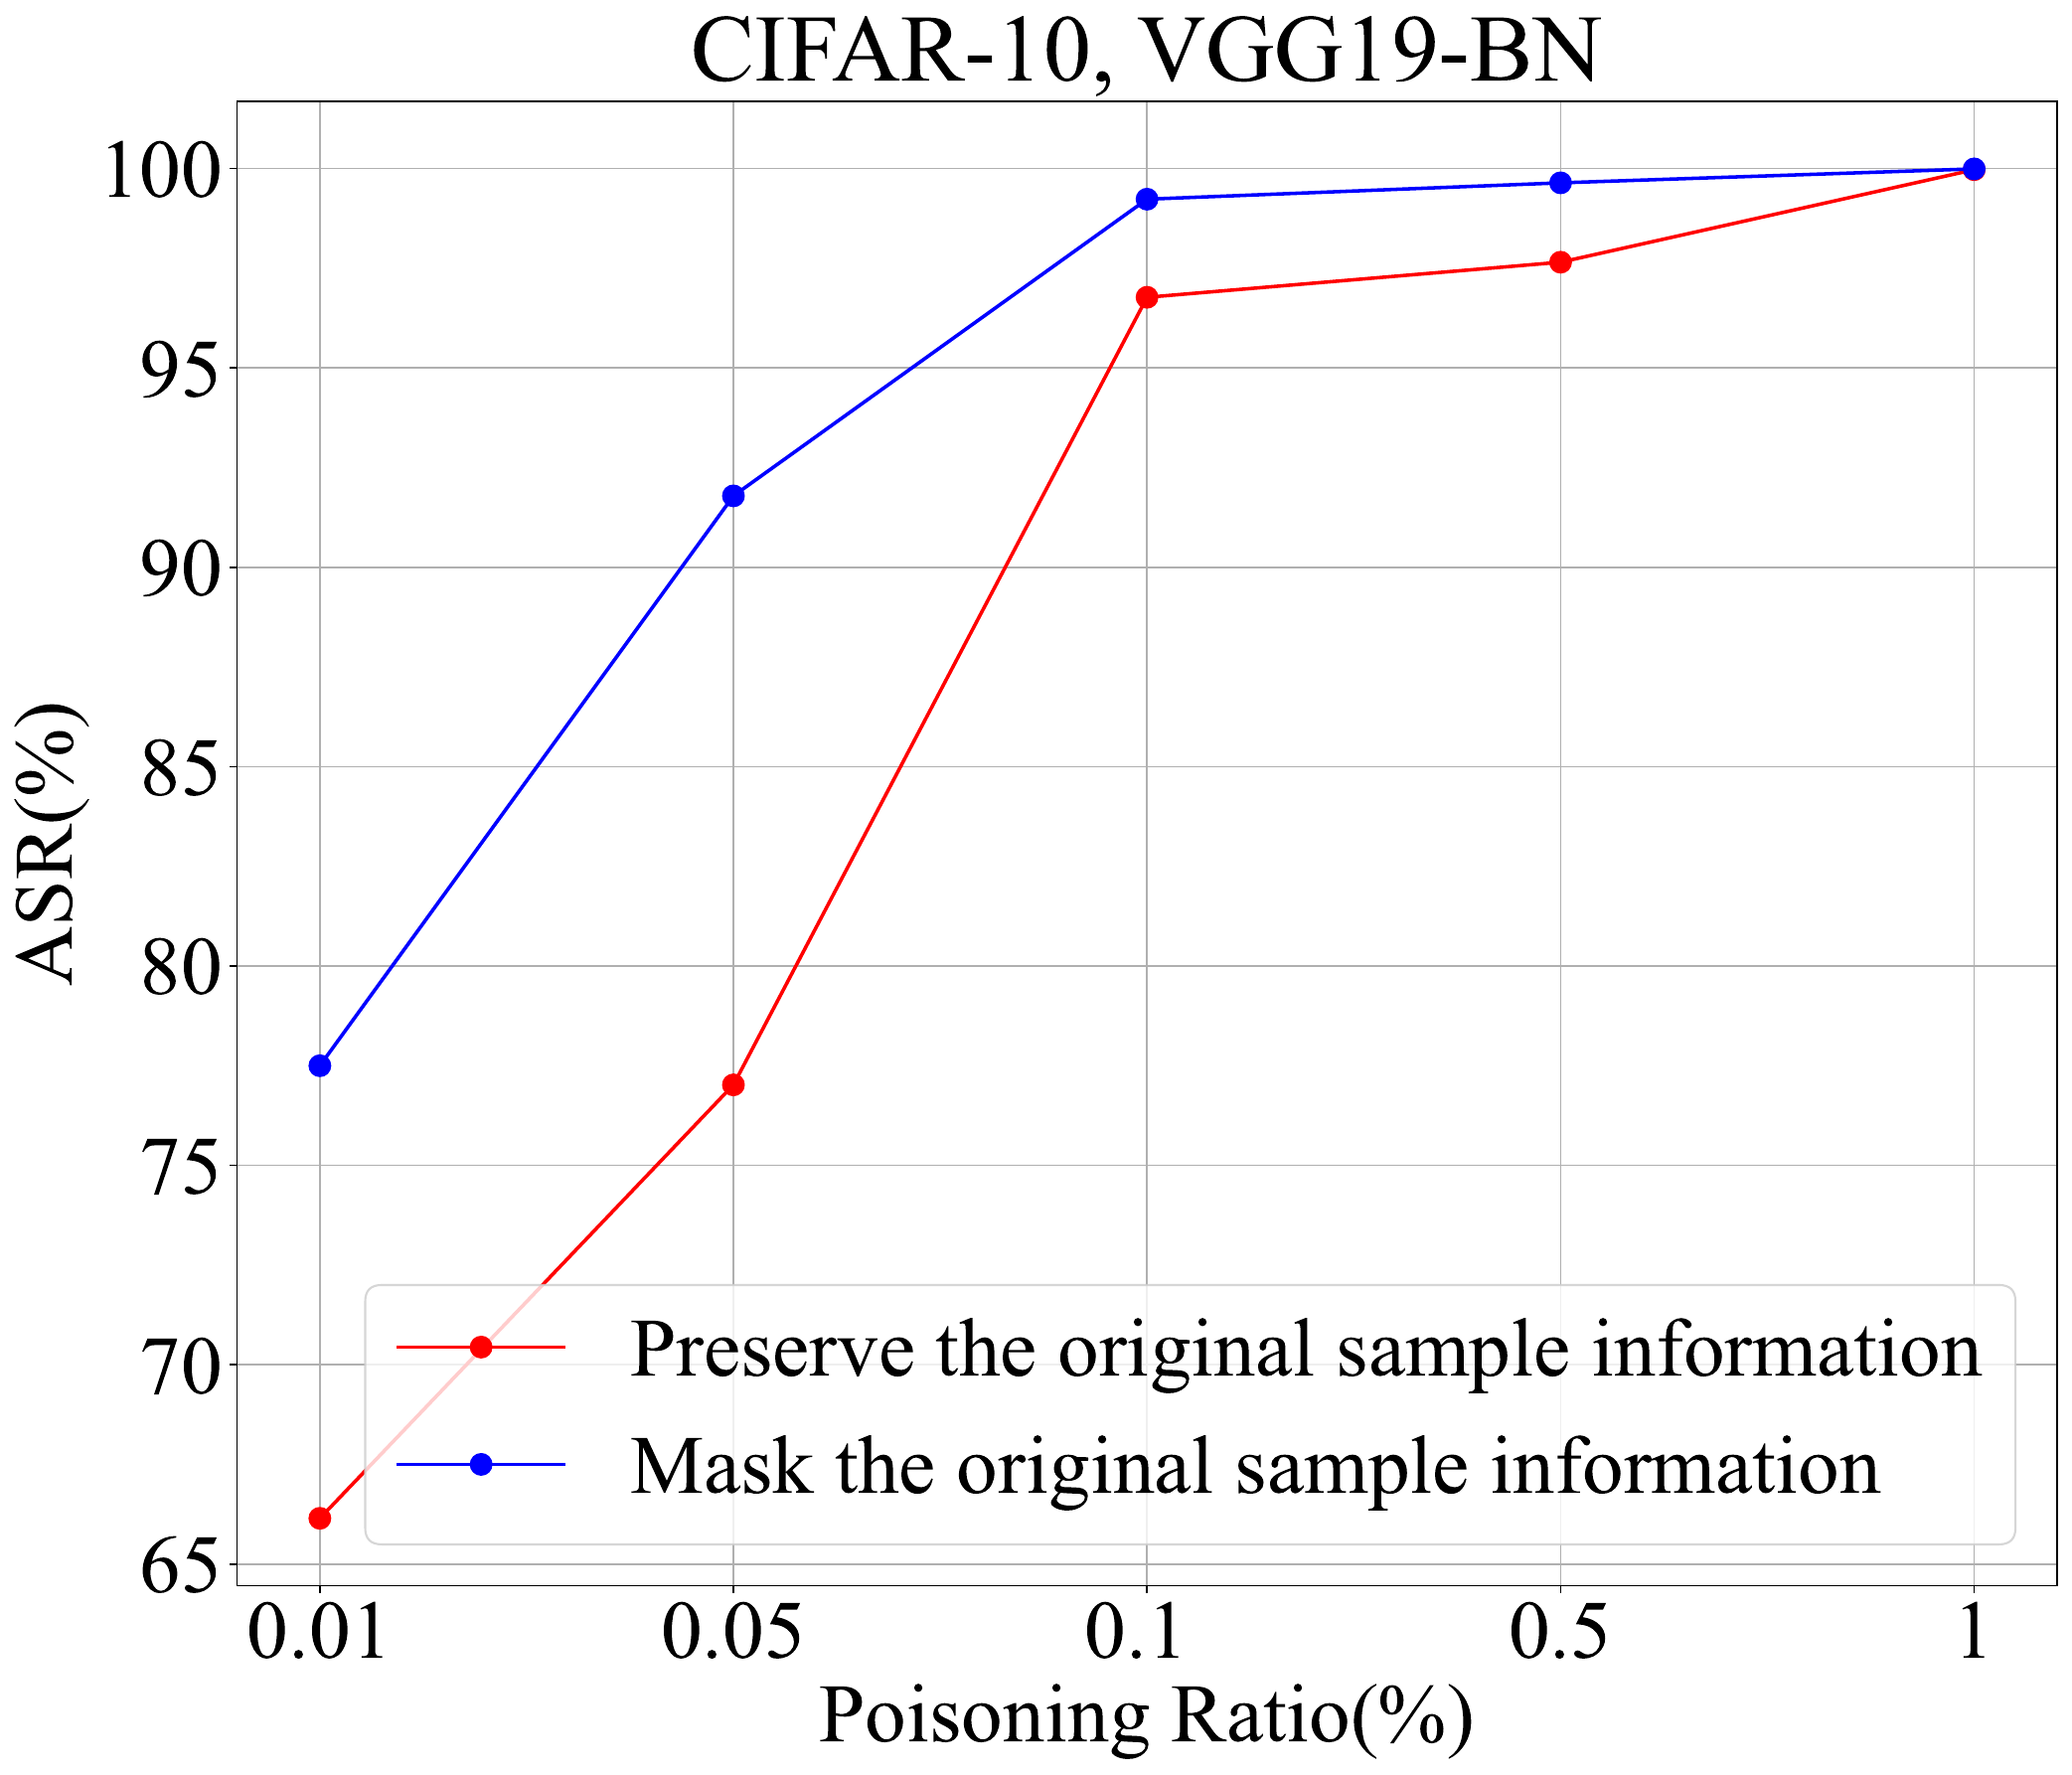}}
    \label{vgg19bn_original_information}
    {
    \includegraphics[width=1.60in]{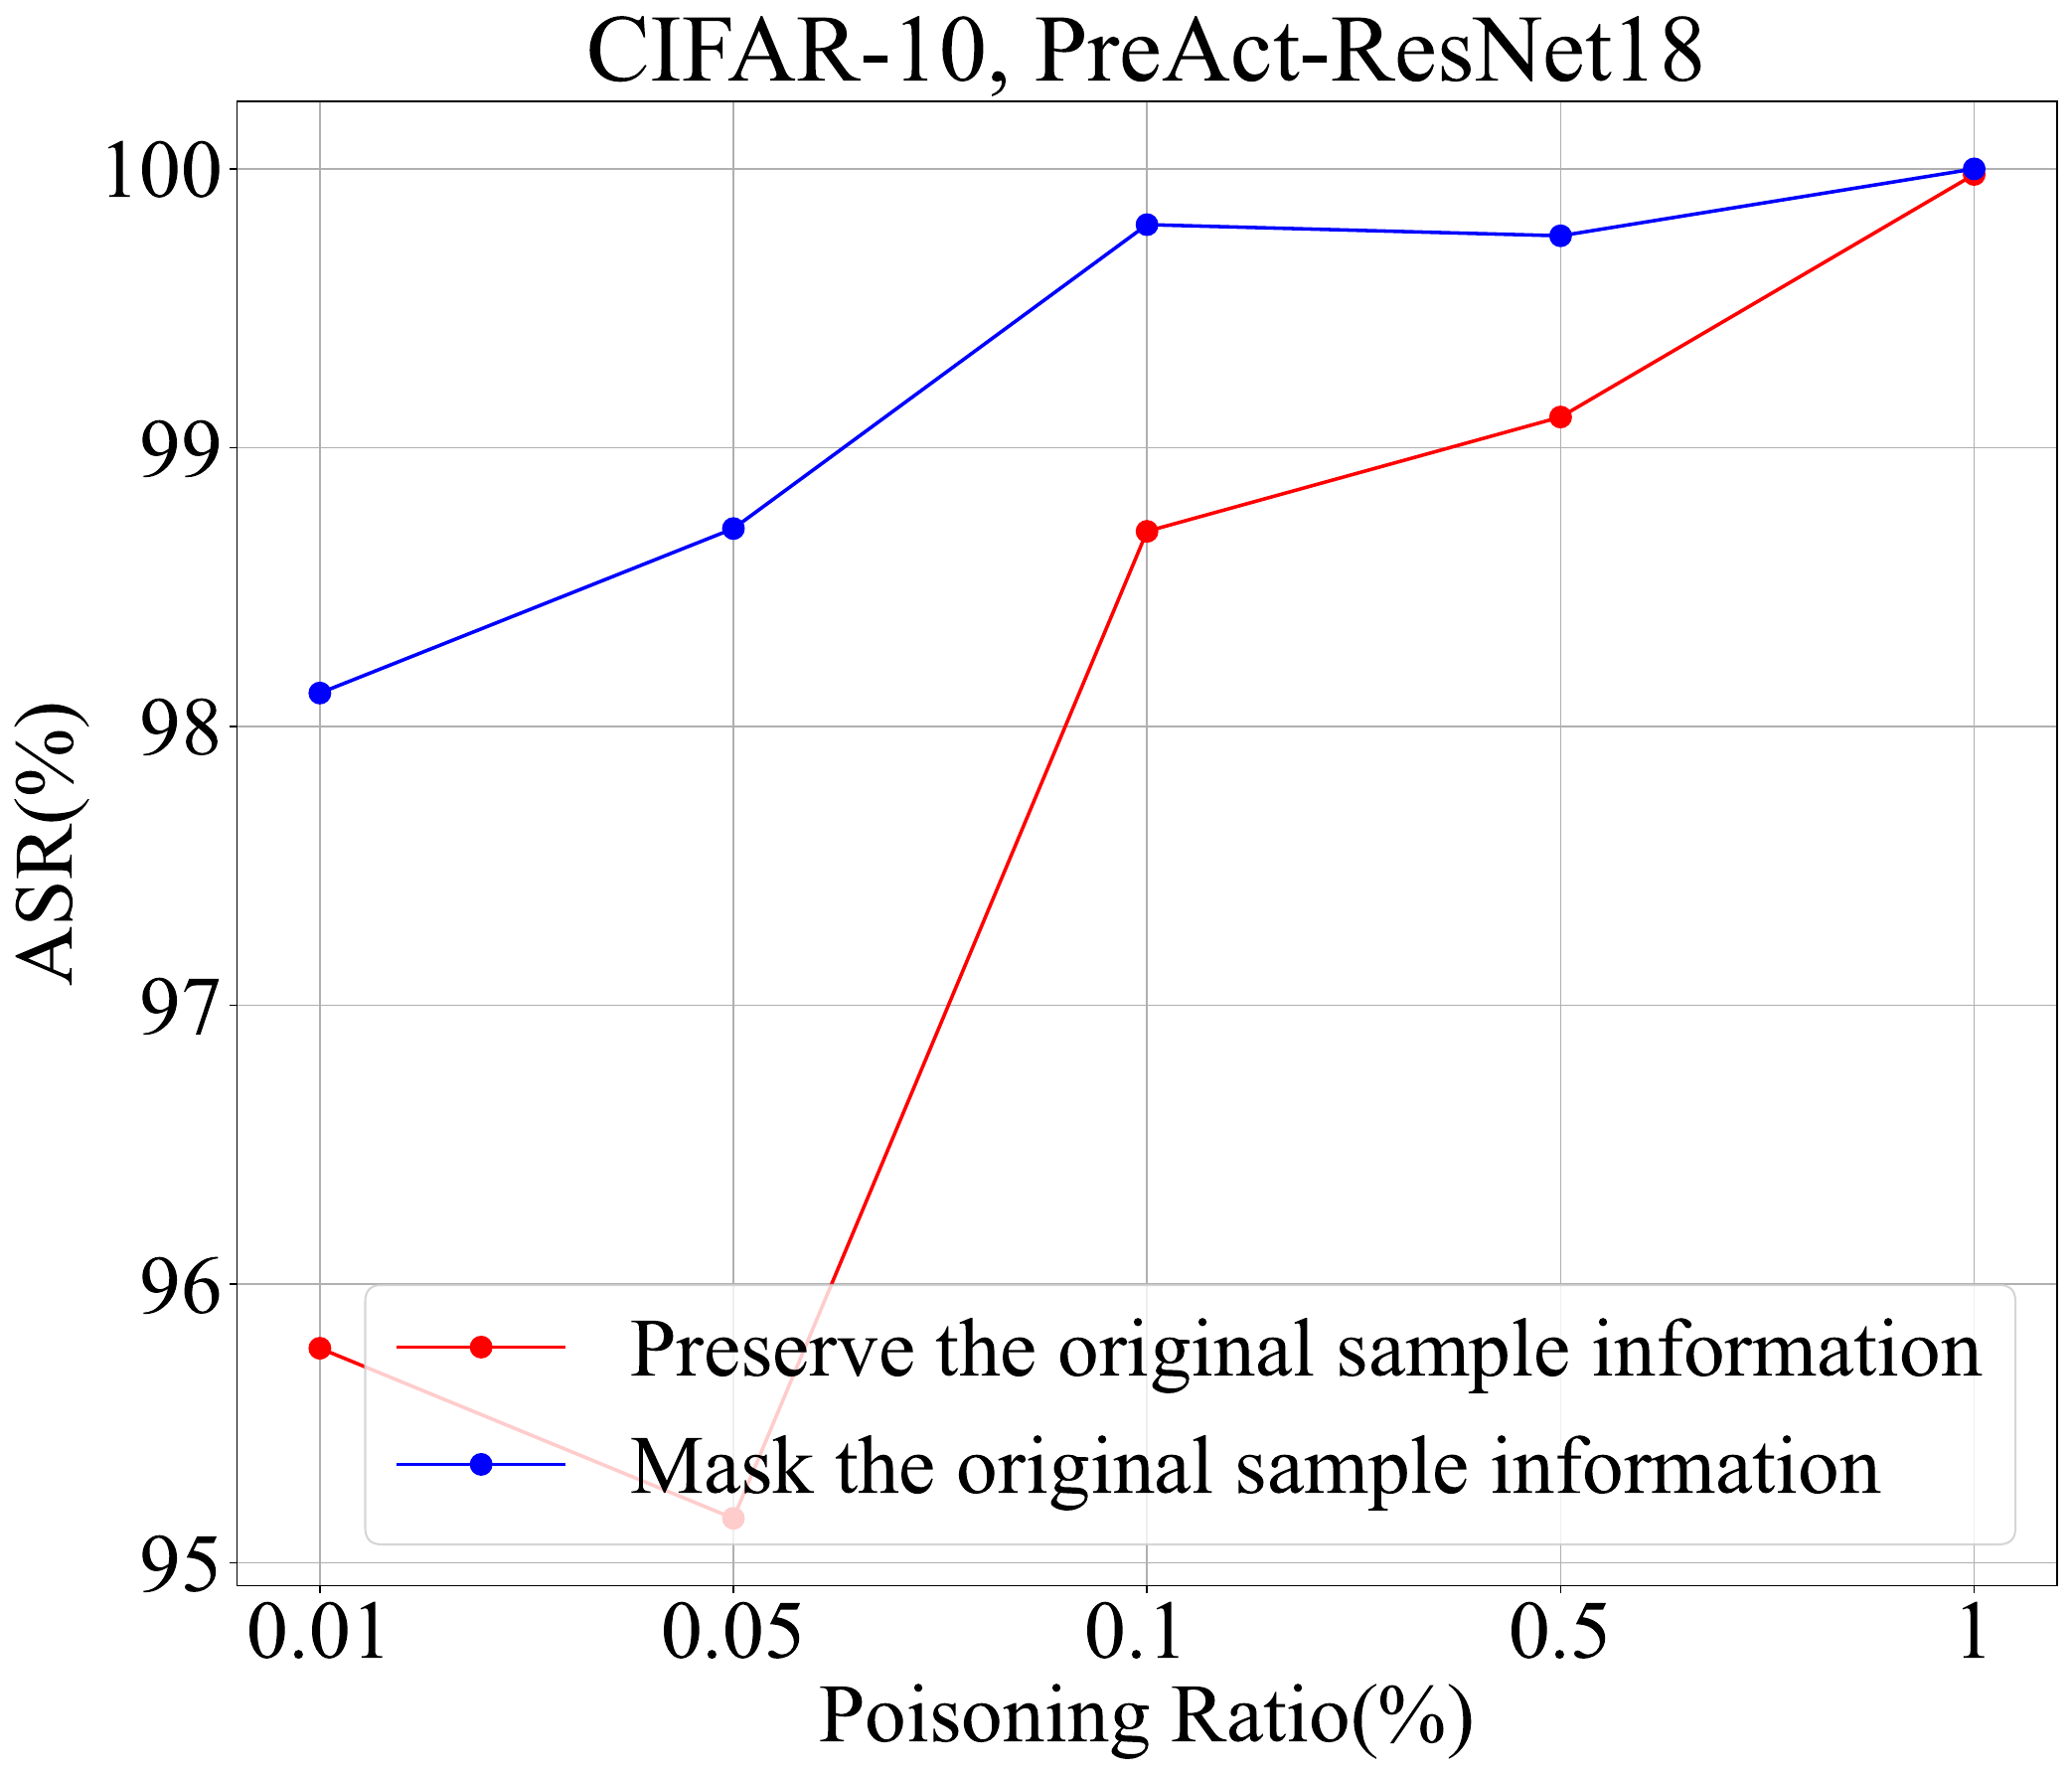}}
    \label{preactresnet18_original_information}
\caption{Effect of original benign sample information in key frequency regions on model learning triggers.}
\label{effect of original_information}
% \vspace{-0.5cm}
\end{figure}

\subsection{\textbf{Detection Performance of WPDA on PreAct-ResNet18}:
\label{detection on pre}}
In Tab.~\ref{detection_result_pre}, we evaluate the stealthiness performance of WPDA and other attacks under 3 SOTA backdoor detection methods on PreAct-ResNet18. It is worth noting that AC, SCAn and STRIP all rely on the model’s response to input samples (\textit{e.g.}, activations or predictions) to detect poisoned samples. As a result, variations in model architectures can lead to differences in detection performance.
\paragraph{\textbf{Evaluations on CIFAR-10}} AC and SCAn fail to detect any poisoned samples generated by WPDA across all 5 poisoning ratios. Regarding STRIP, it successfully detect part of poisoned samples and TPR gradually increases as the poisoning ratio rises, Fig.~\ref{STRIP detection pre} indicates that when the TPR reaches 93.80, the remaining poisoned samples still exhibit a backdoor effect, achieving a successful backdoor attack. The above results indicate that WPDA has great stealthiness, especially at low poisoning ratios.
\paragraph{\textbf{Evaluations on CIFAR-100}} The poisoned samples generated by WPDA evade detection of AC and SCAn across all 5 poisoning ratios. TPR in STRIP increases with the poisoning ratio, reaching 100.00\% at 1\% poisoning ratio, which indicates all poisoned samples are accurately detected. However, Fig.~\ref{STRIP detection pre} indicates that FPR of 8.31\% causes the model to misidentify many benign samples as poisoned, leading to a significant decline in C-Acc. The results indicate that WPDA demonstrates strong stealthiness, making it challenging for detection methods to accurately identify all poisoned samples without misidentifying benign samples as poisoned.
\paragraph{\textbf{Evaluations on Tiny ImageNet}} AC fails to detect any poisoned samples generated by WPDA across all 5 poisoning ratios. SCAn successfully detects 999 out of 1,000 poisoned samples at a 1\% poisoning ratio, eliminating the backdoor effect. However, at low poisoning ratios, the poisoned samples generated by WPDA all successfully evade detection of SCAn. 
% STRIP successfully detects a portion of the poisoned training samples across different poisoning ratios and TPR shows a positive correlation with the poisoning ratio, but STRIP misidentifies a large number of benign samples as poisoned, resulting in a decrease of C-Acc. For instance, the TPR reaches 95.70 at a 1\% poisoning ratio, meaning that 43 out of 1000 poisoned samples are not detected. The remaining poisoned samples still achieve successful backdoor attacks, as shown in Fig.~\ref{STRIP detection pre}.
The TPR of STRIP shows a positive correlation with the poisoning ratio and reaches 95.70 at a 1\% poisoning ratio, meaning that 43 out of 1000 poisoned samples are not detected. The remaining poisoned samples still achieve a successful backdoor attack, as shown in Fig.~\ref{STRIP detection pre}. At the meanwhile, STRIP misidentifies a large number of benign samples as poisoned, resulting in a decrease of C-Acc.
\paragraph{\textbf{Summary}}  Above results illustrate that 3 detection methods struggle to accurately identify all poisoned samples without misidentifying benign samples as poisoned, specially at low poisoning ratios, demonstrating the stealthiness of WPDA across different datasets and models.

\begin{table*}[!ht]
\caption{The result of WPDA against 3 detection methods under 5 different poisoning ratios in the datasets. The training model adopts PreAct-ResNet18. }
\label{detection_result_pre}
\centering
% \small
% \large
\normalsize
\scalebox{0.82}{
\resizebox{\textwidth}{!}{
    \begin{tabular}{m{.11\textwidth} m{.1\textwidth} m{.0355\textwidth}<{\centering} m{.0355\textwidth}<{\centering} m{.0355\textwidth}<{\centering} m{.0355\textwidth}<{\centering} m{.0355\textwidth}<{\centering} m{.0355\textwidth}<{\centering} m{.0355\textwidth}<{\centering} m{.0355\textwidth}<{\centering} m{.0355\textwidth}<{\centering} m{.0355\textwidth}<{\centering} m{.0355\textwidth}<{\centering} m{.0355\textwidth}<{\centering} m{.0355\textwidth}<{\centering} m{.0355\textwidth}<{\centering} m{.0355\textwidth}<{\centering} m{.0355\textwidth}<{\centering} m{.0355\textwidth}<{\centering} m{.0355\textwidth}<{\centering}} %{l l cc cc cc cc cc cc cc cc cc}
    \toprule
  \multirow{2}{*}{Dataset} & Poisoning ratio $\rightarrow$ & \multicolumn{3}{c}{0.004\%}        & \multicolumn{3}{c}{0.01\%}        & \multicolumn{3}{c}{0.05\%}        & \multicolumn{3}{c}{0.1\%}        & \multicolumn{3}{c}{1\%} 
\\
\cmidrule(lr){3-5} \cmidrule(lr){6-8} \cmidrule(lr){9-11} \cmidrule(lr){12-14} \cmidrule(lr){15-17} \cmidrule(lr){18-20}
 & Detection $\downarrow$  & \multicolumn{1}{c}{TPR }    & FPR     & $F^{\omega}_1$    & \multicolumn{1}{c}{TPR }    & FPR     & $F^{\omega}_1$    & \multicolumn{1}{c}{TPR }    & FPR     & $F^{\omega}_1$    & \multicolumn{1}{c}{TPR }    & FPR     & $F^{\omega}_1$    & \multicolumn{1}{c}{TPR }    & FPR     & $F^{\omega}_1$       
\\ 
\hline \hline 
\multirow{4}{*}{CIFAR10} & AC~\cite{chen2018detecting}     
& \multicolumn{1}{c}{0.00} & 0.00 & 0.00
& \multicolumn{1}{c}{0.00} & 0.00 & 0.00
& \multicolumn{1}{c}{0.00} & 0.00 & 0.00
& \multicolumn{1}{c}{0.00} & 0.00 & 0.00
& \multicolumn{1}{c}{0.00} & 0.00 & 0.00
\\ 
  & SCAn~\cite{tang2021demon} 
& \multicolumn{1}{c}{0.00} & 0.00 & 0.00 
& \multicolumn{1}{c}{0.00} & 0.00 & 0.00  
& \multicolumn{1}{c}{0.00} & 0.00 & 0.00  
& \multicolumn{1}{c}{0.00} & 0.00 & 0.00
& \multicolumn{1}{c}{0.00} & 0.00 & 0.00  
\\ 
%   & Spectral~\cite{tran2018spectral}  
% & \multicolumn{1}{c}{0.00} & 0.15 & 0.00 
% & \multicolumn{1}{c}{0.00} & 0.15 & 0.00 
% & \multicolumn{1}{c}{0.12} & 0.15 & 0.00  
% & \multicolumn{1}{c}{0.00} & 0.15 & 0.00  
% & \multicolumn{1}{c}{0.00} & 0.15 & 0.00
%   & Spectral~\cite{tran2018spectral}  
% & \multicolumn{1}{c}{0.00} & 15.00 & 0.00 
% & \multicolumn{1}{c}{0.00} & 15.00 & 0.00 
% & \multicolumn{1}{c}{12.00} & 15.01 & 0.08  
% & \multicolumn{1}{c}{0.00} & 15.02 & 0.00  
% & \multicolumn{1}{c}{0.00} & 15.16 & 0.00
% \\ 
  & STRIP~\cite{gao2019strip}    
& \multicolumn{1}{c}{50.00} & 8.00 & 0.05 
& \multicolumn{1}{c}{20.00} & 8.15 & 0.05 
& \multicolumn{1}{c}{44.00} & 8.29 & 0.51  
& \multicolumn{1}{c}{56.00} & 10.29 & 1.04  
& \multicolumn{1}{c}{93.80} & 12.25 & 12.88
\\
\hline
% \multirow{4}{*}{CIFAR-100}  &AC~\cite{chen2018detecting}     
% & \multicolumn{1}{c}{0.00} & 0.04 & 0.00
% & \multicolumn{1}{c}{0.00} & 0.03 & 0.00
% & \multicolumn{1}{c}{0.00} & 0.01 & 0.00
% & \multicolumn{1}{c}{0.00} & 0.03 & 0.00
% & \multicolumn{1}{c}{0.00} & 0.02 & 0.00
% \\ 
%   &SCAn~\cite{tang2021demon} 
% & \multicolumn{1}{c}{0.00} & 0.00 & 0.00 
% & \multicolumn{1}{c}{0.00} & 0.00 & 0.00  
% & \multicolumn{1}{c}{0.00} & 0.00 & 0.00  
% & \multicolumn{1}{c}{0.00} & 0.00 & 0.00
% & \multicolumn{1}{c}{0.00} & 0.00 & 0.00  
% \\ 
%   &Spectral~\cite{tran2018spectral}  
% & \multicolumn{1}{c}{1.00} & 0.15 & 0.00 
% & \multicolumn{1}{c}{1.00} & 0.15 & 0.00 
% & \multicolumn{1}{c}{0.00} & 0.15 & 0.00  
% & \multicolumn{1}{c}{1.00} & 0.15 & 0.01  
% & \multicolumn{1}{c}{0.00} & 0.15 & 0.00
% \\ 
%   &STRIP~\cite{gao2019strip}    
% & \multicolumn{1}{c}{0.00} & 0.12 & 0.00 
% & \multicolumn{1}{c}{0.00} & 0.13 & 0.00 
% & \multicolumn{1}{c}{0.48} & 0.13 & 0.00  
% & \multicolumn{1}{c}{0.78} & 0.13 & 0.01  
% & \multicolumn{1}{c}{1.00} & 0.13 & 0.14
\multirow{4}{*}{CIFAR-100}  &AC~\cite{chen2018detecting}     
& \multicolumn{1}{c}{0.00} & 0.97 & 0.00
& \multicolumn{1}{c}{0.00} & 0.28 & 0.00
& \multicolumn{1}{c}{0.00} & 0.48 & 0.00
& \multicolumn{1}{c}{0.00} & 0.92 & 0.00
& \multicolumn{1}{c}{0.00} & 0.93 & 0.00
\\ 
  &SCAn~\cite{tang2021demon} 
& \multicolumn{1}{c}{0.00} & 0.00 & 0.00 
& \multicolumn{1}{c}{0.00} & 0.00 & 0.00  
& \multicolumn{1}{c}{0.00} & 0.00 & 0.00  
& \multicolumn{1}{c}{0.00} & 0.00 & 0.00
& \multicolumn{1}{c}{0.00} & 0.00 & 0.00  
% \\ 
%   &Spectral~\cite{tran2018spectral}  
% & \multicolumn{1}{c}{100.00} & 30.00 & 0.03 
% & \multicolumn{1}{c}{100.00} & 30.00 & 0.07 
% & \multicolumn{1}{c}{0.00} & 15.02 & 0.00  
% & \multicolumn{1}{c}{100.00} & 30.00 & 0.66 
% & \multicolumn{1}{c}{0.00} & 15.22 & 0.00
\\ 
  &STRIP~\cite{gao2019strip}    
& \multicolumn{1}{c}{0.00} & 14.66 & 0.00 
& \multicolumn{1}{c}{0.00} & 12.56 & 0.00 
& \multicolumn{1}{c}{48.00} & 13.06 & 0.36  
& \multicolumn{1}{c}{76.00} & 12.47 & 1.19  
& \multicolumn{1}{c}{100.00} & 8.31 & 19.56
\\
\hline
% \multirow{4}{*}{Tiny ImageNet}  &AC~\cite{chen2018detecting}     
% & \multicolumn{1}{c}{0.00} & 0.01 & 0.00
% & \multicolumn{1}{c}{0.00} & 0.01 & 0.00
% & \multicolumn{1}{c}{0.00} & 0.01 & 0.00
% & \multicolumn{1}{c}{0.00} & 0.01 & 0.00
% & \multicolumn{1}{c}{0.00} & 0.02 & 0.00
% \\ 
%   &SCAn~\cite{tang2021demon} 
% & \multicolumn{1}{c}{0.00} & 0.00 & 0.00 
% & \multicolumn{1}{c}{0.00} & 0.00 & 0.00  
% & \multicolumn{1}{c}{0.00} & 0.00 & 0.00  
% & \multicolumn{1}{c}{0.99} & 0.00 & 0.96
% & \multicolumn{1}{c}{0.99} & 0.00 & 1.00  
% \\ 
%   &Spectral~\cite{tran2018spectral}  
% & \multicolumn{1}{c}{0.00} & 0.15 & 0.00 
% & \multicolumn{1}{c}{0.70} & 0.00 & 0.14 
% & \multicolumn{1}{c}{0.40} & 0.15 & 0.00  
% & \multicolumn{1}{c}{0.80} & 0.15 & 0.01  
% & \multicolumn{1}{c}{0.00} & 0.15 & 0.00
% \\ 
%   &STRIP~\cite{gao2019strip}    
% & \multicolumn{1}{c}{0.25} & 0.16 & 0.00 
% & \multicolumn{1}{c}{0.40} & 0.13 & 0.00 
% & \multicolumn{1}{c}{0.62} & 0.16 & 0.00  
% & \multicolumn{1}{c}{0.78} & 0.16 & 0.01  
% & \multicolumn{1}{c}{0.96} & 0.18 & 0.10
\multirow{4}{*}{Tiny ImageNet}  &AC~\cite{chen2018detecting}     
& \multicolumn{1}{c}{0.00} & 1.07 & 0.00
& \multicolumn{1}{c}{0.00} & 0.68 & 0.00
& \multicolumn{1}{c}{0.00} & 0.58 & 0.00
& \multicolumn{1}{c}{0.00} & 0.67 & 0.00
& \multicolumn{1}{c}{0.00} & 1.60 & 0.00
\\ 
  &SCAn~\cite{tang2021demon} 
& \multicolumn{1}{c}{0.00} & 0.00 & 0.00 
& \multicolumn{1}{c}{0.00} & 0.00 & 0.00  
& \multicolumn{1}{c}{0.00} & 0.00 & 0.00  
& \multicolumn{1}{c}{0.00} & 0.00 & 0.00  
% & \multicolumn{1}{c}{99.00} & 0.00 & 95.65
& \multicolumn{1}{c}{99.90} & 0.00 & 99.50  
% \\ 
%   &Spectral~\cite{tran2018spectral}  
% & \multicolumn{1}{c}{0.00} & 15.00 & 0.00 
% & \multicolumn{1}{c}{90.00} & 14.99 & 0.12 
% & \multicolumn{1}{c}{40.00} & 15.00 & 0.26  
% & \multicolumn{1}{c}{80.00} & 14.95 & 1.05  
% & \multicolumn{1}{c}{0.00} & 15.22 & 0.00
\\ 
  &STRIP~\cite{gao2019strip}    
& \multicolumn{1}{c}{25.00} & 15.67 & 0.01 
& \multicolumn{1}{c}{40.00} & 13.03 & 0.06 
& \multicolumn{1}{c}{62.00} & 16.16 & 0.38  
& \multicolumn{1}{c}{78.00} & 15.91 & 0.96  
& \multicolumn{1}{c}{95.70} & 18.41 & 9.32
\\
\bottomrule
\end{tabular}
}}
\end{table*}

\begin{figure}[htbp]
\centering
\includegraphics[width=8.85cm,height=2.9cm]
% {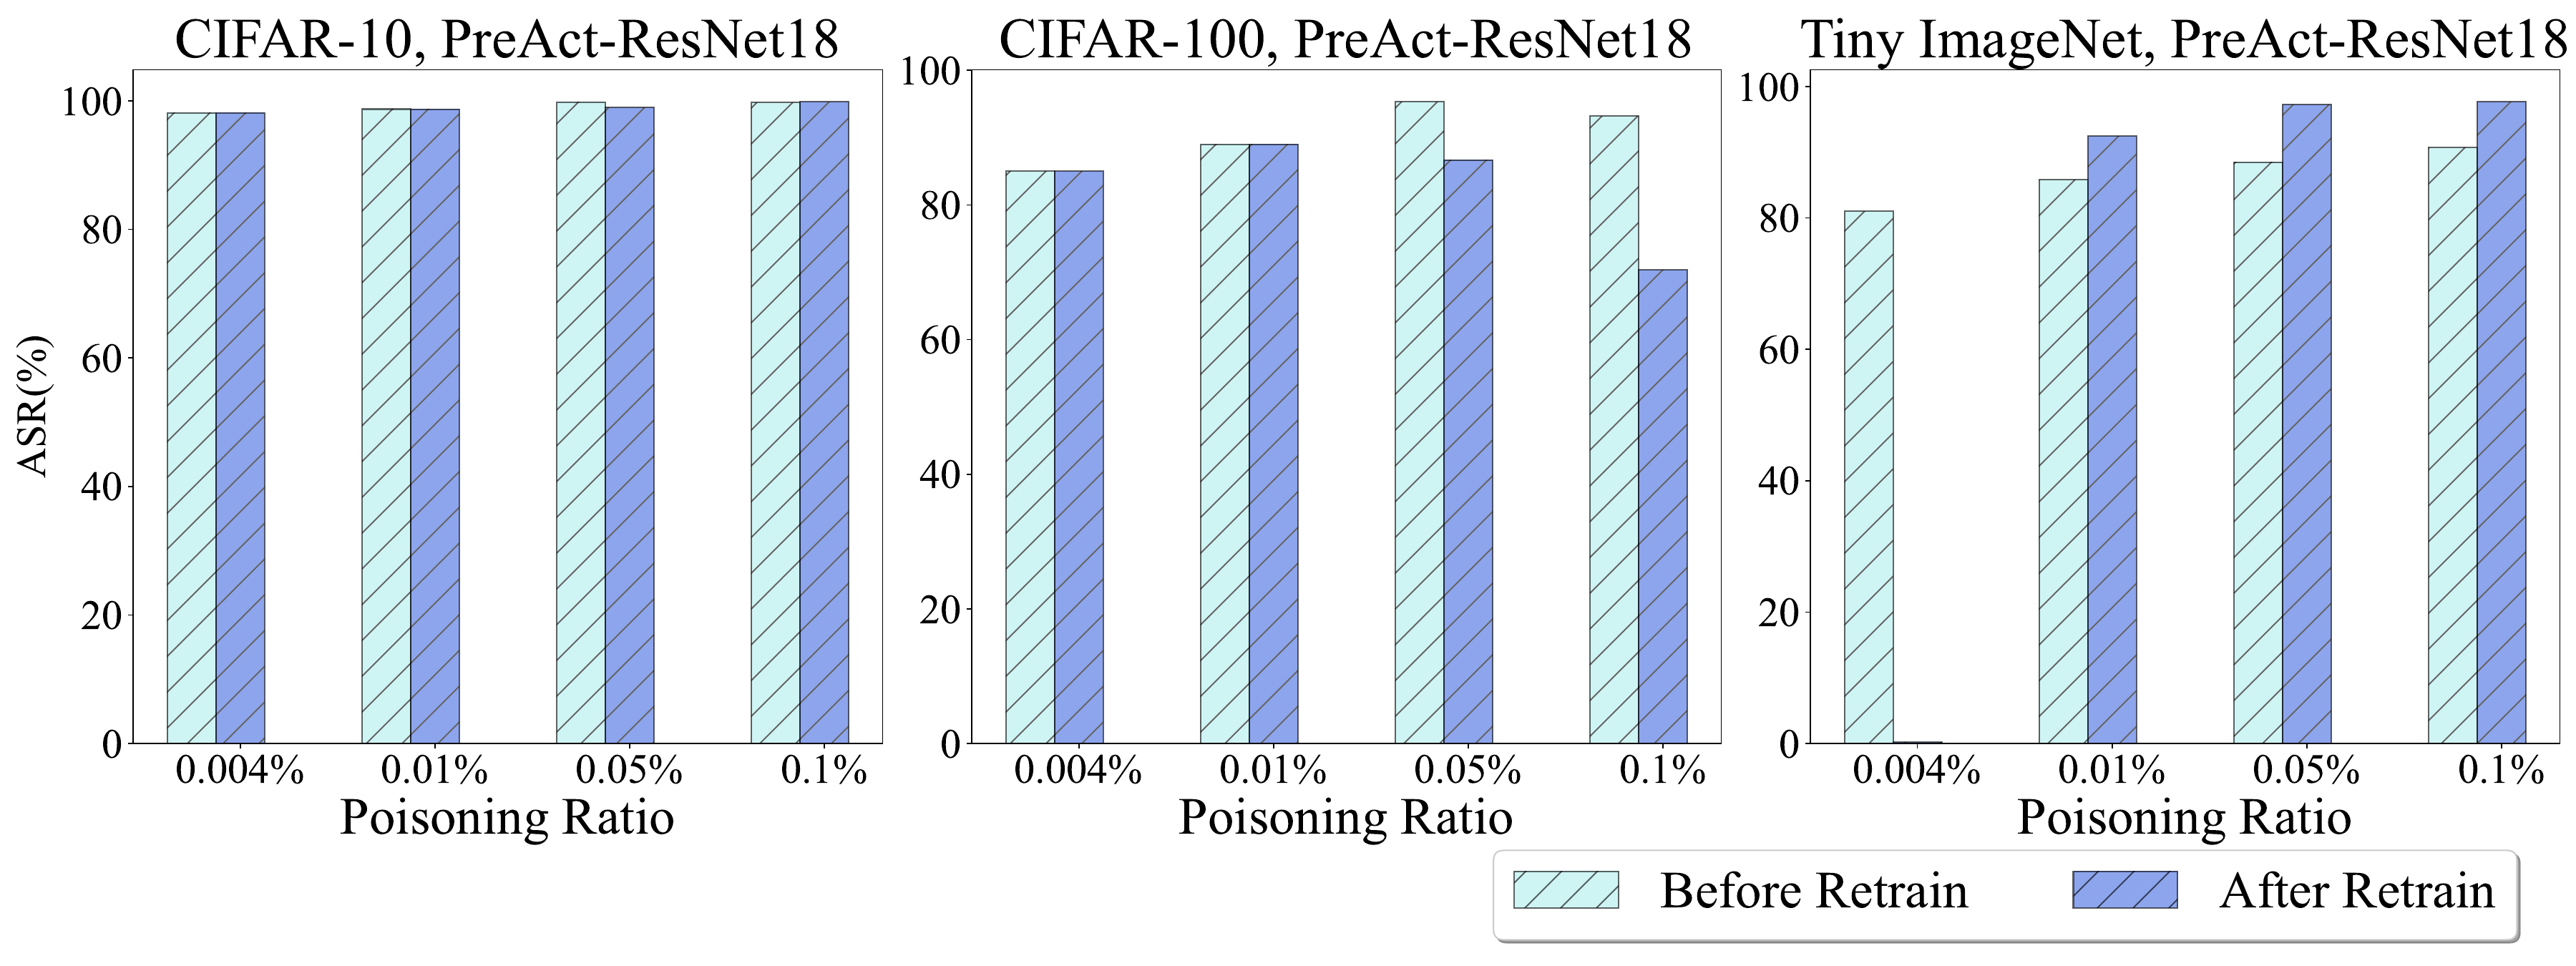}
{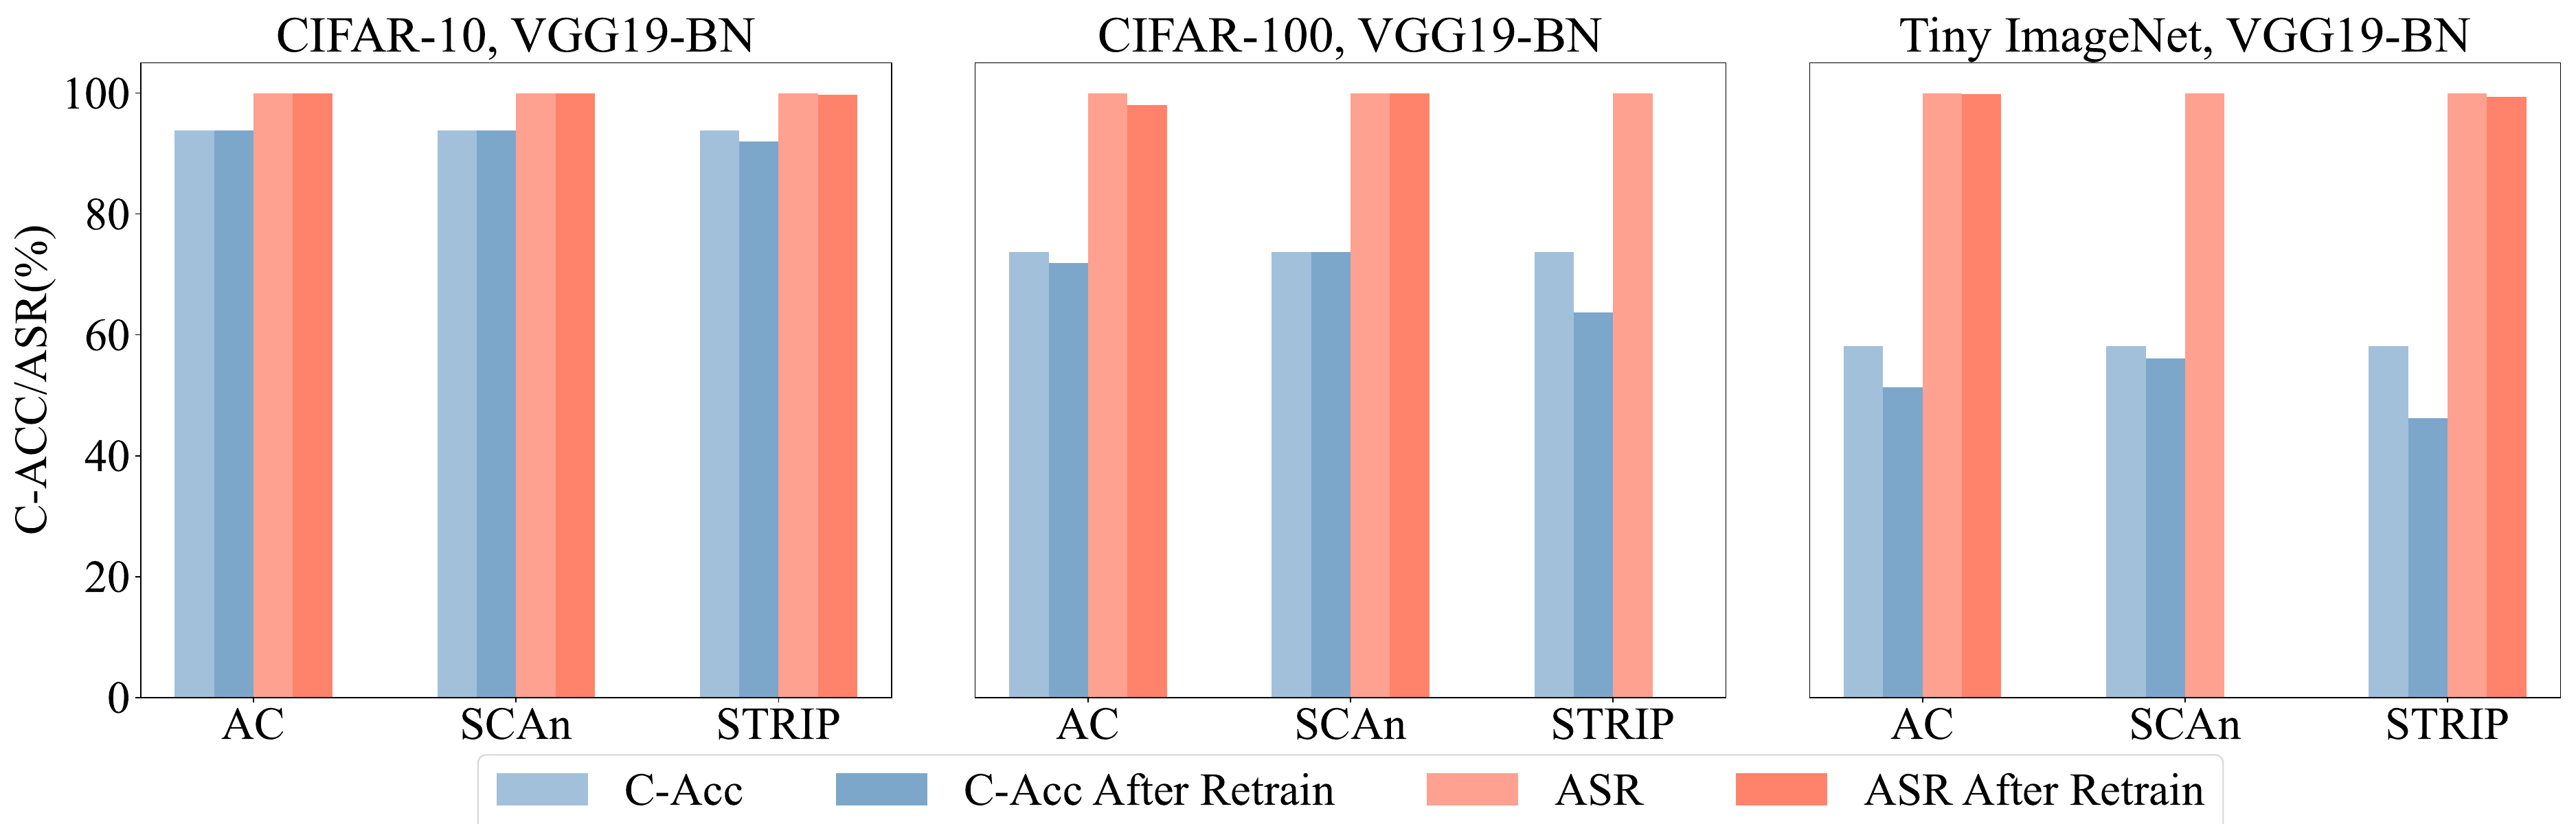}
\caption{Results of retraining after removing suspicious samples using detection methods at 1\% poisoning ratio on PreAct-ResNet18.}
\label{STRIP detection pre}
\vspace{-0.5cm}
\end{figure}

\begin{figure}[!ht]
\centering  %图片全局居中
% \vspace{-5.2cm}
    \subfigure[CIFAR-10]{
    \includegraphics[width=3.45in]
    {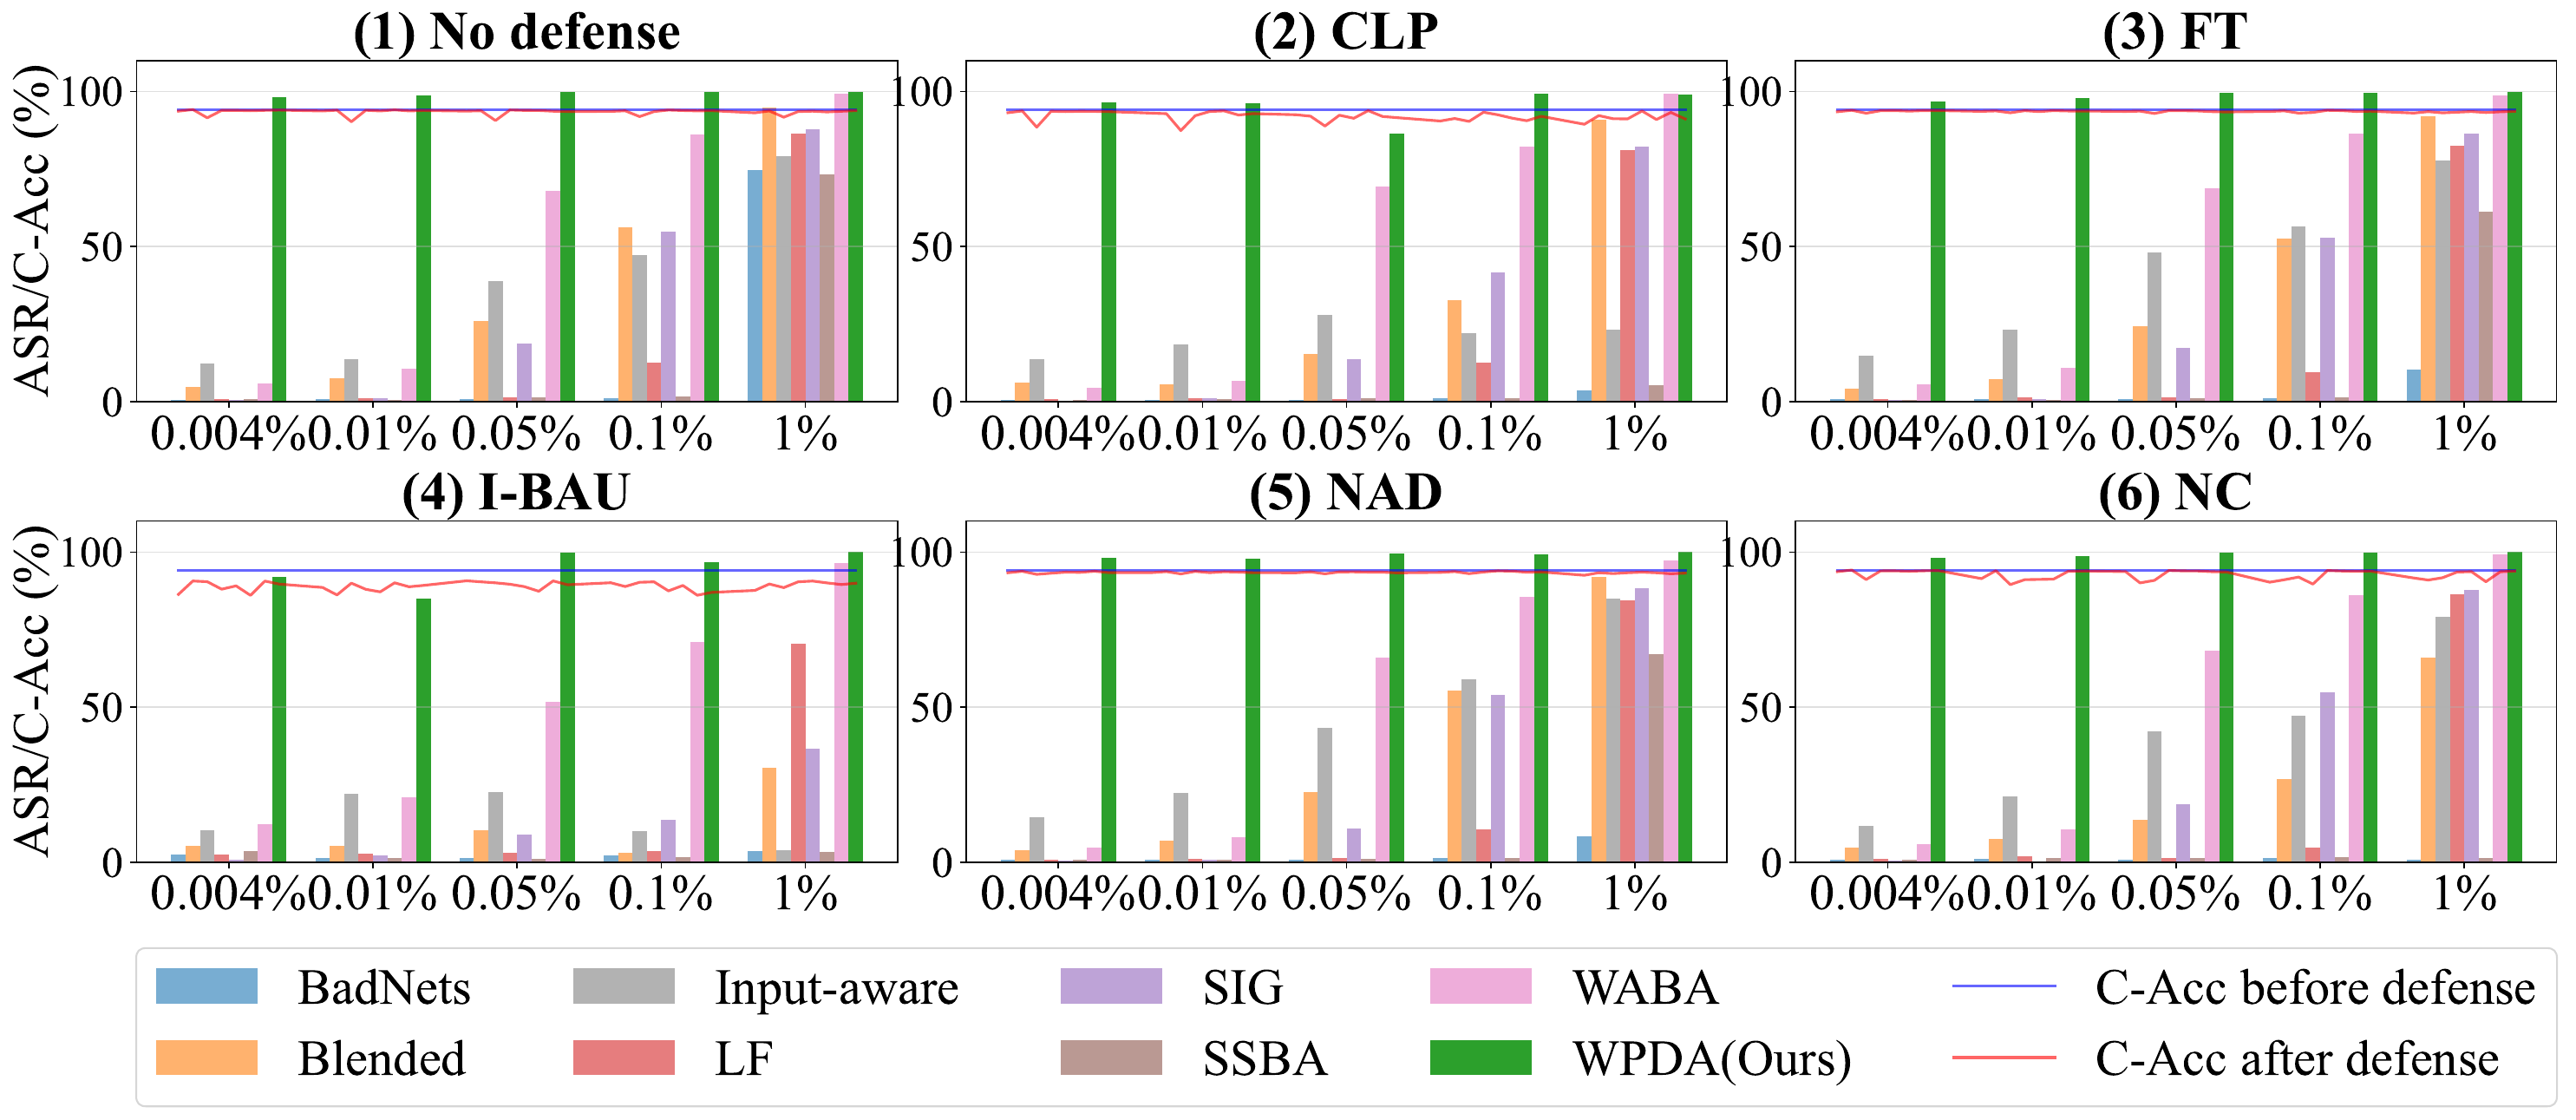}
    % {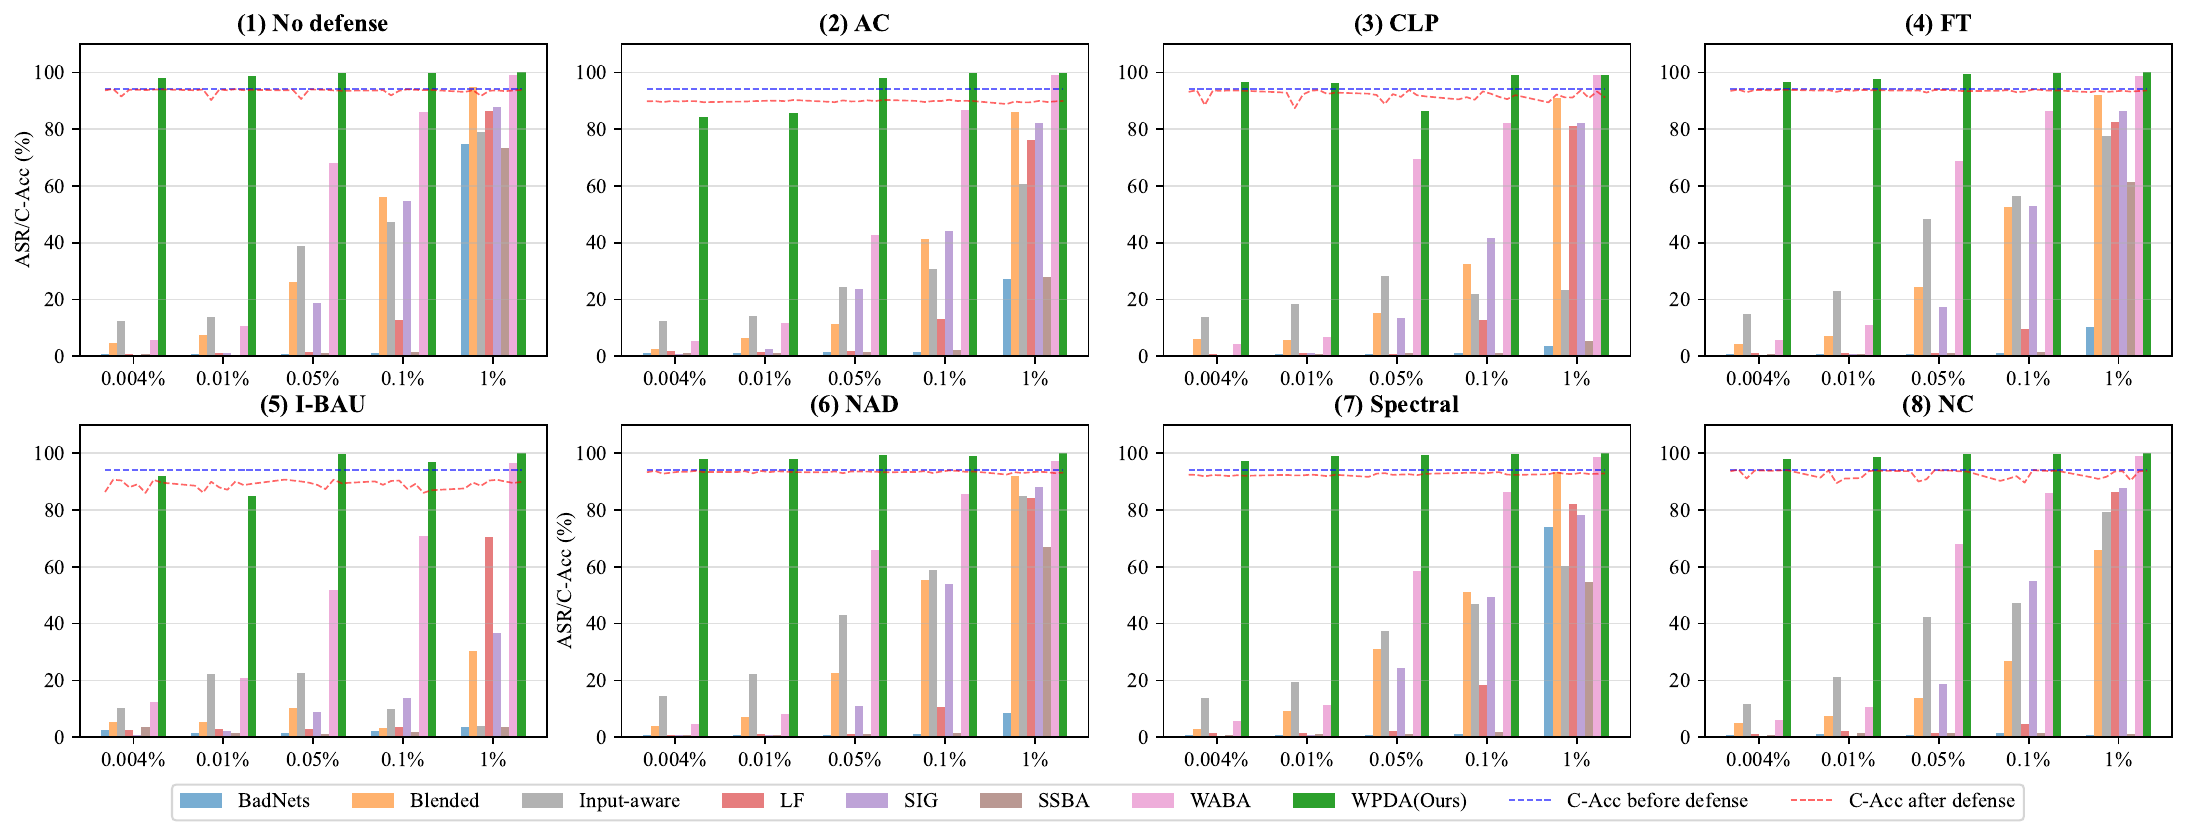}
    }
    \label{CIFAR-10_pre_defense}
    \subfigure[CIFAR-100]{
    \includegraphics[width=3.45in]
    {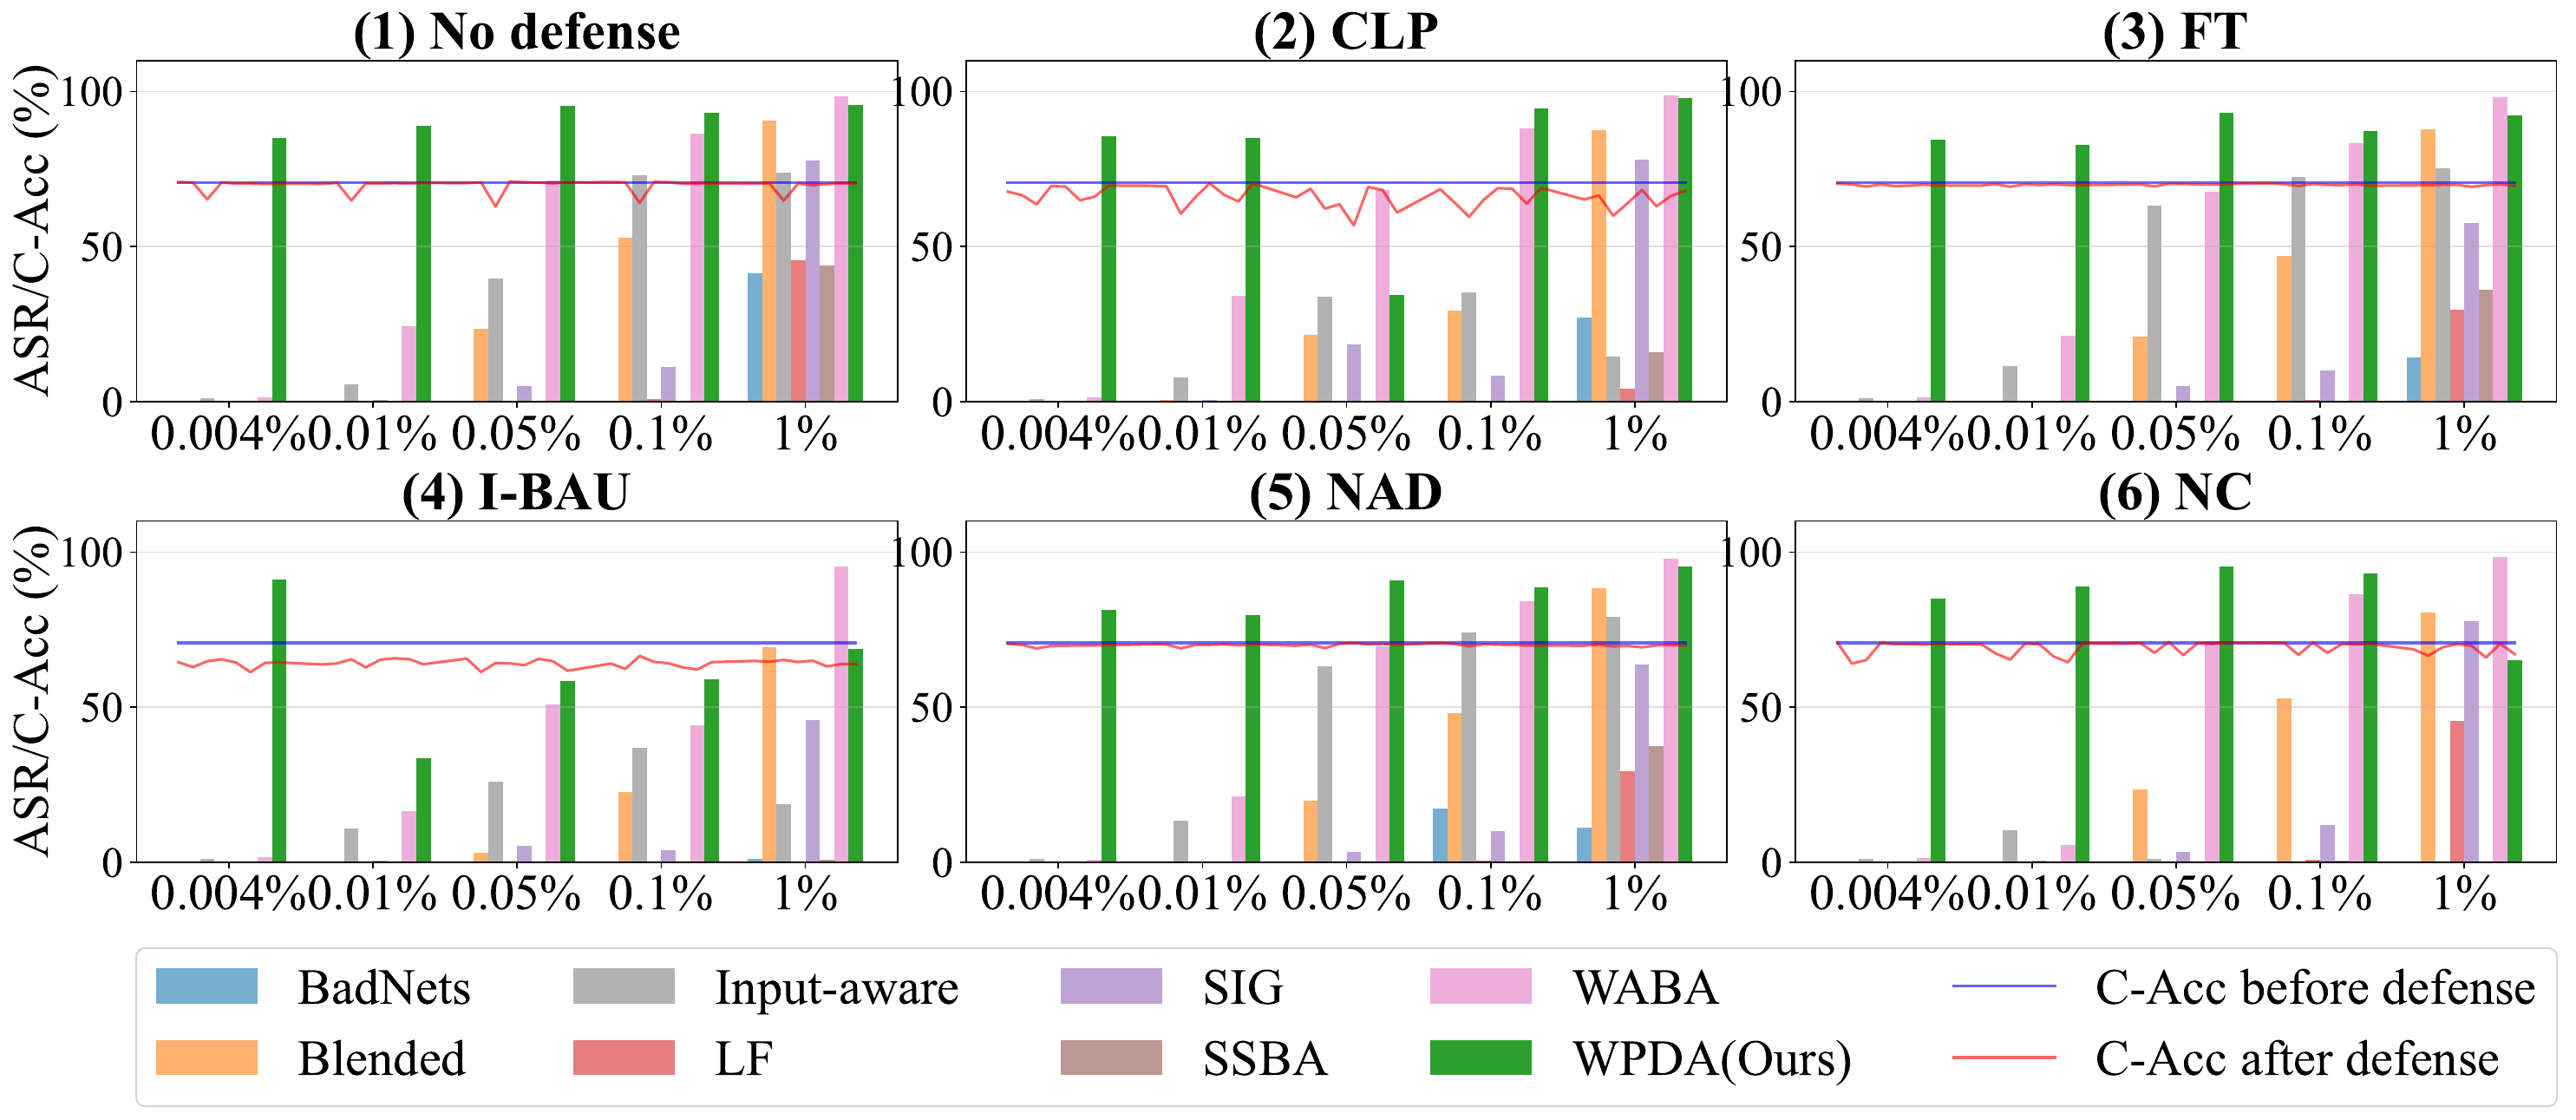}
    % {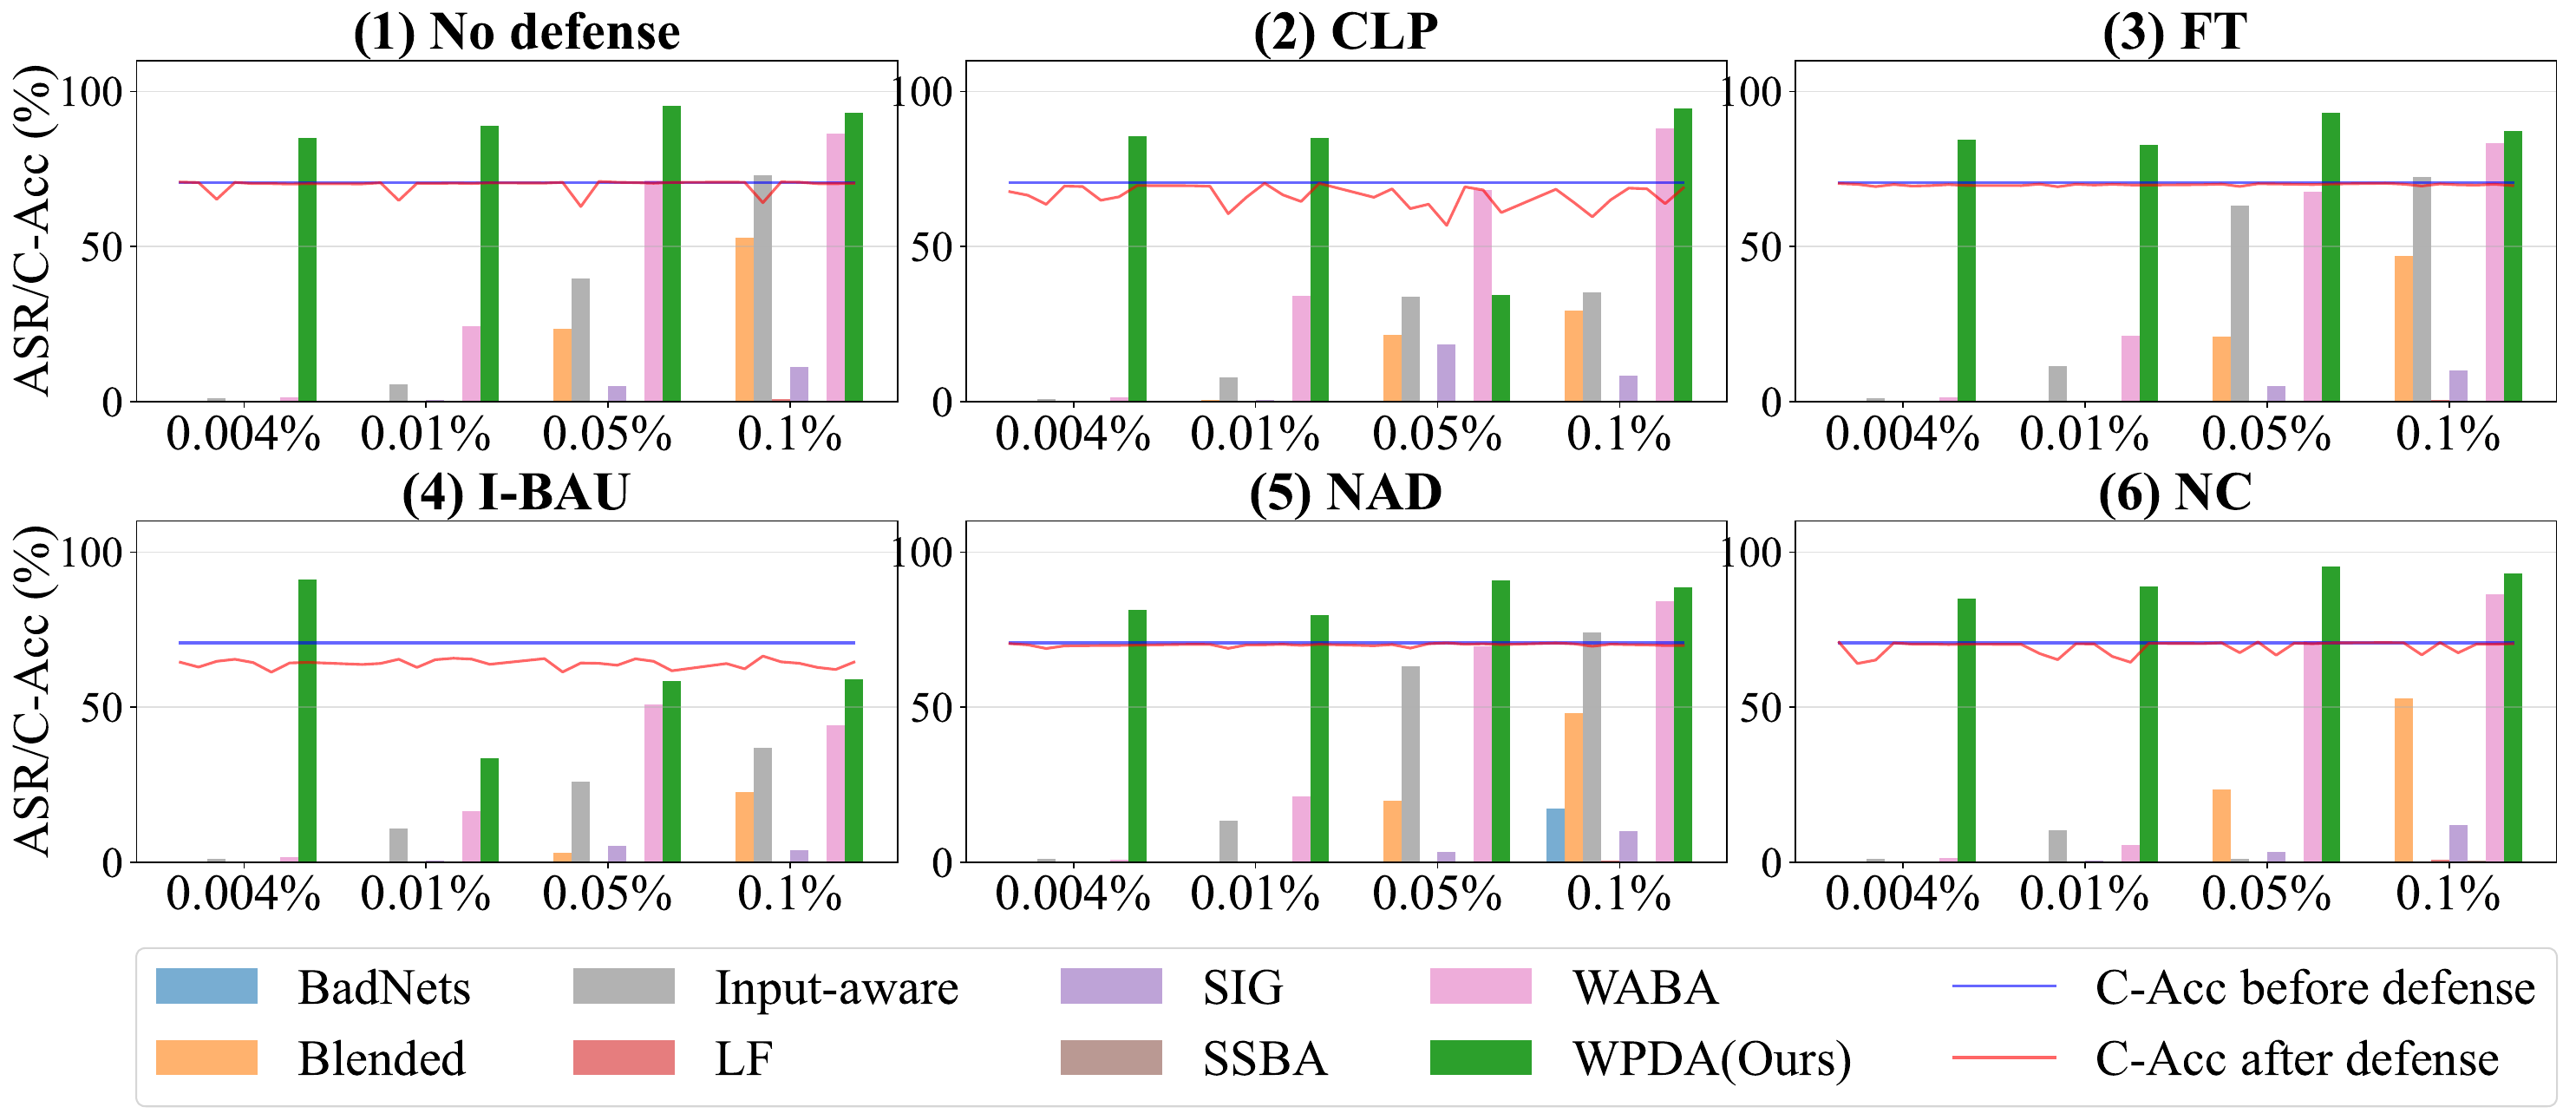}
    }
    \label{CIFAR-100_pre_defense}
    \subfigure[Tiny ImageNet]{
    \includegraphics[width=3.45in]
    {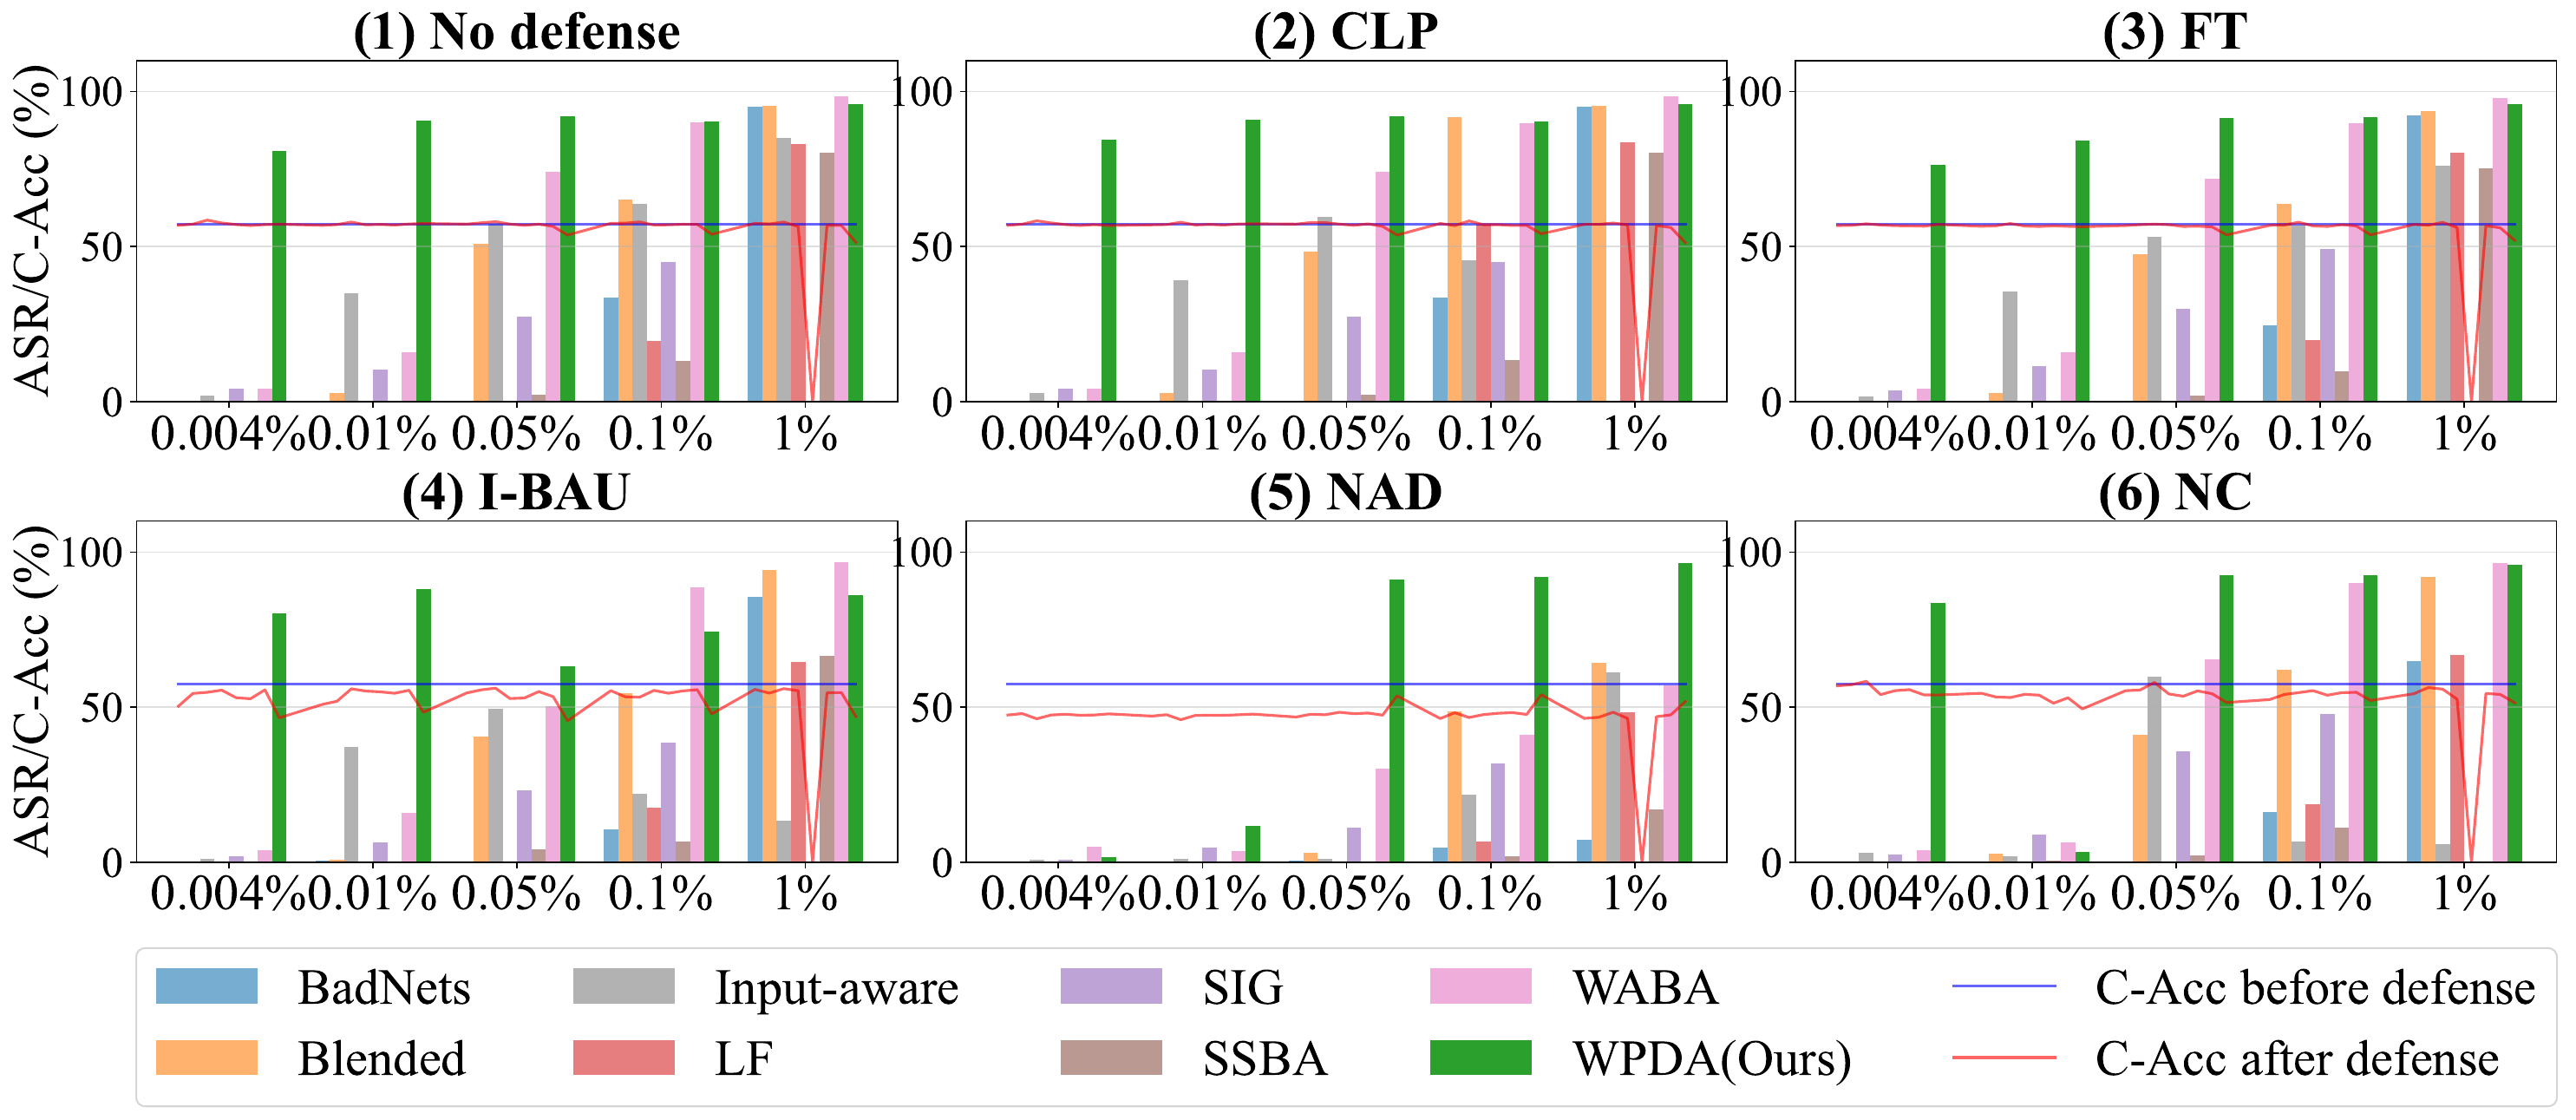}
    % {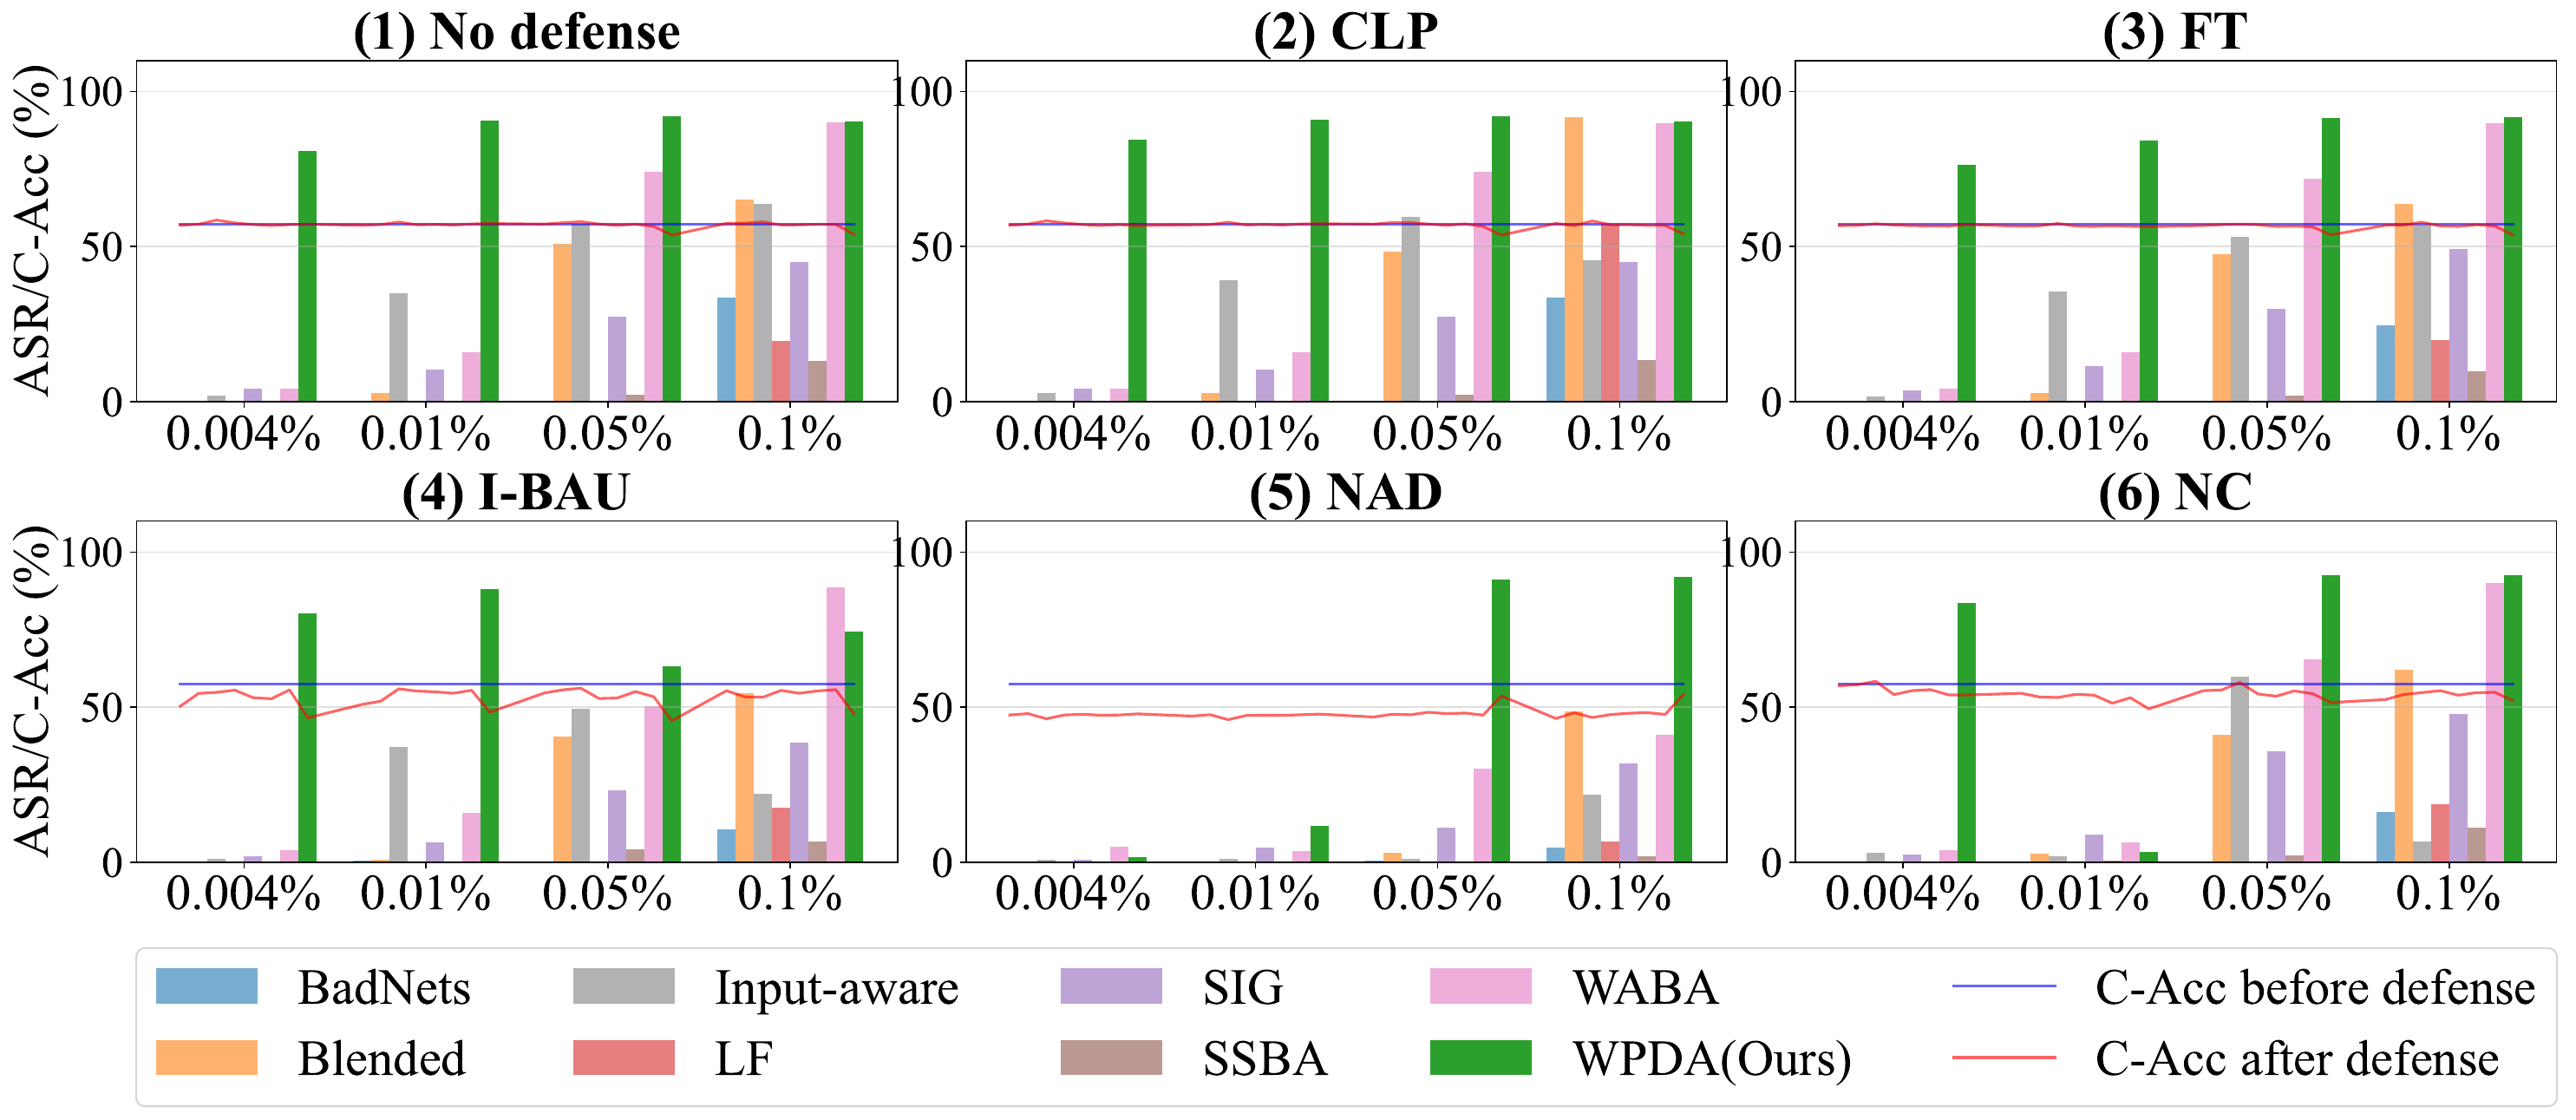}
    }
    \label{tiny_pre_defense}
\caption{Results of 7 compared attack methods and WPDA against 5 defense methods on PreAct-ResNet18, including CLP, FT, I-BAU, NAD and NC. Each sub-plot corresponds to one defense method. In each sub-plot, each bar in the histogram indicates the ASR value of one attack method, and the C-Acc values are represented by curves.}
\vspace{-0.5cm}
\label{all-defense-pre}
\end{figure}
\subsection{\textbf{Defense Performance of WPDA on PreAct-ResNet18}
\label{defense on pre}}
In Fig.~\ref{all-defense-pre}, we evaluate the resistance performance of WPDA and other attacks under 5 SOTA backdoor defense methods on PreAct-ResNet18. 
\paragraph{\textbf{Evaluations On CIFAR-10}} At low poisoning ratios, due to 7 compared attack methods fail to achieve successful backdoor attacks, their resistance are difficult to be evaluated. As poisoning ratios increases, although ASRs of attack methods improve, some compared attack methods perform weak resistance, such as Blended, Input-aware and SIG after CLP and I-BAU at 0.1\% poisoning ratio, BadNets after 5 defenses at 1\% poisoning ratio. While WPDA demonstrates superior resistance at all 5 poisoning ratios. 
\paragraph{\textbf{Evaluations On CIFAR-100}} Most methods with lower poisoning ratios exhibit more resistant performance after defense compared to those with higher poisoning ratios. For instance, after CLP, the ASR degradation observed in Blended and Input-aware methods is demonstrably more pronounced at a poisoning ratio of 0.1\% relative to 0.05\%. Similarly, the decrease in ASR for WPDA at 0.05\% poisoning ratio is higher than that at 0.01\% poisoning ratio. This phenomenon is also evident after I-BAU. WPDA performs strong resistance, particularly at 0.004\% poisoning ratio, with its effectiveness remaining unaffected after undergoing five defenses.

\paragraph{\textbf{Evaluations On Tiny ImageNet}} After CLP and FT, WPDA continues to outperform all compared attack methods across all poisoning ratios. After I-BAU, although there is a certain degree of decline in WPDA's ASR, it still remains effective, particularly the WPDA at low poisoning ratios, exhibiting more resistant performance to defense compared to high poisoning ratios. After NAD, the effectiveness of all attack methods at poisoning ratios of 0.004\% and 0.01\% is significantly impacted, only WPDA still exhibits residual efficay at 0.01\% poisoning ratio. However, the C-Acc of the model is seriously impacted, indicating that NAD fails to resist the attacks. After NC, 
WPDA demonstrates most resistant than other attack methods at poisoning ratios of 0.004\%, 0.05\%, 0.1\%, and 1\%. At  0.01\%, there is a significant decrease in C-Acc for WPDA, indicating that Nc is unable to resist WPDA.
\paragraph{\textbf{Summary}} The above results illustrate that WPDA exhibits strong resistance across 3 datasets and 2 models, particularly the WPDA at low poisoning ratios, which presents significant challenges to defenses.
