# Supplementary material for: WPDA: Frequency-based Backdoor Attack with Wavelet Packet Decomposition
Source: arXiv:2401.13578 source file (2024-12-01)
Supplement: Supplementary file 3 [file 7_appendix_new.tex]

% \twocolumn[\section*{Appendix}]
% \newpage
\section{Appendix}
% \appendix
\label{appendix}
% \section*{Appendix}
\subsection{\textbf{Verification}: Using the absolute average algorithm could potentially reduce sensitivity to noise compared to using the average absolute algorithm.
\label{explain why it is important to take the average value before taking the absolute value}
}
\noindent\textbf{1. Understanding Noise and Its Impact:}
In image processing and signal analysis, noise refers to unwanted variations or disturbances that corrupt the original signal. Noise can arise from various sources, such as sensor limitations, transmission errors, or environmental factors. When applying wavelet packet decomposition to an image, noise can manifest as small fluctuations in the coefficient values within each sub-spectrogram. These fluctuations might not necessarily represent meaningful information but rather random disturbances.The design of effectiveness metric $E$ influences how sensitive the selection of key frequency regions is to these noise-induced fluctuations.\\
\textbf{2. Absolute average algorithm \textit{vs} Average absolute algorithm and Noise Reduction:}
Before calculating the absolute values, computing the average of the coefficient matrix can reduce the impact of noise-induced fluctuations on the overall average. For example, considering a sub-spectrogram with a coefficient matrix like [-3, +4, -2, +5], the absolute average value of the coefficient matrix is +1. However, if noise causes small fluctuations, the coefficient matrix might become [-3.1, +3.9, -1.9, +4.2]. The average value of the coefficient matrix now changes to 1.025, even though the overall information content has not significantly changed.
Using the average absolute algorithm, the average absolute value of the coefficient matrix is +3.5, while the average absolute value of the coefficient matrix with noise is +3.275, demonstrating a higher sensitivity to the noise-induced fluctuations.\\
\textbf{3. Verification Experiment:}
Using the average absolute algorithm, the key frequency regions are `ah', `hh', `vv', `dd'. We conduct empirical experiments to complete the training and generate backdoor samples in the same way as WPDA. Take CIFAR-10 as an example, Fig.~\ref{abs mean} demonstrates that poisoned samples generated by the average absolute algorithm are less effective than those produced by absolute average algorithm. 
\begin{figure}[H]
\centering  %图片全局居中
    {
    \includegraphics[width=1.60in]{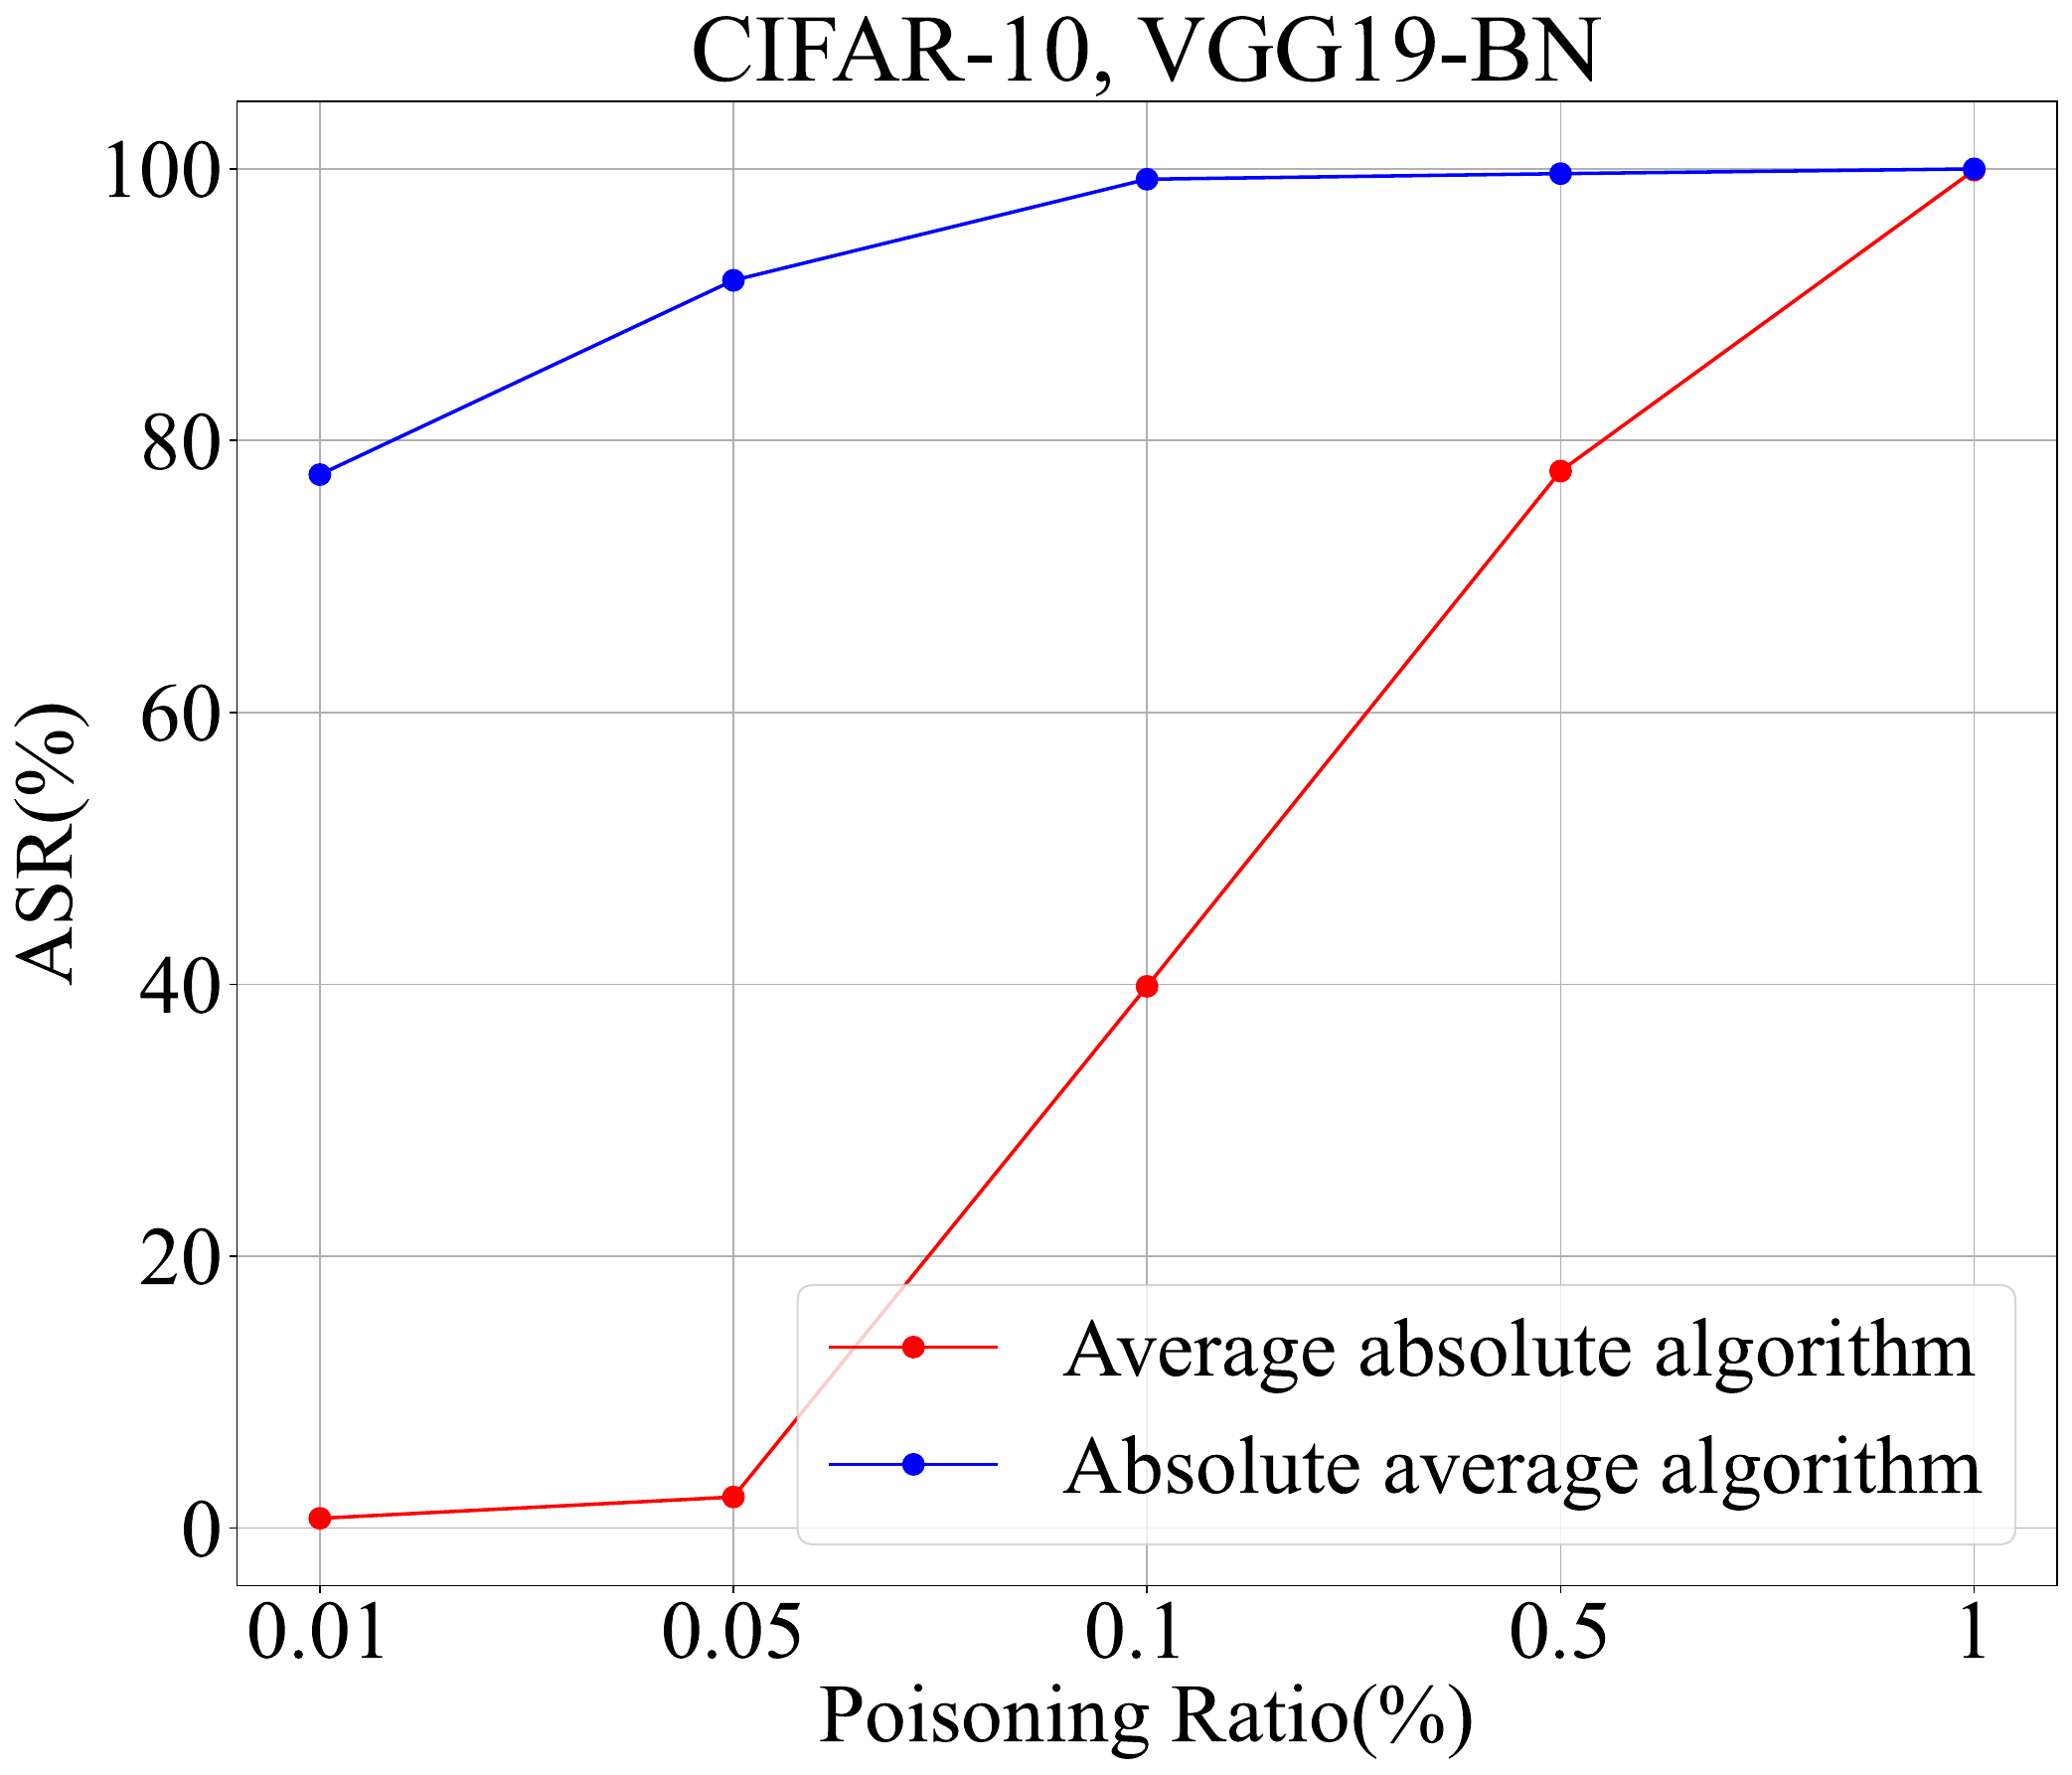}}
    \label{vgg19bn_abs_mean}
    {
    \includegraphics[width=1.60in]{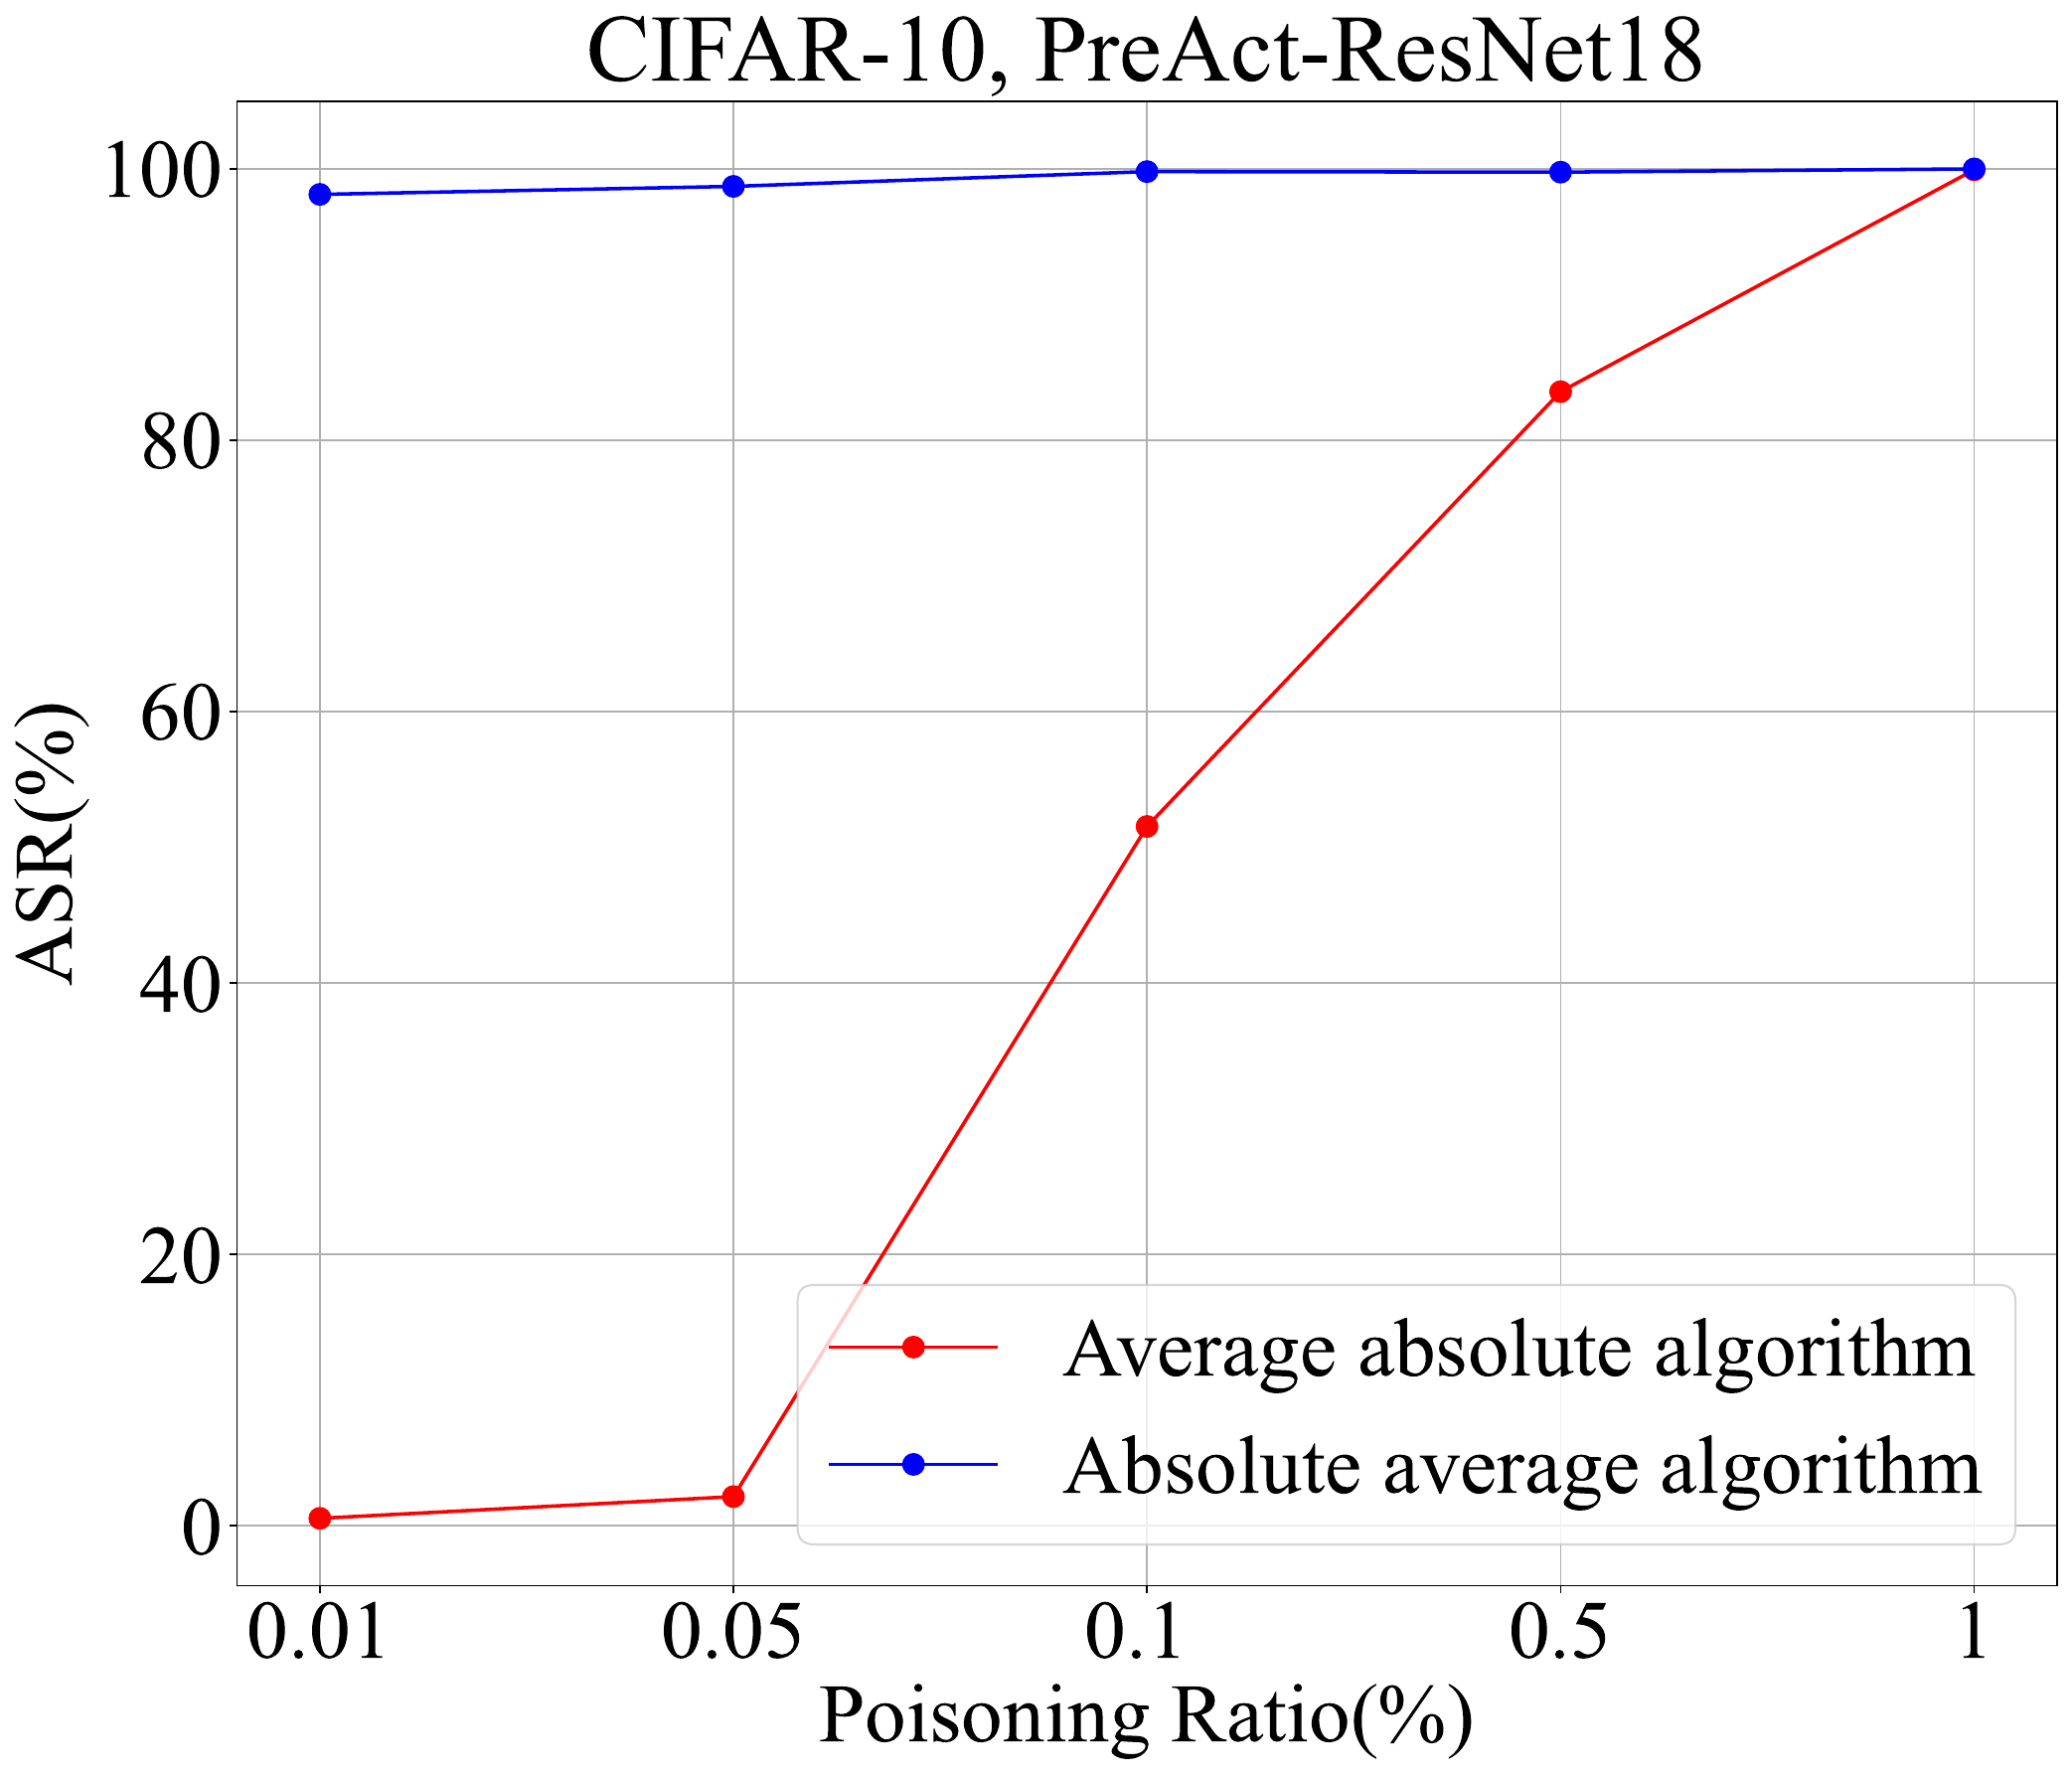}}
    \label{preactresnet18_abs_mean}
\caption{Performance of absolute average algorithm and average absolute algorithm.}
\label{abs mean}
\vspace{-0.7cm}
\end{figure}
\noindent\textbf{4. Combining Evidence and Reasoning:}
By combining theoretical reasoning and empirical evidence, we can infer that absolute average algorithm can effectively reduce the effect of noise on the samples and help us accurately select key frequency regions.

\subsection{\textbf{Verification}:
\label{original information have negative effect on the backdoor activation}
The original benign sample information compete with the trigger information for the model’s attention, making it harder for the model to learn the association between the trigger and the target label. 
}
We conduct empirical experiments to complete the training process while preserving the original benign sample information and to generate poisoned testing samples in the same way as WPDA. Take CIFAR-10 as an example, Fig.~\ref{effect of original_information} describes that the ASR of  preserving the original benign sample information in the training process is lower than that of masking the original benign sample information, especially at low poisoning ratios. The results demonstrate a dynamic competition between the original benign sample information and trigger information. As an increased proportion of poisoned training samples,  the influence of the original benign sample information diminishes progressively. Consequently, for achieving effective backdoor attacks at low poisoning ratios, it becomes necessary to mask the original benign sample information in training process.
\begin{figure}[H]
\centering  %图片全局居中
    {
    \includegraphics[width=1.60in]{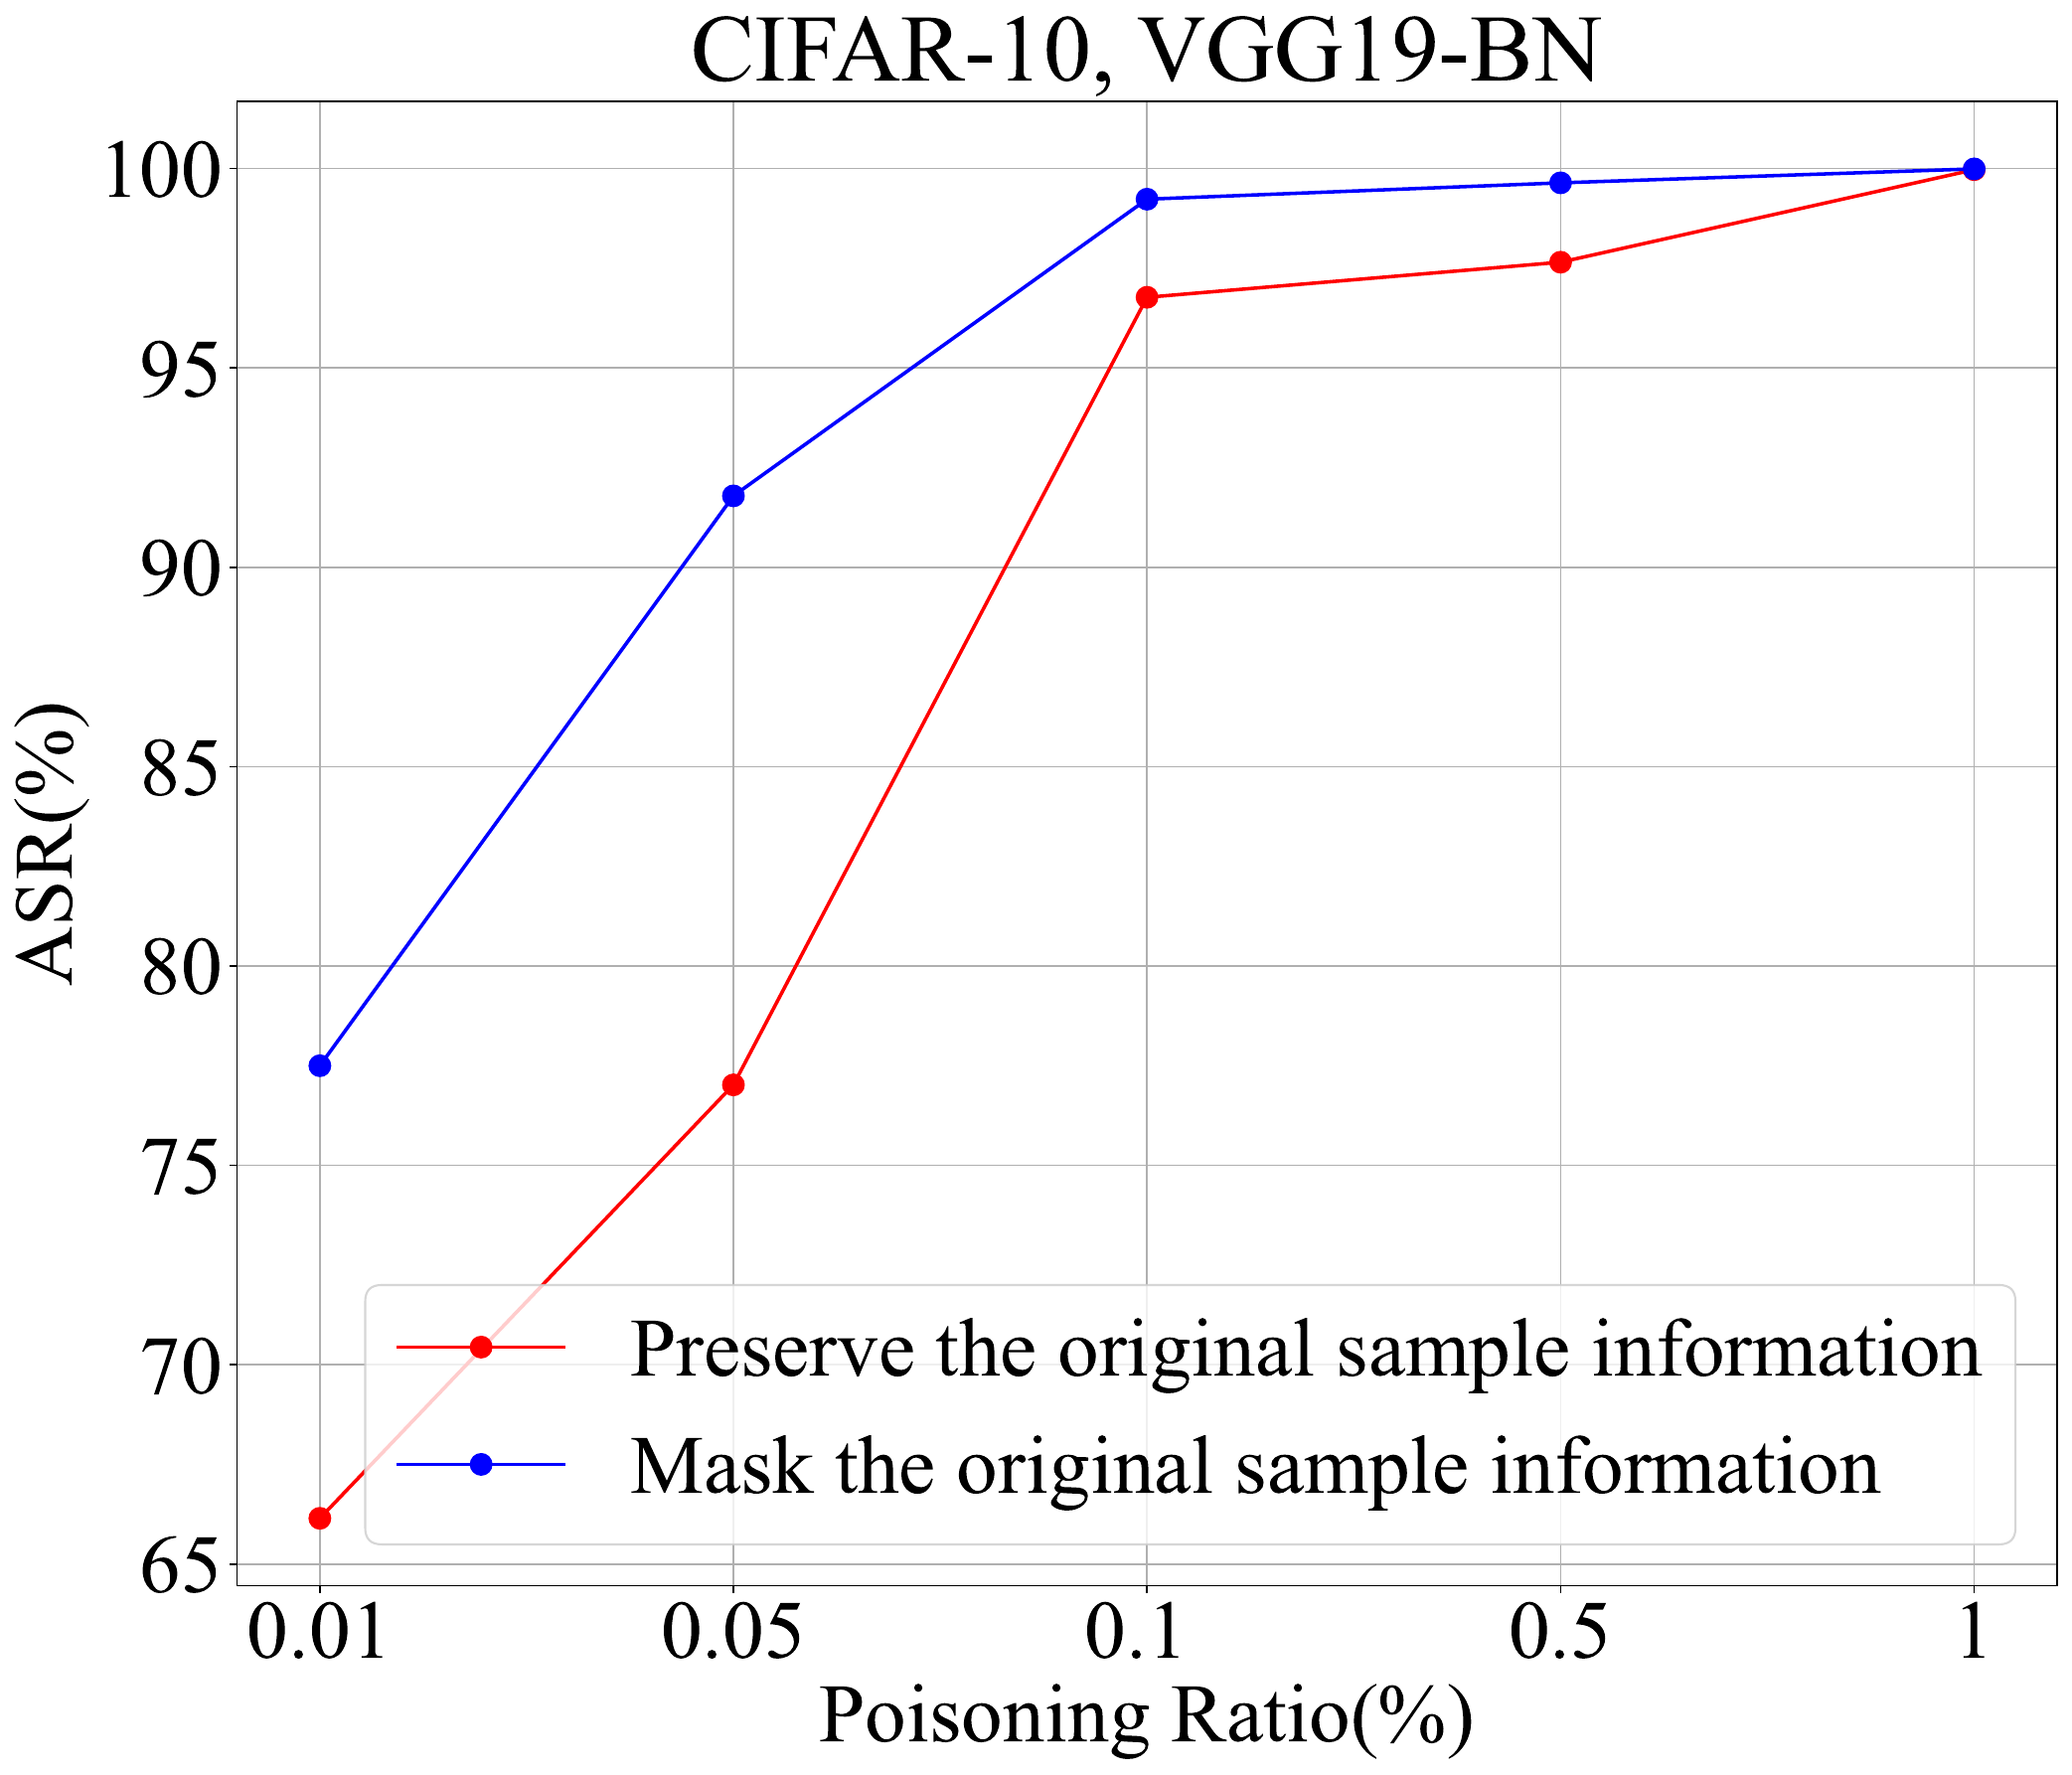}}
    \label{vgg19bn_original_information}
    {
    \includegraphics[width=1.60in]{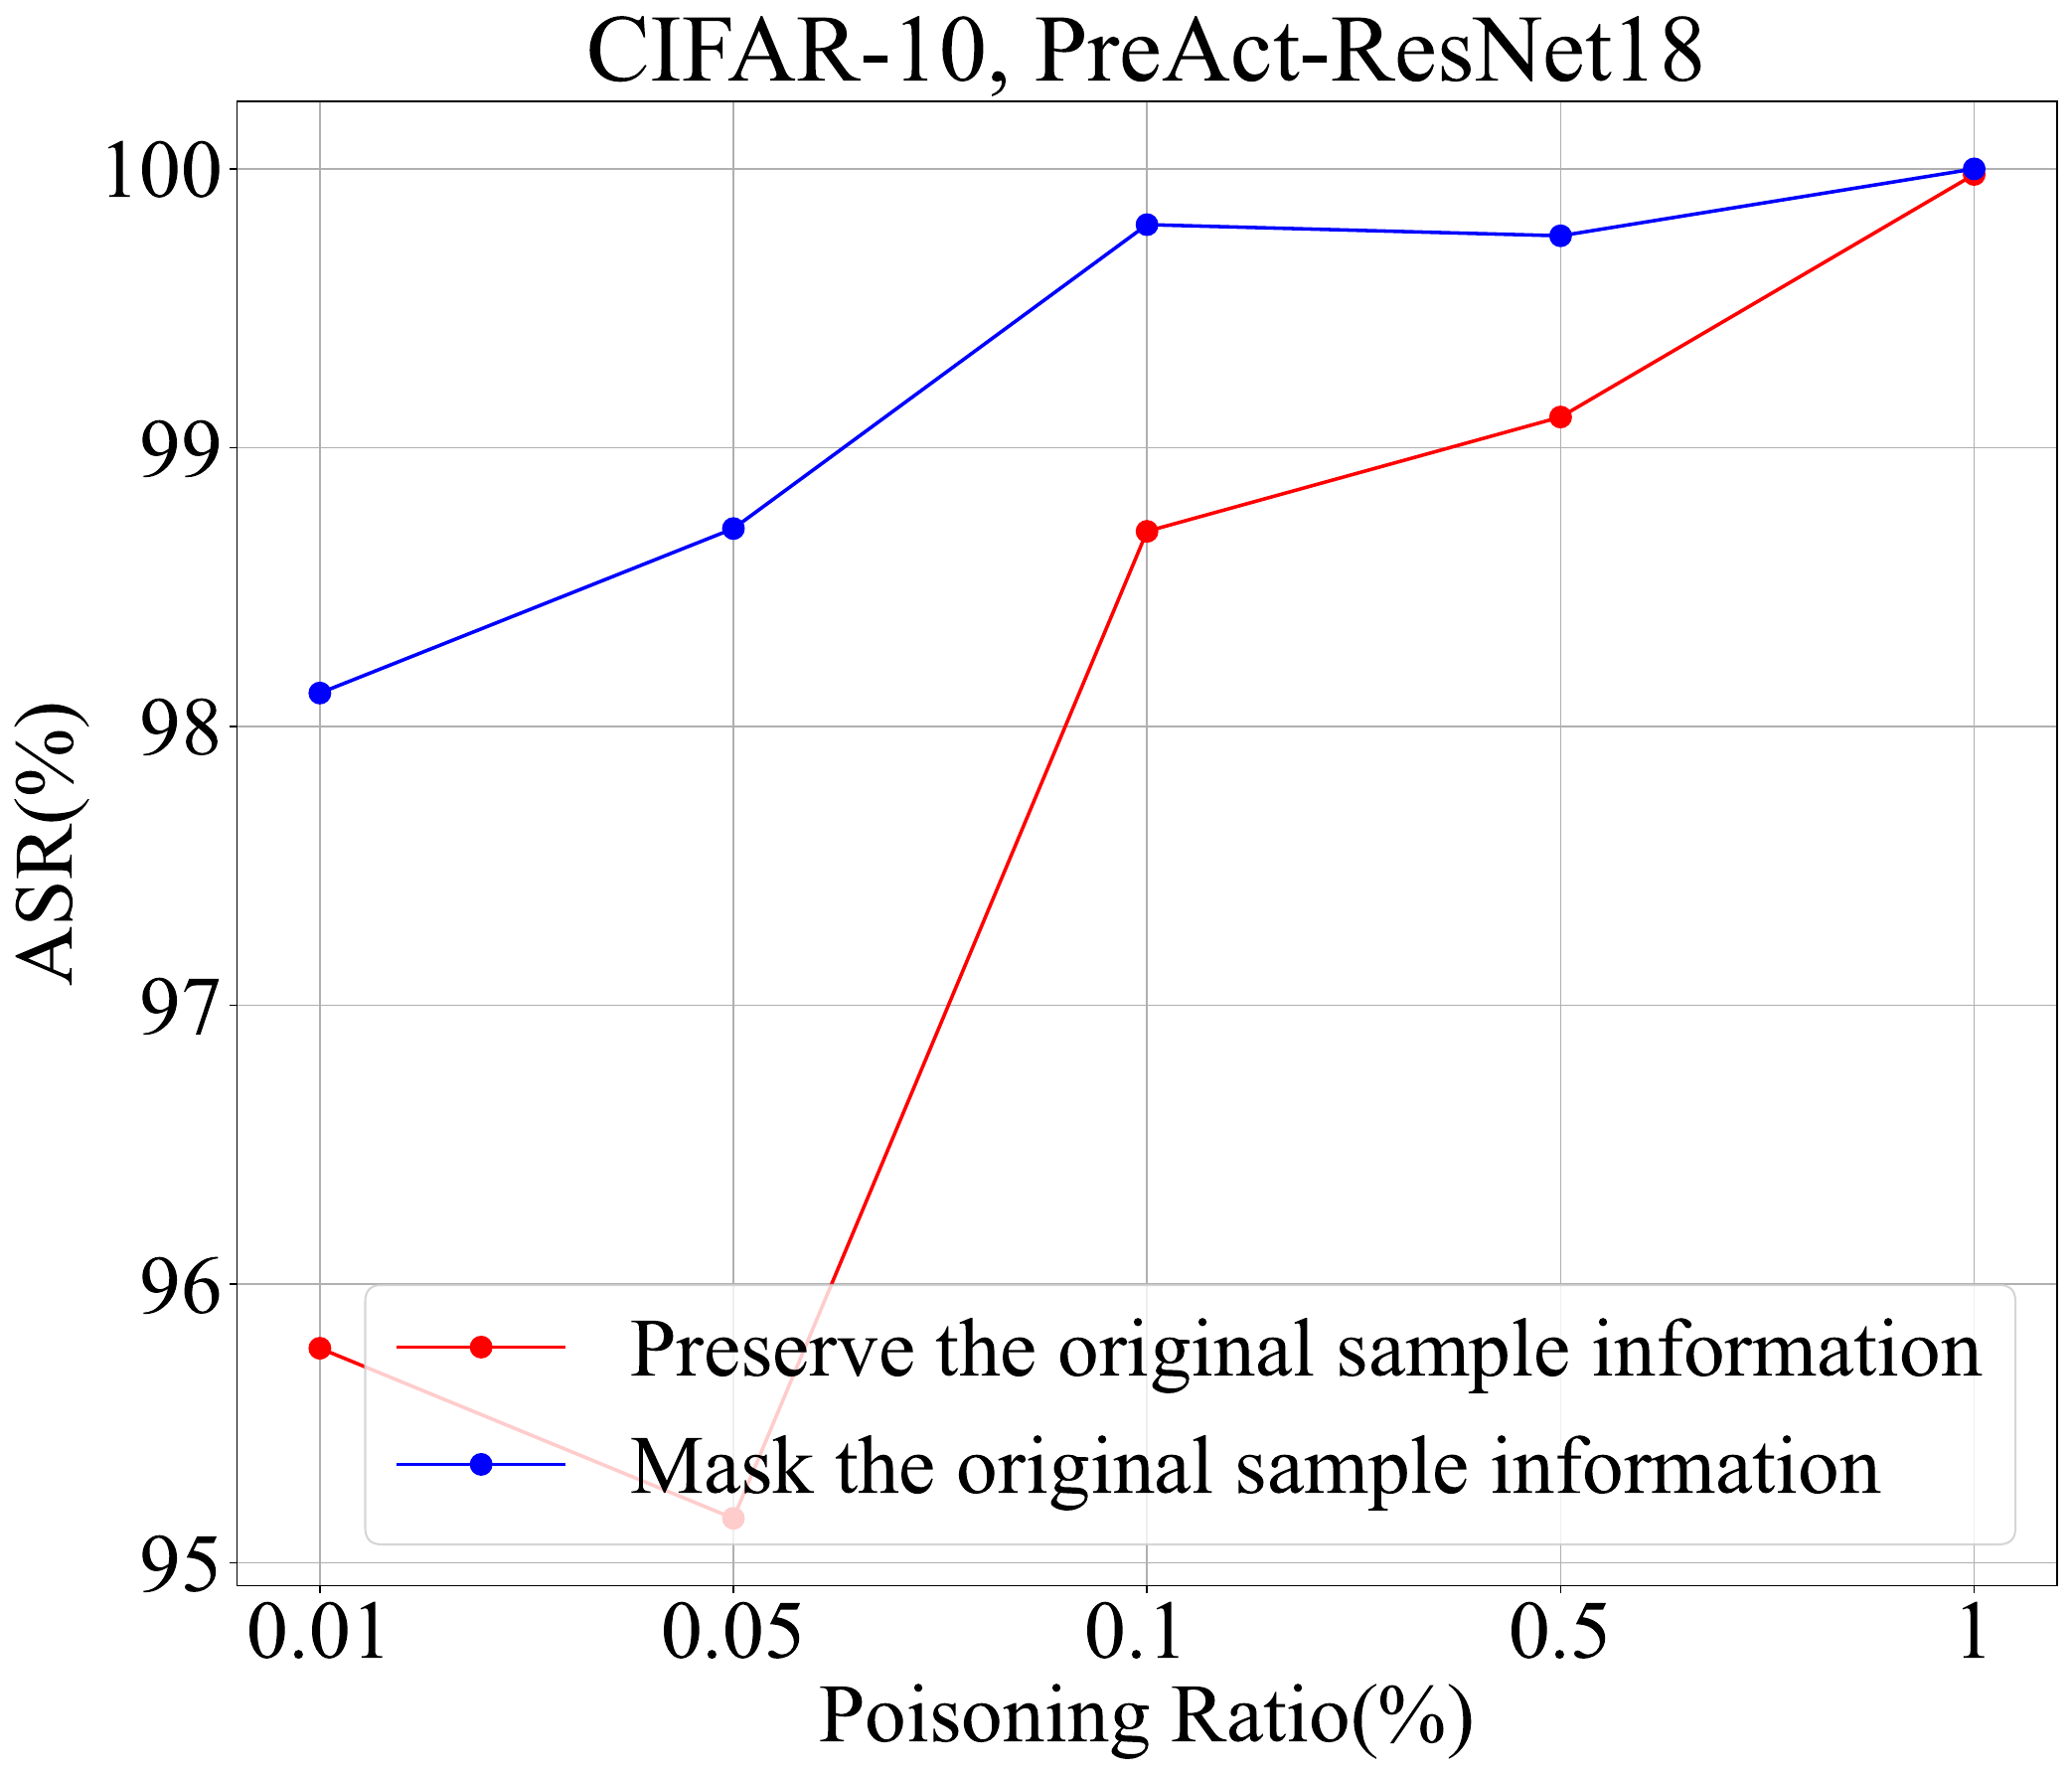}}
    \label{preactresnet18_original_information}
\caption{Effect of original benign sample information in key frequency regions on model learning triggers.}
\label{effect of original_information}
\vspace{-0.5cm}
\end{figure}

\subsection{\textbf{Detection Performance of WPDA on PreAct-ResNet18}:
\label{detection on pre}}
Tab.~\ref{detection_result_pre} indicates that WPDA maintains stability, effectiveness and stealth after AC and SCAn detection methods across all datasets and poisoning ratios. The reported TPR values are 0, indicating that no poisoned training samples are identified as suspicious, \textit{i.e.}, WPDA effectively evades detection by AC and SCAn. For STRIP, the performance varies across datasets due to differences among the datasets. 
\textbf{On CIFAR-10}, STRIP correctly identifies some of the poisoned training data at all poisoning rates, but it also mistakenly classifies some benign training samples as poisoned. In a further analysis shown in Fig.~\ref{STRIP detection pre}, we remove the training samples identified as suspicious by STRIP and retain the model. The results indicate that our attack remains highly effective, with a high ASR. 
\textbf{On CIFAR-100}, At 0.004\% and 0.01\% poisoning ratios, WPDA effectively evades detection by the STRIP method. Furthermore, under these conditions, STRIP exhibits a propensity to misidentify a substantial proportion of benign training samples as poisoned. As the poisoning ratio increases to 0.05\% and above, STRIP successfully detects some of the poisoned training samples. However, after removing all the samples identified as suspicious by STRIP and retraining the models, WPDA still works with a high ASR shown in Fig.~\ref{STRIP detection pre}. 
\textbf{On Tiny ImageNet}, STRIP successfully detects some of the poisoned training samples across different poisoning ratios. Moreover, as the poisoning ratio increases, the accuracy of STRIP in detecting the poisoned training samples also exhibits a corresponding rise in Tab.\ref{detection_result_pre}. In Fig.~\ref{STRIP detection pre}, after removing the suspicious samples and retraining the model, ASR at 0.004\% poisoning ratio decays a lot. However, the reported high FPR 15.67\% indicates a significant misidentification of a large number of benign training samples as poisoned, which means that the accuracy of the model on benign samples could be compromised, so our attack still works. At more than 0.05\% poisoning ratios, our method remains effective after STRIP.
 
\begin{table*}[!ht]
\caption{The result of WPDA against 3 detection methods under 5 different poisoning ratios in the datasets. The training model adopts PreAct-ResNet18. }
\label{detection_result_pre}
\centering
% \small
% \large
\normalsize
\scalebox{0.82}{
\resizebox{\textwidth}{!}{
    \begin{tabular}{m{.11\textwidth} m{.1\textwidth} m{.0355\textwidth}<{\centering} m{.0355\textwidth}<{\centering} m{.0355\textwidth}<{\centering} m{.0355\textwidth}<{\centering} m{.0355\textwidth}<{\centering} m{.0355\textwidth}<{\centering} m{.0355\textwidth}<{\centering} m{.0355\textwidth}<{\centering} m{.0355\textwidth}<{\centering} m{.0355\textwidth}<{\centering} m{.0355\textwidth}<{\centering} m{.0355\textwidth}<{\centering} m{.0355\textwidth}<{\centering} m{.0355\textwidth}<{\centering} m{.0355\textwidth}<{\centering} m{.0355\textwidth}<{\centering} m{.0355\textwidth}<{\centering} m{.0355\textwidth}<{\centering}} %{l l cc cc cc cc cc cc cc cc cc}
    \toprule
  \multirow{2}{*}{Dataset} & Poisoning ratio $\rightarrow$ & \multicolumn{3}{c}{0.004\%}        & \multicolumn{3}{c}{0.01\%}        & \multicolumn{3}{c}{0.05\%}        & \multicolumn{3}{c}{0.1\%}        & \multicolumn{3}{c}{1\%} 
\\
\cmidrule(lr){3-5} \cmidrule(lr){6-8} \cmidrule(lr){9-11} \cmidrule(lr){12-14} \cmidrule(lr){15-17} \cmidrule(lr){18-20}
 & Detection $\downarrow$  & \multicolumn{1}{c}{TPR }    & FPR     & $F^{\omega}_1$    & \multicolumn{1}{c}{TPR }    & FPR     & $F^{\omega}_1$    & \multicolumn{1}{c}{TPR }    & FPR     & $F^{\omega}_1$    & \multicolumn{1}{c}{TPR }    & FPR     & $F^{\omega}_1$    & \multicolumn{1}{c}{TPR }    & FPR     & $F^{\omega}_1$       
\\ 
\hline \hline 
\multirow{4}{*}{CIFAR10} & AC~\cite{chen2018detecting}     
& \multicolumn{1}{c}{0.00} & 0.00 & 0.00
& \multicolumn{1}{c}{0.00} & 0.00 & 0.00
& \multicolumn{1}{c}{0.00} & 0.00 & 0.00
& \multicolumn{1}{c}{0.00} & 0.00 & 0.00
& \multicolumn{1}{c}{0.00} & 0.00 & 0.00
\\ 
  & SCAn~\cite{tang2021demon} 
& \multicolumn{1}{c}{0.00} & 0.00 & 0.00 
& \multicolumn{1}{c}{0.00} & 0.00 & 0.00  
& \multicolumn{1}{c}{0.00} & 0.00 & 0.00  
& \multicolumn{1}{c}{0.00} & 0.00 & 0.00
& \multicolumn{1}{c}{0.00} & 0.00 & 0.00  
\\ 
%   & Spectral~\cite{tran2018spectral}  
% & \multicolumn{1}{c}{0.00} & 0.15 & 0.00 
% & \multicolumn{1}{c}{0.00} & 0.15 & 0.00 
% & \multicolumn{1}{c}{0.12} & 0.15 & 0.00  
% & \multicolumn{1}{c}{0.00} & 0.15 & 0.00  
% & \multicolumn{1}{c}{0.00} & 0.15 & 0.00
%   & Spectral~\cite{tran2018spectral}  
% & \multicolumn{1}{c}{0.00} & 15.00 & 0.00 
% & \multicolumn{1}{c}{0.00} & 15.00 & 0.00 
% & \multicolumn{1}{c}{12.00} & 15.01 & 0.08  
% & \multicolumn{1}{c}{0.00} & 15.02 & 0.00  
% & \multicolumn{1}{c}{0.00} & 15.16 & 0.00
% \\ 
  & STRIP~\cite{gao2019strip}    
& \multicolumn{1}{c}{50.00} & 8.00 & 0.05 
& \multicolumn{1}{c}{20.00} & 8.15 & 0.05 
& \multicolumn{1}{c}{44.00} & 8.29 & 0.51  
& \multicolumn{1}{c}{56.00} & 10.29 & 1.04  
& \multicolumn{1}{c}{93.80} & 12.25 & 12.88
\\
\hline
% \multirow{4}{*}{CIFAR-100}  &AC~\cite{chen2018detecting}     
% & \multicolumn{1}{c}{0.00} & 0.04 & 0.00
% & \multicolumn{1}{c}{0.00} & 0.03 & 0.00
% & \multicolumn{1}{c}{0.00} & 0.01 & 0.00
% & \multicolumn{1}{c}{0.00} & 0.03 & 0.00
% & \multicolumn{1}{c}{0.00} & 0.02 & 0.00
% \\ 
%   &SCAn~\cite{tang2021demon} 
% & \multicolumn{1}{c}{0.00} & 0.00 & 0.00 
% & \multicolumn{1}{c}{0.00} & 0.00 & 0.00  
% & \multicolumn{1}{c}{0.00} & 0.00 & 0.00  
% & \multicolumn{1}{c}{0.00} & 0.00 & 0.00
% & \multicolumn{1}{c}{0.00} & 0.00 & 0.00  
% \\ 
%   &Spectral~\cite{tran2018spectral}  
% & \multicolumn{1}{c}{1.00} & 0.15 & 0.00 
% & \multicolumn{1}{c}{1.00} & 0.15 & 0.00 
% & \multicolumn{1}{c}{0.00} & 0.15 & 0.00  
% & \multicolumn{1}{c}{1.00} & 0.15 & 0.01  
% & \multicolumn{1}{c}{0.00} & 0.15 & 0.00
% \\ 
%   &STRIP~\cite{gao2019strip}    
% & \multicolumn{1}{c}{0.00} & 0.12 & 0.00 
% & \multicolumn{1}{c}{0.00} & 0.13 & 0.00 
% & \multicolumn{1}{c}{0.48} & 0.13 & 0.00  
% & \multicolumn{1}{c}{0.78} & 0.13 & 0.01  
% & \multicolumn{1}{c}{1.00} & 0.13 & 0.14
\multirow{4}{*}{CIFAR-100}  &AC~\cite{chen2018detecting}     
& \multicolumn{1}{c}{0.00} & 0.97 & 0.00
& \multicolumn{1}{c}{0.00} & 0.28 & 0.00
& \multicolumn{1}{c}{0.00} & 0.48 & 0.00
& \multicolumn{1}{c}{0.00} & 0.92 & 0.00
& \multicolumn{1}{c}{0.00} & 0.93 & 0.00
\\ 
  &SCAn~\cite{tang2021demon} 
& \multicolumn{1}{c}{0.00} & 0.00 & 0.00 
& \multicolumn{1}{c}{0.00} & 0.00 & 0.00  
& \multicolumn{1}{c}{0.00} & 0.00 & 0.00  
& \multicolumn{1}{c}{0.00} & 0.00 & 0.00
& \multicolumn{1}{c}{0.00} & 0.00 & 0.00  
% \\ 
%   &Spectral~\cite{tran2018spectral}  
% & \multicolumn{1}{c}{100.00} & 30.00 & 0.03 
% & \multicolumn{1}{c}{100.00} & 30.00 & 0.07 
% & \multicolumn{1}{c}{0.00} & 15.02 & 0.00  
% & \multicolumn{1}{c}{100.00} & 30.00 & 0.66 
% & \multicolumn{1}{c}{0.00} & 15.22 & 0.00
\\ 
  &STRIP~\cite{gao2019strip}    
& \multicolumn{1}{c}{0.00} & 14.66 & 0.00 
& \multicolumn{1}{c}{0.00} & 12.56 & 0.00 
& \multicolumn{1}{c}{48.00} & 13.06 & 0.36  
& \multicolumn{1}{c}{76.00} & 12.47 & 1.19  
& \multicolumn{1}{c}{100.00} & 8.31 & 19.56
\\
\hline
% \multirow{4}{*}{Tiny ImageNet}  &AC~\cite{chen2018detecting}     
% & \multicolumn{1}{c}{0.00} & 0.01 & 0.00
% & \multicolumn{1}{c}{0.00} & 0.01 & 0.00
% & \multicolumn{1}{c}{0.00} & 0.01 & 0.00
% & \multicolumn{1}{c}{0.00} & 0.01 & 0.00
% & \multicolumn{1}{c}{0.00} & 0.02 & 0.00
% \\ 
%   &SCAn~\cite{tang2021demon} 
% & \multicolumn{1}{c}{0.00} & 0.00 & 0.00 
% & \multicolumn{1}{c}{0.00} & 0.00 & 0.00  
% & \multicolumn{1}{c}{0.00} & 0.00 & 0.00  
% & \multicolumn{1}{c}{0.99} & 0.00 & 0.96
% & \multicolumn{1}{c}{0.99} & 0.00 & 1.00  
% \\ 
%   &Spectral~\cite{tran2018spectral}  
% & \multicolumn{1}{c}{0.00} & 0.15 & 0.00 
% & \multicolumn{1}{c}{0.70} & 0.00 & 0.14 
% & \multicolumn{1}{c}{0.40} & 0.15 & 0.00  
% & \multicolumn{1}{c}{0.80} & 0.15 & 0.01  
% & \multicolumn{1}{c}{0.00} & 0.15 & 0.00
% \\ 
%   &STRIP~\cite{gao2019strip}    
% & \multicolumn{1}{c}{0.25} & 0.16 & 0.00 
% & \multicolumn{1}{c}{0.40} & 0.13 & 0.00 
% & \multicolumn{1}{c}{0.62} & 0.16 & 0.00  
% & \multicolumn{1}{c}{0.78} & 0.16 & 0.01  
% & \multicolumn{1}{c}{0.96} & 0.18 & 0.10
\multirow{4}{*}{Tiny ImageNet}  &AC~\cite{chen2018detecting}     
& \multicolumn{1}{c}{0.00} & 1.07 & 0.00
& \multicolumn{1}{c}{0.00} & 0.68 & 0.00
& \multicolumn{1}{c}{0.00} & 0.58 & 0.00
& \multicolumn{1}{c}{0.00} & 0.67 & 0.00
& \multicolumn{1}{c}{0.00} & 1.60 & 0.00
\\ 
  &SCAn~\cite{tang2021demon} 
& \multicolumn{1}{c}{0.00} & 0.00 & 0.00 
& \multicolumn{1}{c}{0.00} & 0.00 & 0.00  
& \multicolumn{1}{c}{0.00} & 0.00 & 0.00  
& \multicolumn{1}{c}{0.00} & 0.00 & 0.00  
% & \multicolumn{1}{c}{99.00} & 0.00 & 95.65
& \multicolumn{1}{c}{99.90} & 0.00 & 99.50  
% \\ 
%   &Spectral~\cite{tran2018spectral}  
% & \multicolumn{1}{c}{0.00} & 15.00 & 0.00 
% & \multicolumn{1}{c}{90.00} & 14.99 & 0.12 
% & \multicolumn{1}{c}{40.00} & 15.00 & 0.26  
% & \multicolumn{1}{c}{80.00} & 14.95 & 1.05  
% & \multicolumn{1}{c}{0.00} & 15.22 & 0.00
\\ 
  &STRIP~\cite{gao2019strip}    
& \multicolumn{1}{c}{25.00} & 15.67 & 0.01 
& \multicolumn{1}{c}{40.00} & 13.03 & 0.06 
& \multicolumn{1}{c}{62.00} & 16.16 & 0.38  
& \multicolumn{1}{c}{78.00} & 15.91 & 0.96  
& \multicolumn{1}{c}{95.70} & 18.41 & 9.32
\\
\bottomrule
\end{tabular}
}}
\end{table*}

\begin{figure}[htbp]
\centering
\includegraphics[width=8.85cm,height=2.9cm]{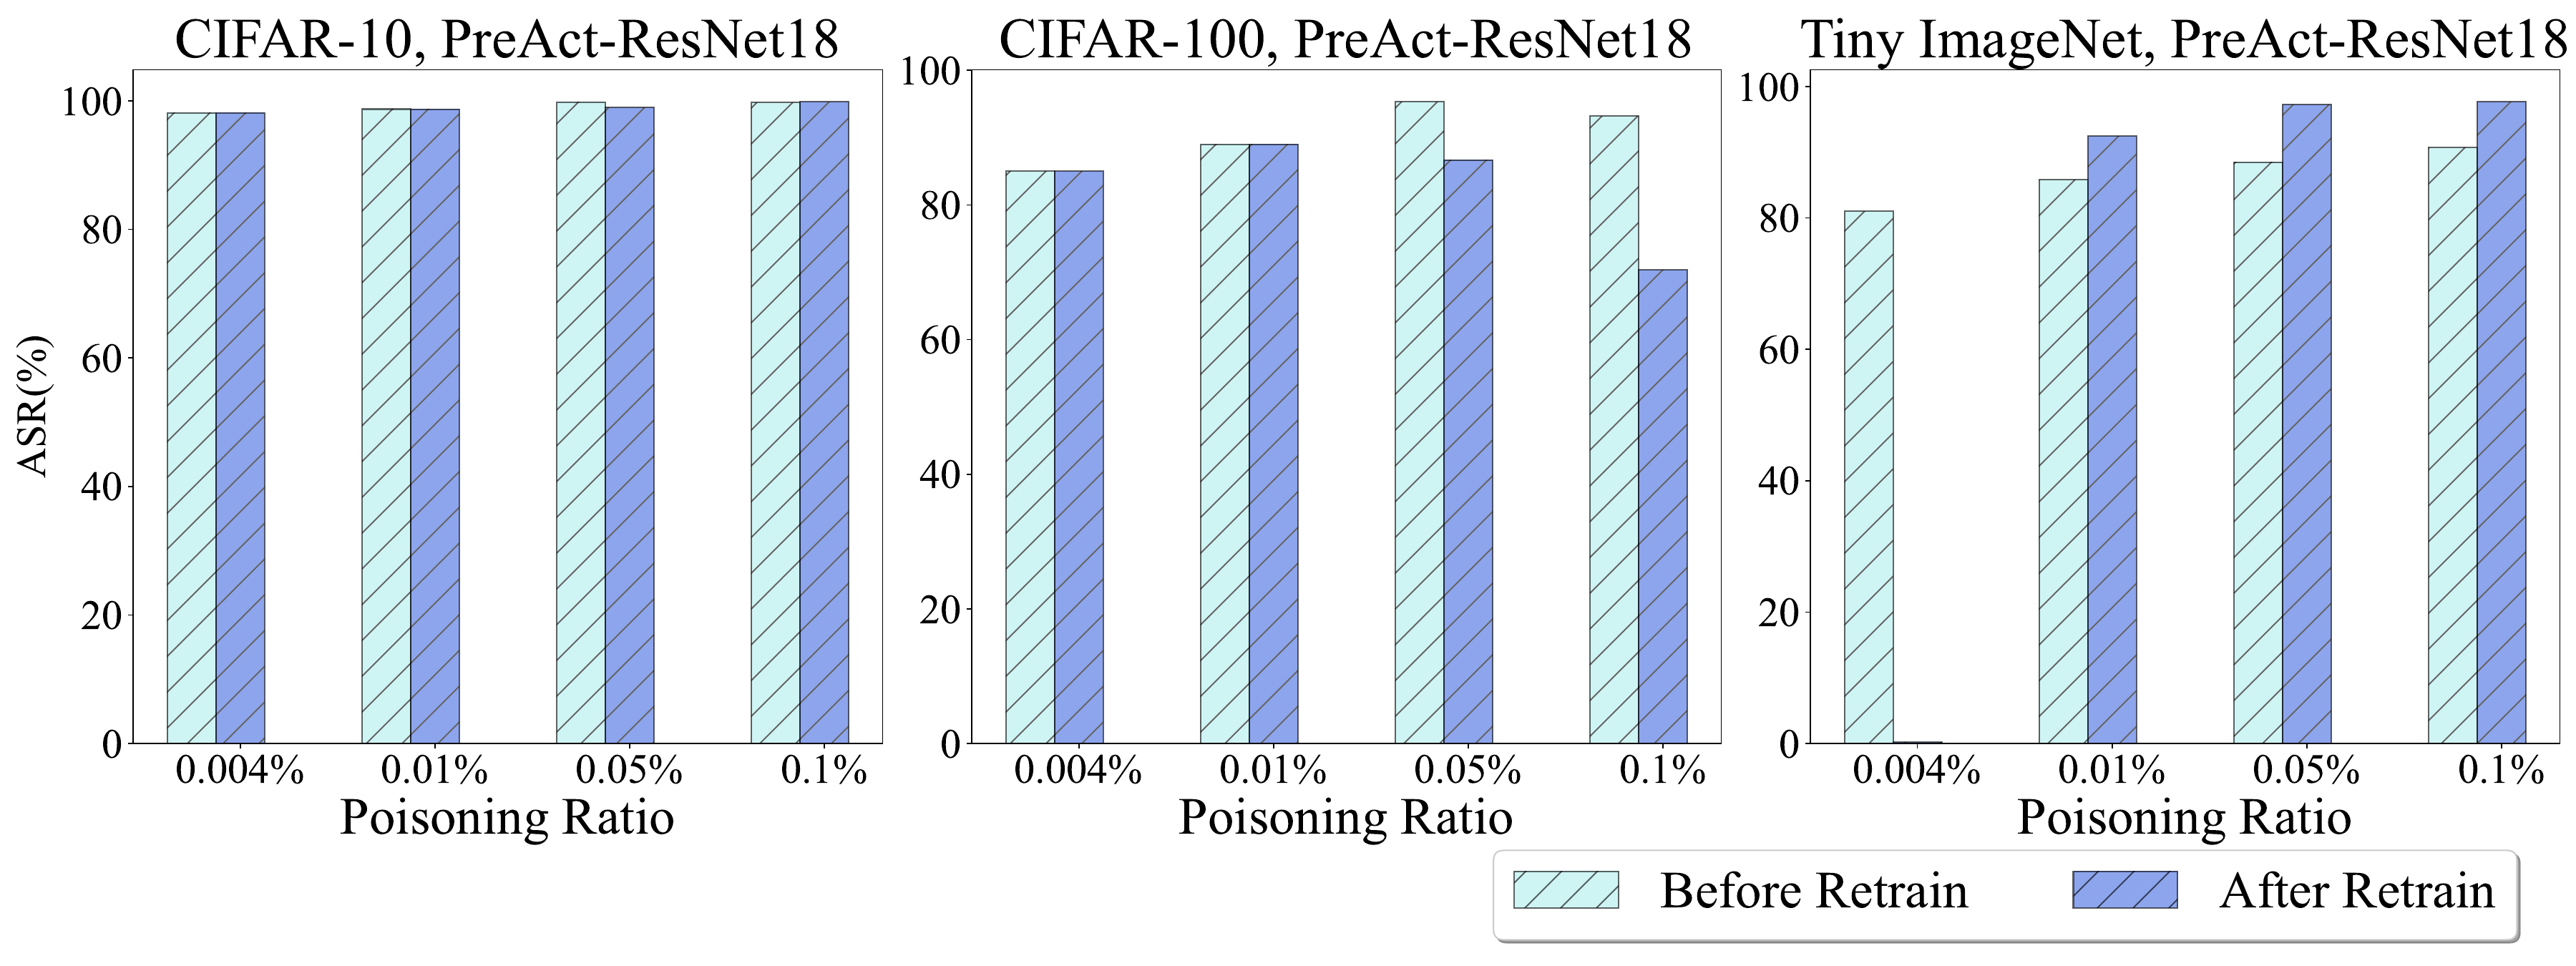}
\caption{Results of STRIP retraining after removing suspicious samples on PreAct-ResNet18.}
\label{STRIP detection pre}
\vspace{-0.5cm}
\end{figure}

\begin{figure}[!ht]
\centering  %图片全局居中
% \vspace{-5.2cm}
    \subfigure[CIFAR-10]{
    \includegraphics[width=3.45in]
    {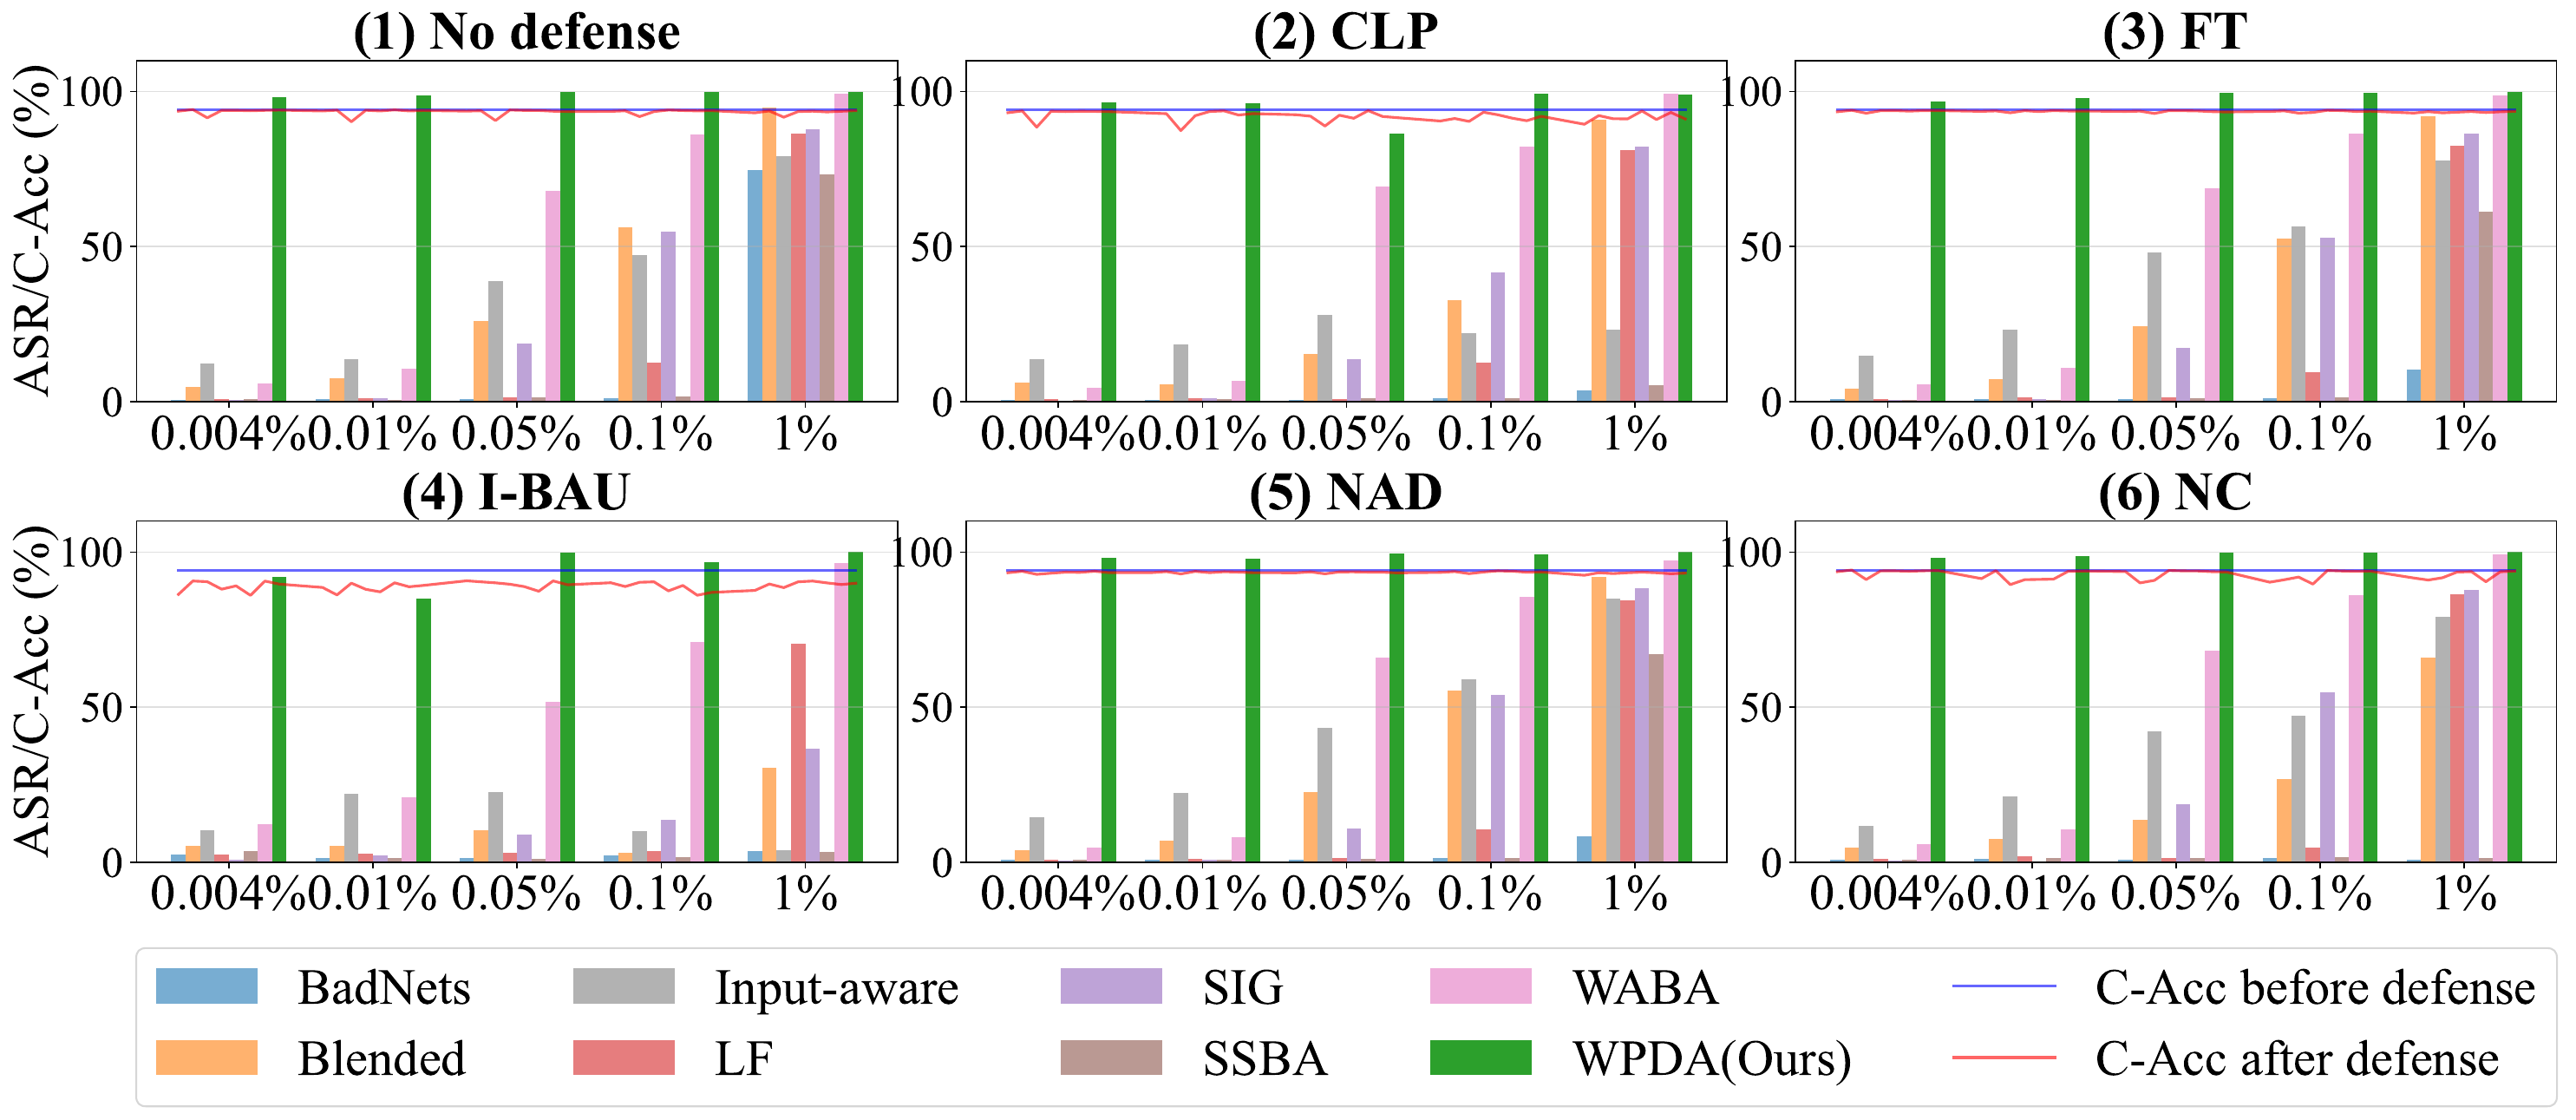}
    % {figures/cifar10_preactresnet18_1.pdf}
    }
    \label{CIFAR-10_pre_defense}
    \subfigure[CIFAR-100]{
    \includegraphics[width=3.45in]
    {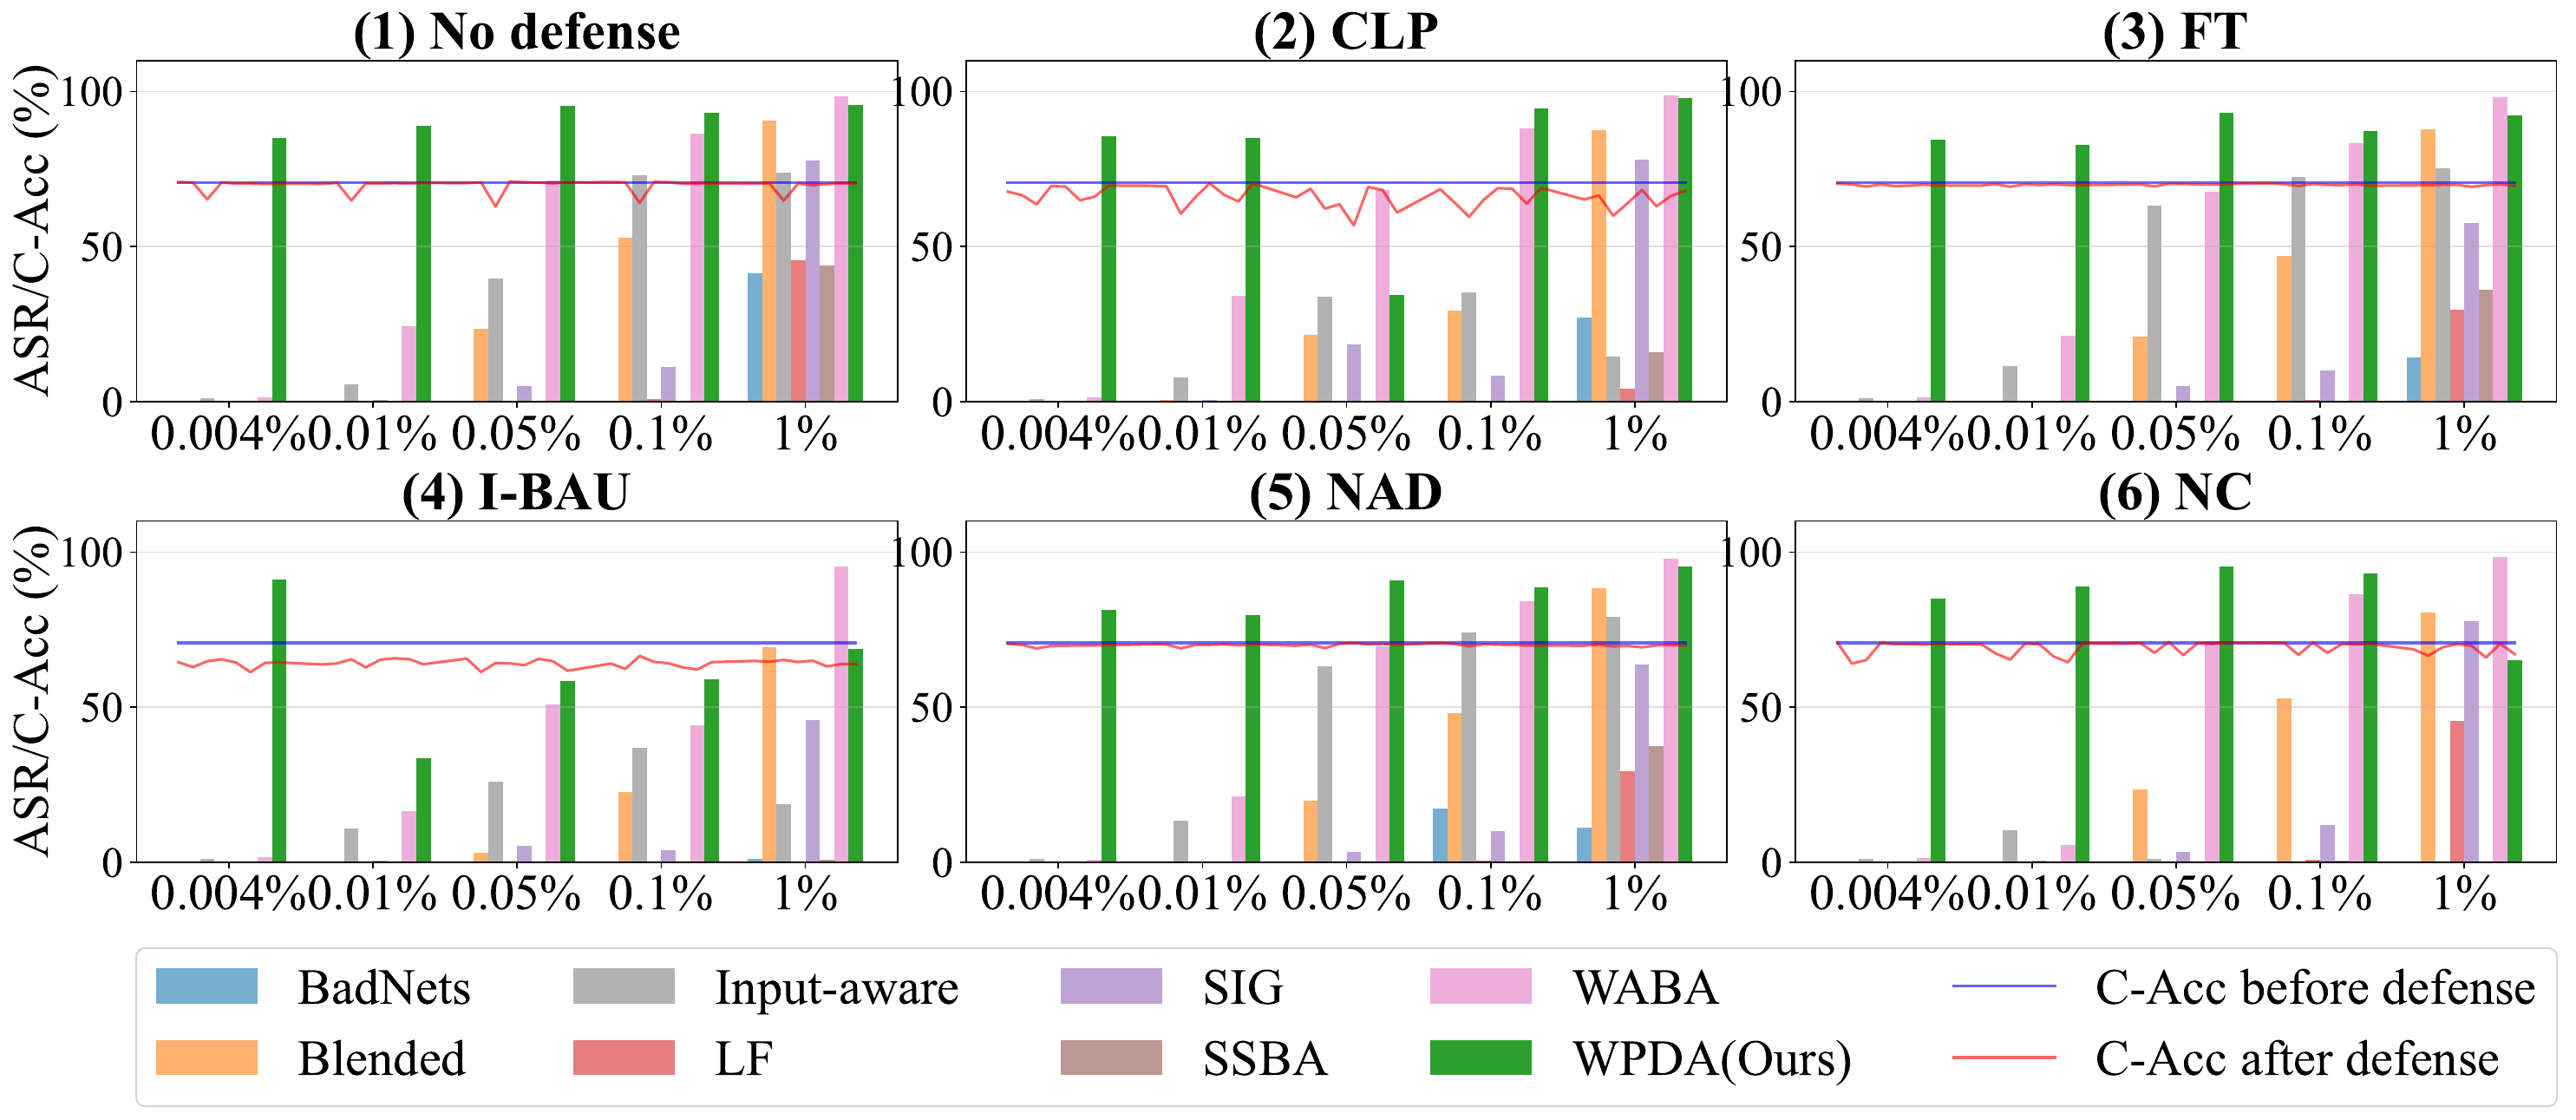}
    % {figures/cifar100_preactresnet18_2.pdf}
    }
    \label{CIFAR-100_pre_defense}
    \subfigure[Tiny ImageNet]{
    \includegraphics[width=3.45in]
    {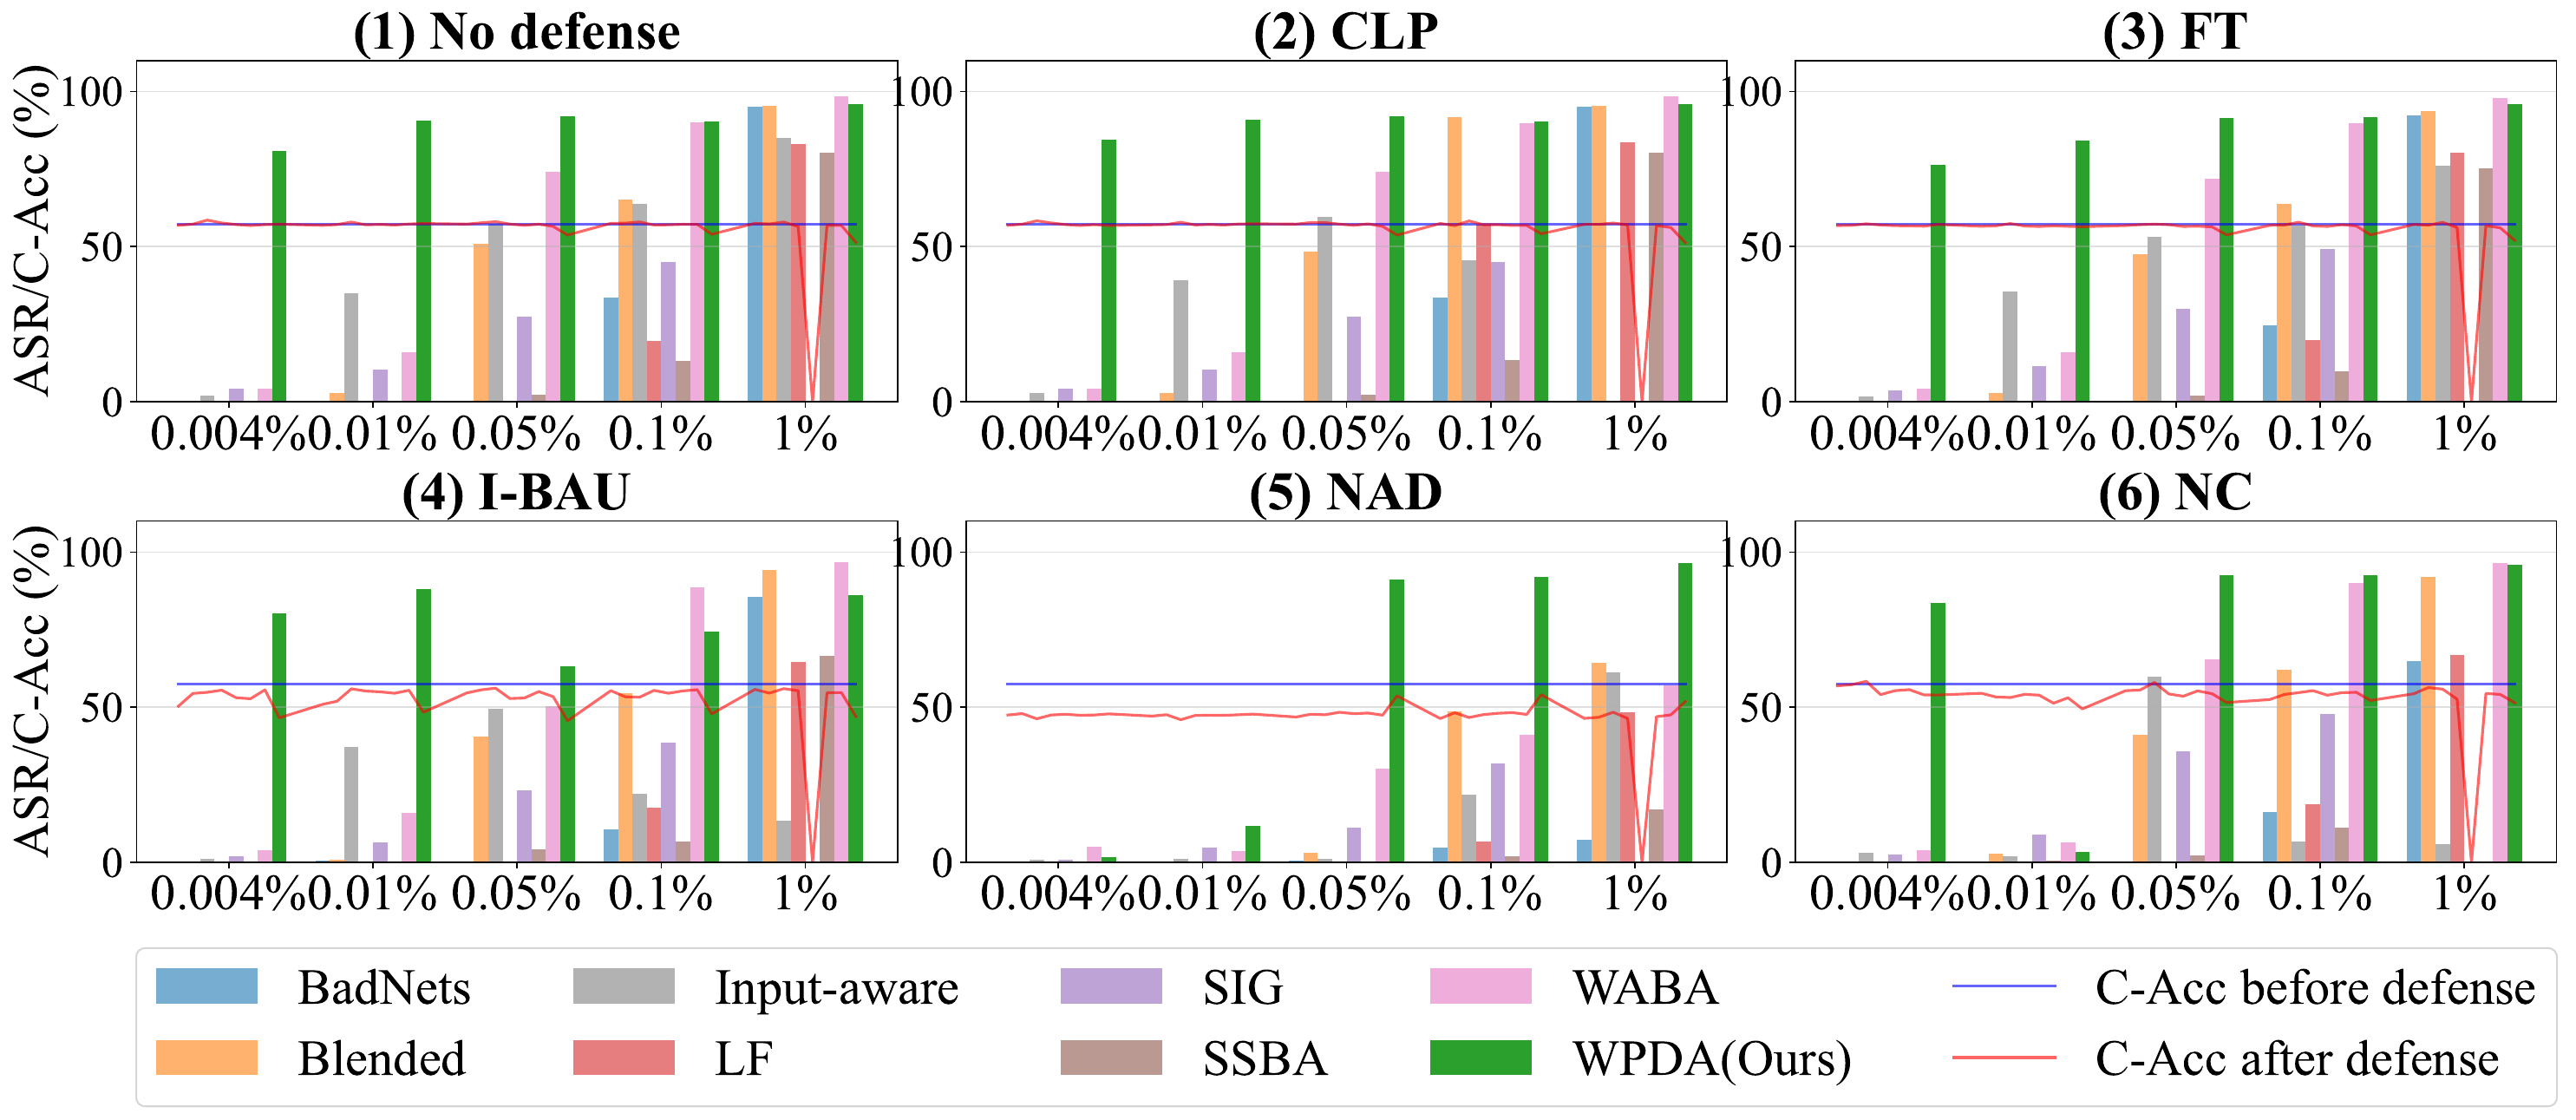}
    % {figures/tiny_preactresnet18_2.pdf}
    }
    \label{tiny_pre_defense}
\caption{Results of 7 compared attack methods and WPDA against 5 defense methods on PreAct-ResNet18, including CLP, FT, I-BAU, NAD and NC. Each sub-plot corresponds to one defense method. In each sub-plot, each bar in the histogram indicates the ASR value of one attack method, and the C-Acc values are represented by curves.}
\vspace{-0.5cm}
\label{all-defense-pre}
\end{figure}
\subsection{\textbf{Defense Performance of WPDA on PreAct-ResNet18}:
\label{defense on pre}}
Fig.~\ref{all-defense-pre} illustrates the attack performance of WPDA and other attacks under 5 SOTA backdoor defense methods on PreAct-ResNet18. 
\textbf{On CIFAR-10}, WPDA demonstrates resistant, efficient, and stealthy performance after undergoing various defense methods. Maintaining a consistently high ASR across all poisoning ratios, it demonstrably outperforms other attack methods. 
\textbf{On CIFAR-100}, most methods with lower poisoning ratios exhibit more resistant performance after defense compared to those with higher poisoning ratios. For instance, after CLP, the ASR degradation observed in Blended and Input-aware methods is demonstrably more pronounced at a poisoning ratio of 0.1\% relative to 0.05\%. Similarly, the decrease in ASR for WPDA at 0.05\% poisoning ratio is higher than that at 0.01\% poisoning ratio. This phenomenon is also evident after I-BAU. 
\textbf{On Tiny ImageNet}, after CLP and FT, WPDA continues to outperform all compared attack methods across all poisoning ratios. After I-BAU, although there is a certain degree of decline in WPDA's ASR, it still remains effective, particularly the WPDA at low poisoning ratios, exhibiting more resistant performance to defense compared to high poisoning ratios. After NAD, the effectiveness of all attack methods at poisoning ratios of 0.004\% and 0.01\% is significantly impacted. However, our ASR still exhibits residual activity at 0.01\% poisoning ratio. Furthermore, the accuracy of the model at 0.004\% and 0.01\% poisoning ratios on benign samples has decreased substantially after NAD, even dropping below 50\%, which means the performance of the model on benign samples is compromised, and attacks still works. After NC, WPDA demonstrates more resistant and efficient performance than other attack methods at poisoning ratios of 0.004\%, 0.05\%, and 0.1\%. At 0.1\% poisoning ratio, there is a significant decrease in ASR for all attack methods, but only WPDA compromises the performance of the model on benign samples successfully. For WPDA, after undergoing NAD, the accuracy of the model on benign samples drops to around 50\%, greatly impacting the model's performance.  
\textbf{In summary}, our method demonstrates more resistant, stealthy, and effective performance than other compared attack methods after undergoing various defense methods. Additionally, it is evident that the effectiveness of most defense methods significantly decreases when faced with attacks at low poisoning ratios. Therefore, it is crucial to develop defense methods for low  poisoning ratios.
